# Supplementary material for: The Randomized BH Procedure: A Generalized Framework Encompassing Conformal and Competition Tests
Source: arXiv:2607.07245 source file (2026-10-26)
Supplement: Supplementary file 1 [file Re_supp.tex]

\documentclass{article}
\usepackage{arxiv}
\usepackage{amsmath,amssymb}
\usepackage{amsthm}

\usepackage{graphicx}
\graphicspath{ {./images/} }
\usepackage{float}
\usepackage[ruled,vlined]{algorithm2e}
\usepackage[titles]{tocloft}

\usepackage{xr-hyper}
\usepackage{hyperref}       % hyperlinks
% cleveref removed; use \ref instead

\externaldocument{Re_main}
\usepackage{booktabs}       % professional-quality tables
\usepackage{amsfonts}       % blackboard math symbols
\usepackage{nicefrac}       % compact symbols for 1/2, etc.
\usepackage{microtype}      % microtypography
\usepackage{siunitx}
\usepackage{appendix}
\usepackage{chngcntr}  % change counter for appendix
\usepackage{caption}   % caption for appendix

\setcounter{page}{1}
\newtheorem{Thm}{Theorem}
\newtheorem{Lemma}{Lemma}

\theoremstyle{definition}

\pagestyle{fancy}

\usepackage{geometry}
\usepackage[pagewise]{lineno}
\usepackage{setspace}
\setstretch{2}
\allowdisplaybreaks

\title{Supplementary Materials}

% \title{Supplementary Materials for ``The Randomized BH Procedure: A Generalized Framework Encompassing Conformal and Competition Tests''}

% \author{
%   Mingzhou Deng \\
%   State Key Laboratory of Mathematical Science, Academy of Mathematics and Systems Science\\ Chinese Academy of Sciences\\
%   \texttt{dengminzghou@amss.ac.cn} \\
%    \And
%   Yan Fu \\
%   State Key Laboratory of Mathematical Science, Academy of Mathematics and Systems Science\\ Chinese Academy of Sciences\\
%   \texttt{yfu@amss.ac.cn} \\
% }

\begin{document}
\raggedbottom

\maketitle

\setcounter{section}{0}
\setcounter{equation}{0}
\def\theequation{S\arabic{section}.\arabic{equation}}
\def\thesection{S\arabic{section}}

\tableofcontents

\section{Proofs for FDR Control for BH and Conformal BH Procedures}
\label{app:bh}

To prove Theorem~\ref{thm:fdr_cbh}, it suffices to establish Theorem~\ref{thm:fdr_bh} and to verify that conformal p-values are BH-valid. We provide the proofs of both results below.

\begin{proof}[Proof of Theorem~\ref{thm:fdr_bh}]
By definition, we have $K=|\mathcal{R}_{\alpha}(\mathbf{X})|$,
\begin{align*}
    \mathrm{FDR}&=\mathbb{E}\frac{\sum_{j\in\mathcal{H}_0}\mathbf{1}\{X_j\leq q_K^{m,\alpha}\}}{1\vee\sum_{i\in\mathcal{H}}\mathbf{1}\{X_i\leq q_K^{m,\alpha}\}}=\sum_{j\in\mathcal{H}_0}\mathbb{E}\frac{\mathbf{1}\{X_j\leq q_K^{m,\alpha}\}}{1\vee K}\\
    &=\sum_{j\in\mathcal{H}_0}\mathbb{E}\sum_{k=1}^m\frac{\mathbf{1}\{X_j\leq q_k^{m,\alpha}\}}{k}\mathbf{1}\{K=k\}\\
    &=\sum_{j\in\mathcal{H}_0}\sum_{k=1}^m\frac{1}{k}\mathbb{P}\left\{X_j\leq q_k^{m,\alpha},|\mathcal{R}_{\alpha}(\mathbf{X})|=k\right\}\\
    &\leq\sum_{j\in\mathcal{H}_0}\sum_{k=1}^m\frac{\alpha}{m}\mathbb{P}\left\{|\mathcal{R}_{\alpha}(\mathbf{X})|=k\big| X_j\leq q_k^{m,\alpha}\right\}
\end{align*}
The inequality in the last line holds because $\mathbf{X}$ are p-variables. Note that for any $\boldsymbol{x}' \geq \boldsymbol{x}$ and $k > |\mathcal{R}_{\alpha}(\boldsymbol{x})|$, we have $x'_{(k)} \geq x_{(k)} > q_k^{m,\alpha}$. Therefore, the set $\{\boldsymbol{x} : |\mathcal{R}_{\alpha}(\boldsymbol{x})| \leq k\}$ is nondecreasing. Since $\mathbf{X}$ are $\mathrm{PRDS}_{\mathcal{H}_0}$, it follows that for any $j \in \mathcal{H}_0$,
\[
\mathbb{P} \left\{ |\mathcal{R}_{\alpha}(\mathbf{X})| \leq k-1 \mid X_j \leq q_{k-1}^{m,\alpha} \right\} \leq \mathbb{P} \left\{ |\mathcal{R}_{\alpha}(\mathbf{X})| \leq k-1 \mid X_j \leq q_{k}^{m,\alpha} \right\},
\]
and then
\begin{align*}
    &\mathrm{FDR}\leq\sum_{j\in\mathcal{H}_0}\sum_{k=1}^m\frac{\alpha}{m}\mathbb{P}\left\{|\mathcal{R}_{\alpha}(\mathbf{X})|=k\big| X_j\leq q_k^{m,\alpha}\right\}\\
    &\leq\frac{\alpha}{m}\sum_{j\in\mathcal{H}_0}\sum_{k=1}^m\left(\mathbb{P}\left\{|\mathcal{R}_{\alpha}(\mathbf{X})|\leq k\big| X_j\leq q_k^{m,\alpha}\right\}-\mathbb{P}\left\{|\mathcal{R}_{\alpha}(\mathbf{X})|\leq k-1\big| X_j\leq q_{k-1}^{m,\alpha}\right\}\right)\\
    &\leq\frac{\alpha}{m}\sum_{j\in\mathcal{H}_0}\mathbb{P}\left\{|\mathcal{R}_{\alpha}(\mathbf{X})|\leq m\big| X_j\leq q_m^{m,\alpha}\right\}\leq\alpha\frac{m_0}{m}.
\end{align*}
\end{proof}

\begin{proof}[Proof of Theorem~\ref{thm:fdr_ebh}]
By definition, we have $K=|\mathcal{R}_{\alpha}(\mathbf{X})|$. Note that when $K\leq m$, the identity $f^{m,\alpha}_K=m/[(m-K+1)\alpha]$ gives $\alpha f^{m,\alpha}_K/m=1/(m-K+1)=1/(1\vee(m-K+1))$. When $K=m+1$, both $1/(1\vee(m-K+1))$ and $\alpha f^{m,\alpha}_{K\wedge m}/m$ equal $1$. Hence
\begin{align*}
    \mathrm{FDR}&=\mathbb{E}\frac{\sum_{j\in\mathcal{H}_0}\mathbf{1}\{X_j\geq f_K^{m,\alpha}\}}{1\vee\sum_{i\in\mathcal{H}}\mathbf{1}\{X_i\geq f_K^{m,\alpha}\}}=\sum_{j\in\mathcal{H}_0}\mathbb{E}\frac{\mathbf{1}\{X_j\geq f_K^{m,\alpha}\}}{1\vee (m-K+1)}\\
    &=\sum_{j\in\mathcal{H}_0}\mathbb{E}\frac{\alpha f^{m,\alpha}_{K\wedge m}}{m}\mathbf{1}\{X_j\geq f_K^{m,\alpha}\}\\
    &\leq\frac{\alpha}{m}\sum_{j\in\mathcal{H}_0}\mathbb{E}X_j\mathbf{1}\{X_j\geq f_K^{m,\alpha}\}\leq\frac{\alpha}{m}\sum_{j\in\mathcal{H}_0}\mathbb{E}X_j
\end{align*}
Because $\mathbf{X}$ are compound e-variables,
\[
\mathrm{FDR}\leq\frac{\alpha}{m}\sum_{j\in\mathcal{H}_0}\mathbb{E}X_j\leq\alpha.
\]
\end{proof}

\begin{proof}[Proof of Theorem~\ref{thm:fdr_cbh}]
We need to verify two conditions. First, under exchangeability, let $\mathbf{Z}_{\cup j}=(X_j,\mathbf{Y})$ and $\mathbf{Z}_{\cup j,(\cdot)}$ be its order statistics,
\[
\mathbb{P}\left\{P_j\leq t\right\}=\mathbb{E}\left[\mathbb{P}\left\{P_j\leq t\mid \mathbf{Z}_{\cup j,(\cdot)},\mathbf{X}_{-j}\right\}\right]=\frac{\lceil t(1+n)\rceil}{1+n}\leq t.
\]
Furthermore, we have for any $k\in[n+1]$,
\[
\mathbb{P}\left\{P_j=\frac{k}{1+n}\right\}=\mathbb{E}\left[\mathbb{P}\left\{P_j=\frac{k}{1+n}\mid \mathbf{Z}_{\cup j,(\cdot)},\mathbf{X}_{-j}\right\}\right]=\frac{1}{1+n}.
\]

Second, we have for any nondecreasing set $C\in\mathbb{R}^m$ and any $k\in[n+1]$,
\begin{align*}
    &\mathbb{P}\left\{\mathbf{P}_{-j}\in C\mid P_j=\frac{k}{1+n}\right\}\\
    =&\mathbb{E}_{\mathbf{Z}_{\cup j,(\cdot)},\mathbf{X}_{-j}}\left[\mathbb{P}\left\{\mathbf{P}_{-j}\in C\mid P_j=\frac{k}{1+n},\mathbf{Z}_{\cup j,(\cdot)},\mathbf{X}_{-j}\right\}\Big|P_j=\frac{k}{1+n}\right]
\end{align*}
where
\[
\mathbb{P}\left\{\mathbf{Z}_{\cup j,(\cdot)},\mathbf{X}_{-j}\mid P_j=\frac{k}{1+n}\right\}=\frac{\mathbb{P}\left(\mathbf{Z}_{\cup j,(\cdot)},\mathbf{X}_{-j}\right)\mathbb{P}\left\{P_j=\frac{k}{1+n}\mid \mathbf{Z}_{\cup j,(\cdot)},\mathbf{X}_{-j}\right\}}{\mathbb{P}\left\{P_j=\frac{k}{1+n}\right\}}=\mathbb{P}\left(\mathbf{Z}_{\cup j,(\cdot)},\mathbf{X}_{-j}\right).
\]
For any vectors $\boldsymbol{x}^j\in\mathbb{R}^{m-1},\boldsymbol{z}^j\in\mathbb{R}^{n}$ and $\boldsymbol{x}\in\mathbb{R}^m,\boldsymbol{y}\in\mathbb{R}^n$ satisfying $\boldsymbol{x}_{-j}=\boldsymbol{x}^j,\boldsymbol{y}_{(\cdot)}=\boldsymbol{z}^j$, we define a function $f_j(\boldsymbol{x}^j,\boldsymbol{z}^j)=\mathbf{1}\{\mathbf{P}_{-j}(\boldsymbol{x},\boldsymbol{y})\in C\}$. This function is well-defined by the construction of the conformal p-values. The function $f_j$ is monotone non-increasing with respect to $\boldsymbol{z}^j$, and hence for any $w\leq k$,
\[
\mathbb{P}\left\{\mathbf{P}_{-j}\in C\mid P_j=\frac{w}{1+n},\mathbf{Z}_{\cup j,(\cdot)},\mathbf{X}_{-j}\right\}\leq\mathbb{P}\left\{\mathbf{P}_{-j}\in C\mid P_j=\frac{k}{1+n},\mathbf{Z}_{\cup j,(\cdot)},\mathbf{X}_{-j}\right\}.
\]
Taking expectations with respect to the conditional distribution derived above shows that
\[
\mathbb{P}\left\{\mathbf{P}_{-j}\in C\mid P_j=\frac{k}{1+n}\right\}
\]
is nondecreasing with respect to $k$. For any $w\leq k$,
\begin{align*}
    \mathbb{P}\left\{\mathbf{P}_{-j}\in C\mid P_j\leq\frac{k}{1+n}\right\}&=\frac{\sum_{v=1}^k\mathbb{P}\left\{\mathbf{P}_{-j}\in C\mid P_j=\frac{v}{1+n}\right\}\mathbb{P}\left\{P_j=\frac{v}{1+n}\right\}}{\mathbb{P}\left\{P_j\leq\frac{k}{1+n}\right\}}\\
    &=\frac{1}{k}\sum_{v=1}^k\mathbb{P}\left\{\mathbf{P}_{-j}\in C\mid P_j=\frac{v}{1+n}\right\}\\
    &\geq \frac{1}{w}\sum_{v=1}^w\mathbb{P}\left\{\mathbf{P}_{-j}\in C\mid P_j=\frac{v}{1+n}\right\}\\
    &=\mathbb{P}\left\{\mathbf{P}_{-j}\in C\mid P_j\leq\frac{w}{1+n}\right\}
\end{align*}
In summary, the conformal p-values $\mathbf{P}(\mathbf{X},\mathbf{Y})$ are $\mathrm{PRDS}_{\mathcal{H}_0}$.
\end{proof}

\section{Proofs for FDR Control for the Competition Procedure}
\label{app:cp}

We introduce three proof methods: 'with martingale', 'with combination', and 'with flip-one'. We will discuss their respective advantages in the following section. In particular, the first two proofs are based on competition statistics, which implies that the label probabilities must be identical fixed values. In contrast, the last proof requires only the sub-competition statistics given in the article to achieve FDR control.

We begin by presenting the following derivation. Regardless of whether $(\mathbf{W},\mathbf{L})$ are sub-competition statistics, with the definition of $T$, we always have the following inequality.
\begin{align*}
    \mathrm{FDR}&=\mathbb{E}\left[\frac{\sum_{j\in\mathcal{H}_0}\mathbf{1}\left\{W_j\geq T,L_j=1\right\}}{\left(\sum_{j\in\mathcal{H}}\mathbf{1}\left\{W_j\geq T,L_j=1\right\}\right)\vee1}\right]\\
    &=\mathbb{E}\left[\frac{r\sum_{j\in\mathcal{H}_0}\mathbf{1}\left\{W_j\geq T,L_j=0\right\}+r}{\left(\sum_{j\in\mathcal{H}}\mathbf{1}\left\{W_j\geq T,L_j=1\right\}\right)\vee1}\cdot\frac{\sum_{j\in\mathcal{H}_0}\mathbf{1}\left\{W_j\geq T,L_j=1\right\}}{r\sum_{j\in\mathcal{H}}\mathbf{1}\left\{W_j\geq T,L_j=0\right\}+r}\right]\\
    &\leq\alpha\mathbb{E}\left[\frac{\sum_{j\in\mathcal{H}_0}\mathbf{1}\left\{W_j\geq T,L_j=1\right\}}{r\sum_{j\in\mathcal{H}}\mathbf{1}\left\{W_j\geq T,L_j=0\right\}+r}\right]
\end{align*}

Thus, we obtain the following sufficient condition to control the FDR.

\[
\mathbb{E}\left[\frac{\sum_{j\in\mathcal{H}_0}\mathbf{1}\left\{W_j\geq T,L_j=1\right\}}{r\sum_{j\in\mathcal{H}}\mathbf{1}\left\{W_j\geq T,L_j=0\right\}+r}\right]\leq1\Rightarrow \mathrm{FDR}\leq\alpha.
\]

In the following, we focus exclusively on the proof of this sufficient condition.

\begin{proof}[Proof via martingale]

We consider FDR control under the condition that $(\mathbf{W},\mathbf{L})$ are competition statistics. Let $\mathbf{W}_{(\cdot)}$ be nonincreasing with $W_{(0)}=+\infty$ and $V_+(t)=|\mathcal{R}_+(t)\cap\mathcal{H}_0|$, $V_-(t)=|\mathcal{R}_-(t)\cap\mathcal{H}_0|$. We define
\[
M_t=\frac{V_+(t)}{1+V_-(t)},\widetilde{M}_k=M_{W_{(k)}}
\]

Let $\mathcal{H}_0(t)=\{j\in\mathcal{H}_0:W_j\geq t\}$ and $k_t=\arg\min_{j}\{W_j:j\in\mathcal{H}_0(t)\}$. When $V_+(t)>0$, we have
\begin{align*}
    P\left(L_{k_t}=1\big| V_+(t),V_-(t),\mathcal{H}_0(t)\right)=\frac{V_+(t)}{V_+(t)+V_-(t)}
\end{align*}
and then for any $k$,
\begin{align*}
    &\mathbb{E}\left[\widetilde{M}_{k}-\widetilde{M}_{k+1}\Big|\sigma\{\widetilde{M}_{k}\}\right]=\mathbb{E}\left[\frac{V_+(W_{(k)})}{1+V_-(W_{(k)})}-\frac{V_+(W_{(k+1)})}{1+V_-(W_{(k+1)})}\Big|\sigma\{\widetilde{M}_{k}\}\right]\\
    =&\mathbb{E}\left[\mathbb{E}\left[\frac{V_+(W_{(k)})}{1+V_-(W_{(k)})}-\frac{V_+(W_{(k+1)})}{1+V_-(W_{(k+1)})}\Big|V_+(W_{(k)}),V_-(W_{(k)}),\mathcal{H}_0(W_{(k)})\right]\Big|\sigma\left\{\widetilde{M}_{k}\right\}\right]\leq 0.
\end{align*}
So $\{\widetilde{M}_k\}$ is a reverse supermartingale, and with Doob's theorem, we have
\begin{align*}
    &\mathbb{E}\left[\frac{\sum_{j\in\mathcal{H}_0}\mathbf{1}\left\{W_j\geq T,L_j=1\right\}}{r\sum_{j\in\mathcal{H}}\mathbf{1}\left\{W_j\geq T,L_j=0\right\}+r}\right]\leq\mathbb{E}\left[\frac{\sum_{j\in\mathcal{H}_0}\mathbf{1}\left\{W_j\geq 0,L_j=1\right\}}{r\sum_{j\in\mathcal{H}_0}\mathbf{1}\left\{W_j\geq 0,L_j=0\right\}+r}\right]\\
    =&\sum_{k=0}^{|\mathcal{H}_0|}\frac{1}{r}\frac{k}{1+|\mathcal{H}_0|-k}\binom{|\mathcal{H}_0|}{k}\left(\frac{r}{1+r}\right)^{k}\left(\frac{1}{1+r}\right)^{|\mathcal{H}_0|-k}<1
\end{align*}
\end{proof}

\begin{proof}[Proof via combination]

We consider FDR control under the condition that $(\mathbf{W},\mathbf{L})$ are competition statistics. Construct a variable which can control the target in the sense of expectation,
\[
\delta(t)=\max_{u\geq t}\left\{V_+(u):V_-(u)=0\right\}.
\]

It is evident that $\delta(0)\geq\delta(T)$, and furthermore we have the following lemma.

\begin{Lemma}
\label{slem:overvariable}
$\delta(T)$ follows a conditional distribution,
\[
\mathbb{P}\left(\delta(T)=k\Big|V_+(T),V_-(T)\right)=f\left(k;V_+(T),V_-(T)\right)
\]
which is independent of the value of $T_i$ with condition that $V_+(T),V_-(T)$ are given. Then, there is a conditional expectation
\[
\mathbb{E}\left[\delta(T)\big|V_+(T),V_-(T)\right]=\frac{V_+(T)}{1+V_-(T)}.
\]
\end{Lemma}
Additionally, since $\delta(0)$ follows a truncated geometric distribution, we have
\[
\mathbb{E}\left[\frac{\sum_{j\in\mathcal{H}_0}\mathbf{1}\left\{W_j\geq T,L_j=1\right\}}{r\sum_{j\in\mathcal{H}}\mathbf{1}\left\{W_j\geq T,L_j=0\right\}+r}\right]=\mathbb{E}\delta(T)/r\leq\mathbb{E}\delta(0)/r<1.
\]
\end{proof}

\begin{proof}[Proof via flip-one]

We consider FDR control under the condition that $(\mathbf{W},\mathbf{L})$ are competition statistics. Let 
\[
T_i=\inf\left\{t\in\{W_j:L_j=1\}:\frac{r\sum_{j\neq i}\mathbf{1}\{W_j\geq t,L_j=0\}+r}{\left(\sum_{j\neq i}\mathbf{1}\{W_j\geq t,L_j=0\}+\mathbf{1}\{W_i\geq t\}\right)\vee1}\leq\alpha\right\},
\]
if $\mathbf{1}\{W_i\geq T,L_i=1\}=1$, then $T=T_i$. Consequently,
\[
\mathbb{E}\left[\frac{\mathbf{1}\left\{W_i\geq T,L_i=1\right\}}{r\sum_{j\in\mathcal{H}}\mathbf{1}\left\{W_j\geq T,L_j=0\right\}+r}\right]=\mathbb{E}\left[\frac{\mathbf{1}\left\{W_i\geq T_i,L_i=1\right\}}{r\sum_{j\in\mathcal{H}\backslash\{i\}}\mathbf{1}\left\{W_j\geq T_i,L_j=0\right\}+r}\right].
\]
Since $\sigma\{T_i\}\subseteq\sigma\{\mathbf{W},\mathbf{L}_{-i}\}$, we have
\begin{align*}
    &\mathbb{E}\left[\frac{\mathbf{1}\left\{W_i\geq T_i,L_i=1\right\}}{r\sum_{j\in\mathcal{H}\backslash\{i\}}\mathbf{1}\left\{W_j\geq T_i,L_j=0\right\}+r}\right]\\
    =&\mathbb{E}\left[\mathbb{E}\left[\frac{\mathbf{1}\left\{W_i\geq T_i,L_i=1\right\}}{r\sum_{j\in\mathcal{H}\backslash\{i\}}\mathbf{1}\left\{W_j\geq T_i,L_j=0\right\}+r}\Big|\sigma\{\mathbf{W},\mathbf{L}_{-i}\}\right]\right]\\
    =&\mathbb{E}\left[P(L_i=1|\mathbf{W},\mathbf{L}_{-i})\cdot\frac{\mathbf{1}\left\{W_i\geq T_i\right\}}{r\sum_{j\in\mathcal{H}\backslash\{i\}}\mathbf{1}\left\{W_j\geq T_i,L_j=0\right\}+r}\right]\\
    =&\frac{r}{1+r}\left(\mathbb{E}\left[\frac{\mathbf{1}\left\{W_i\geq T_i,L_i=1\right\}}{r\sum_{j\in\mathcal{H}\backslash\{i\}}\mathbf{1}\left\{W_j\geq T_i,L_j=0\right\}+r}\right]+\mathbb{E}\left[\frac{\mathbf{1}\left\{W_i\geq T_i,L_i=0\right\}}{r\sum_{j\in\mathcal{H}\backslash\{i\}}\mathbf{1}\left\{W_j\geq T_i,L_j=0\right\}+r}\right]\right)
\end{align*}
and then we have
\[
\mathbb{E}\left[\frac{\mathbf{1}\left\{W_i\geq T,L_i=1\right\}}{r\sum_{j\in\mathcal{H}\backslash\{i\}}\mathbf{1}\left\{W_j\geq T,L_j=0\right\}+r}\right]\leq\mathbb{E}\left[\frac{\mathbf{1}\left\{W_i\geq T_i,L_i=0\right\}}{\sum_{j\in\mathcal{H}\backslash\{i\}}\mathbf{1}\left\{W_j\geq T_i,L_j=0\right\}+1}\right].
\]

In fact, a lemma guarantees that $T_i$ takes at most two values across different indices $i$.
 
\begin{Lemma}
    \label{slem:biovervariable}
    If $\mathbf{1}\left\{W_i\geq T,L_i=0\right\}=1$, we have the following facts
    \begin{enumerate}
        \item $T_i\leq T$.
        \item $\mathbf{1}\left\{W_k\geq T_i,L_k=0\right\}=1\Leftrightarrow T_i=T_k$.
        \item $\mathbf{1}\left\{W_k\geq T_i,L_k=0\right\}=0\Leftrightarrow T=T_k$.
    \end{enumerate}
\end{Lemma}

 With Lemma~\ref{slem:biovervariable}, we have
 \[
 \mathbb{E}\left[\frac{\sum_{j\in\mathcal{H}_0}\mathbf{1}\left\{W_j\geq T,L_j=1\right\}}{r\sum_{j\in\mathcal{H}}\mathbf{1}\left\{W_j\geq T,L_j=0\right\}+r}\right]=\sum_{i\in\mathcal{H}_0}\mathbb{E}\left[\frac{\mathbf{1}\left\{W_i\geq T_i,L_i=0\right\}}{\sum_{j\in\mathcal{H}\backslash\{i\}}\mathbf{1}\left\{W_j\geq T_i,L_j=0\right\}+1}\right]<1.
 \]
\end{proof}

\subsection{Comparison of three proofs}

We briefly outline the main characteristics of the three proof methods.

The martingale proof is the earliest method for establishing FDR control for competition procedures. It works under the assumption of competition statistics, where $\mathbb{P}\{L_j=1\mid\mathbf{W},\mathbf{L}_{-j}\}=r/(1+r)$. Its key insight is to construct the process $\{\widetilde{M}_k\}$, which is shown to be a reverse supermartingale. The FDR bound then follows from Doob's stopping theorem. A notable advantage of this proof is that it reveals a sufficient condition more general than the competition statistics framework: the FDR control holds whenever the process forms a reverse supermartingale with a corresponding stopping time.

The combination proof also assumes competition statistics. Its main idea is to construct an auxiliary random variable $\delta(t)$ that dominates the quantity of interest in expectation. The key advantage is that the fraction $V_+(T)/(rR_-(T)+r)$, whose distribution is difficult to obtain explicitly, is dominated by $\delta(0)/r$, a random variable with a known truncated negative geometric distribution. Specifically, $\delta(T)$ tracks the number of false discoveries when no negative labels precede them at threshold $t$, and its conditional expectation equals $V_+(T)/(1+V_-(T))$. Since $\delta(0)$ follows a truncated geometric distribution, its expectation is straightforward to bound. This dominance replaces the intractable distributional calculation with a simple distributional bound.

The flip-one proof is the most flexible. It works directly under sub-competition statistics, where $\mathbb{P}\{L_j=1\mid\mathbf{W},\mathbf{L}_{-j}\}\leq r/(1+r)$, without requiring the bridge construction needed by the other two methods. Its strategy is based on a deeper analysis of the threshold. After flipping the label of a single null hypothesis to $0$, the original threshold $T$ changes to $T_i$. Lemma~\ref{slem:biovervariable} guarantees that $T_i$ takes at most two values and that its behavior after flipping can be fully predicted. This threshold analysis allows the sub-competition condition to be applied to bound each null hypothesis individually and also naturally extends to general dependence structures and asymptotic analysis.

\subsection{The bridge between sub-competition statistics and competition statistics}

First, it is important to clarify that even without establishing a bridge between sub-competition statistics and competition statistics, the proof of the 'flip-one' method can be straightforwardly extended to general sub-competition statistics. For the other two methods, however, we need to construct the following additional bridge.

Suppose $(\mathbf{W},\mathbf{L})$ are sub-competition statistics. Without loss of generality, assume $W_1<W_2<W_3\cdots<W_m$. Construct a sequence of random variables $Y_1,Y_2,\cdots,Y_m$ one by one, such that their distributions satisfy
\[
\mathbb{P}\{Y_j=1\mid \mathbf{L}_{\{i:i\leq j\}},\mathbf{Y}_{\{i:i<j\}},\mathbf{L}_{\mathcal{H}_1},\mathbf{W}\}=1-L_j-\frac{r}{1+r}(1-L_j)(1-p_j(\mathbf{L}_{\{i:i< j\}}))^{-1},\quad\forall j\in\mathcal{H}_0
\]
and $Y_j=0,\forall j\in\mathcal{H}_1$, where
\[
p_j(\mathbf{L}_{\{i:i< j\}})=\mathbb{P}\{L_j=1\mid \mathbf{L}_{\{i:i<j\}},\mathbf{L}_{\mathcal{H}_1},\mathbf{W}\}.
\]
At this point, we have $L_j\perp \mathbf{Y}_{\{i:i<j\}}\mid\mathbf{L}_{\{i:i<j\}},\forall j\in\mathcal{H}_0$, and
\[
\mathbb{P}\left\{L_j+Y_j=1\mid\mathbf{Y}_{\{i:i<j\}},\mathbf{L}_{\{i:i<j\}},\mathbf{L}_{\mathcal{H}_1},\mathbf{W}\right\}=\frac{r}{1+r},\quad \forall j\in\mathcal{H}_0.
\]
Furthermore, for any $k>j,k\in\mathcal{H}_0$,
\begin{align*}
&\mathbb{P}\left\{L_{k}+Y_{k}=1\mid\mathbf{Y}_{\{i:i<j\}},\mathbf{L}_{\{i:i<j\}},\mathbf{L}_{\mathcal{H}_1},\mathbf{W}\right\}\\
=&\mathbb{E}\left[\mathbb{P}\left\{L_{k}+Y_{k}=1\mid\mathbf{Y}_{\{i:i<k\}},\mathbf{L}_{\{i:i<k\}},\mathbf{L}_{\mathcal{H}_1},\mathbf{W}\right\}\mid\mathbf{Y}_{\{i:i<j\}},\mathbf{L}_{\{i:i<j\}},\mathbf{L}_{\mathcal{H}_1},\mathbf{W}\right]\\
=&\mathbb{E}\left[\frac{r}{1+r}\mid\mathbf{Y}_{\{i:i<j\}},\mathbf{L}_{\{i:i<j\}},\mathbf{L}_{\mathcal{H}_1},\mathbf{W}\right]=\frac{r}{1+r},
\end{align*}
Let $Z_j=L_j+Y_j$, we have
\[
\mathbb{P}\{Z_{j_1}=1\mid \mathbf{Z}_{\{i:i<j_2\}},\mathbf{L}_{\mathcal{H}_1},\mathbf{W}\}=\frac{r}{1+r},\quad\forall j_1\in\mathcal{H}_0,j_2\leq j_1,
\]
and for any $k>j,k\in\mathcal{H}_0$,
\begin{align*}
    &\mathbb{P}\{Z_j=1\mid \mathbf{Z}_{\{i:i<j\}},Z_{k},\mathbf{L}_{\mathcal{H}_1},\mathbf{W}\}\\
    =&\frac{\mathbb{P}\{Z_{k}\mid \mathbf{Z}_{\{i:i\leq j\}},\mathbf{L}_{\mathcal{H}_1},\mathbf{W}\}\mathbb{P}\{Z_{j}\mid \mathbf{Z}_{\{i:i<j\}},\mathbf{L}_{\mathcal{H}_1},\mathbf{W}\}}{\mathbb{P}\{Z_{k}\mid \mathbf{Z}_{\{i:i<j\}},\mathbf{L}_{\mathcal{H}_1},\mathbf{W}\}}\\
    =&\mathbb{P}\{Z_{j}\mid \mathbf{Z}_{\{i:i<j\}},\mathbf{L}_{\mathcal{H}_1},\mathbf{W}\}=\frac{r}{1+r}.
\end{align*}
Thus consider the filtration $\{\sigma_{t}\}$
\[
\sigma_t=\sigma\left\{\sum_{j\in\mathcal{H}_0(u)}\mathbf{1}\{Y_j=1\},\sum_{j\in\mathcal{H}_0(u)}\mathbf{1}\{Y_j=0\},\sum_{j\in\mathcal{H}_0(u)}\mathbf{1}\{L_j=1\},\sum_{j\in\mathcal{H}_0(u)}\mathbf{1}\{L_j=0\},\mathbf{L}_{\mathcal{H}_1},\mathbf{W},\forall u\leq t\right\},
\]
Note that $(\mathbf{W},\mathbf{Z})$ does not form competition statistics. Even if it did, FDR control would not follow directly, because the rejection set of the competition procedure depends on $(\mathbf{W},\mathbf{L})$ rather than $(\mathbf{W},\mathbf{Z})$. However, we do not need $(\mathbf{W},\mathbf{Z})$ to be competition statistics. The construction above already provides enough structure to satisfy the conditions required by the martingale proof.

\section{Proofs for the Equivalent Forms}
\label{app:ef}

\begin{proof}[Proof of Theorem~\ref{thm:cf_to_cp}]

If $X_j\geq T$, with the definition of $T$,
\[
\frac{m}{1+n}\frac{1+\sum_{i=1}^n\mathbf{1}\{Y_i\geq X_j\}}{1\vee\sum_{i=1}^m\mathbf{1}\{X_i\geq T\}}\leq\frac{m}{1+n}\frac{1+\sum_{i=1}^n\mathbf{1}\{Y_i\geq T\}}{1\vee\sum_{i=1}^m\mathbf{1}\{X_i\geq T\}}\leq \alpha.
\]
So we have for any $j$ that $X_j\geq T$,
\[
P_j(\mathbf{X},\mathbf{Y})=\frac{1+\sum_{i=1}^n\mathbf{1}\{Y_i\geq X_j\}}{1+n}\leq\alpha\frac{\sum_{i=1}^m\mathbf{1}\{X_i\geq T\}}{m},
\]
and then
\[
\left\{k\in[m]:X_k\geq T\right\}\subseteq\left\{k\in[m]:P_k(\mathbf{X},\mathbf{Y})\leq\alpha\frac{\sum_{i=1}^m\mathbf{1}\{X_i\geq T\}}{m}\right\}.
\]
If $X_j<T$, with the definition of $T$,
\[
\frac{m}{1+n}\frac{1+\sum_{i=1}^n\mathbf{1}\{Y_i\geq X_j\}}{1\vee\sum_{i=1}^m\mathbf{1}\{X_i\geq T\}}\geq\frac{m}{1+n}\frac{1+\sum_{i=1}^n\mathbf{1}\{Y_i\geq X_j\}}{1\vee\sum_{i=1}^m\mathbf{1}\{X_i\geq X_j\}}>\alpha.
\]
So we have for any $j$ that $X_j<T$,
\[
P_j(\mathbf{X},\mathbf{Y})=\frac{1+\sum_{i=1}^n\mathbf{1}\{Y_i\geq X_j\}}{1+n}>\alpha\frac{\sum_{i=1}^m\mathbf{1}\{X_i\geq X_j\}}{m},
\]
and then
\[
\left\{k\in[m]:P_k(\mathbf{X},\mathbf{Y})\leq\alpha\frac{\sum_{i=1}^m\mathbf{1}\{X_i\geq X_j\}}{m}\right\}\subsetneq\left\{k\in[m]:X_k\geq X_j\right\}.
\]
Because the order of $P_j$ is the same as that of $X_j$,
\[
\mathcal{R}^*_{\alpha}(\mathbf{X},\mathbf{Y})=\mathcal{R}_{\alpha}(\mathbf{P}(\mathbf{X},\mathbf{Y})).
\]
Furthermore, because
\[
K=|\mathcal{R}^*_{\alpha}(\mathbf{X},\mathbf{Y})|=|\mathcal{R}_{\alpha}(\mathbf{P}(\mathbf{X},\mathbf{Y}))|,
\]
it is evident that
\[
\frac{1+\sum_{i=1}^n\mathbf{1}\{Y_i\geq T\}}{1+n}\leq \alpha\frac{\sum_{i=1}^m\mathbf{1}\{X_i\geq T\}}{m}=\frac{\alpha K}{m}=q_K^{m,\alpha}.
\]
\end{proof}

\begin{proof}[Proof of Theorem~\ref{thm:cp_to_cf}]

If $R_+(0)=0$, both $\mathcal{R}_{\alpha,r}(\mathbf{W},\mathbf{L})$ and $\mathcal{R}^*_{\alpha}(\mathbf{P}_{\mathcal{R}_+(0)},\mathbf{P}_{\mathcal{R}_-(0)})$ are $0$. The two rejection sets are equal, so we only need to consider the case $R_+(0)>0$. If $P_j/E_j\leq q^{R_+(0),\alpha}_K$, we have
\[
r\frac{1+R_-(W_j)}{1\vee R_+(W_j)}=r\frac{1+R_-(W_j)}{R_+(0)}\frac{R_+(0)}{1\vee R_+(W_j)}\leq\alpha\frac{K}{R_+(0)}\frac{R_+(0)}{1\vee R_+(W_j)}=\alpha\frac{K}{1\vee R_+(W_j)}.
\]
Because the values of $E_j$ are all equal and $W_j$ and $P_j$ have the same order, according to the definition of $K$, we have for any $j$ that $P_j/E_j\leq q^{R_+(0),\alpha}_K$, $R_+(W_j)=|\{i:W_i\geq W_j,L_i=1\}|\leq K$. Hence, there exist $j_K$ for which $R_+(W_{j_K})=K, P_{j_K}/E_{j_K}\leq q_K^{R_+(0),\alpha}$ and
\[
r\frac{1+R_-(W_{j_K})}{1\vee R_+(W_{j_K})}\leq \alpha\frac{K}{K}=\alpha
\]
which implies that $T\leq W_{j_K}$ and 
\[
\mathcal{R}^*_{\alpha}(\mathbf{P}_{\mathcal{R}_+(0)},\mathbf{P}_{\mathcal{R}_-(0)};\mathbf{E})\subseteq\mathcal{R}_{\alpha,r}(\mathbf{W},\mathbf{L}).
\]
Similarly, for any $j$ that $P_j/E_j> q^{R_+(0),\alpha}_K$, with the definition of $K$, $P_j/E_j> q^{R_+(0),\alpha}_{R_+(W_j)}$ and so $R_+(W_j)>K$,
\[
r\frac{1+R_-(W_j)}{1\vee R_+(W_j)}>\alpha\frac{R_+(W_j)}{1\vee R_+(W_j)}=\alpha,
\]
which implies
\[
\mathcal{R}_{\alpha,r}(\mathbf{W},\mathbf{L})\subseteq\mathcal{R}^*_{\alpha}(\mathbf{P}_{\mathcal{R}_+(0)},\mathbf{P}_{\mathcal{R}_-(0)};\mathbf{E}).
\]
So we have
\[
\mathcal{R}_{\alpha,r}(\mathbf{W},\mathbf{L})=\mathcal{R}^*_{\alpha}(\mathbf{P}_{\mathcal{R}_+(0)},\mathbf{P}_{\mathcal{R}_-(0)};\mathbf{E}).
\]
\end{proof}

\section{Proofs for the Generalized BH Procedures}
\label{app:gbh}

\begin{proof}[Proof of Theorem~\ref{thm:fdr_wbh}]

By definition, we have $K=|\mathcal{R}_{\alpha}(\mathbf{P}')|$,
\begin{align*}
    &\mathbb{E}\left[\frac{\sum_{j\in\mathcal{H}_0}\mathbf{1}\{P_j/E_j\leq q_K^{m,\alpha}\}}{1\vee\sum_{i\in\mathcal{H}}\mathbf{1}\{P_i/E_i\leq q_K^{m,\alpha}\}}\big| \mathbf{E}\right]\\
    =&\sum_{j\in\mathcal{H}_0}\mathbb{E}\left[\sum_{k=1}^m\frac{\mathbf{1}\{P_j/E_j\leq q_k^{m,\alpha}\}}{k}\mathbf{1}\{K=k\}\big| \mathbf{E}\right]\\
    =&\sum_{j\in\mathcal{H}_0}\sum_{k=1}^m\frac{1}{k}\mathbb{P}\left\{P_j/E_j\leq q_k^{m,\alpha},|\mathcal{R}_{\alpha}(\mathbf{P}')|=k\big| \mathbf{E}\right\}\\
    \leq&\sum_{j\in\mathcal{H}_0}\sum_{k=1}^m\frac{\alpha E_j}{m}\mathbb{P}\left\{|\mathcal{R}_{\alpha}(\mathbf{P}')|=k\big| P_j\leq q_k^{m,\alpha}E_j, \mathbf{E}\right\}
\end{align*}
Similarly, if $\mathbf{E}$ is given as the condition, $|\mathcal{R}_{\alpha}(\mathbf{P}')|\leq k$ is a nondecreasing set with respect to $\mathbf{P}_{-j}$ for any $k$ and any $j$. So
\begin{align*}
    \mathrm{FDR}&=\mathbb{E}\left[\mathbb{E}\left[\mathrm{FDP}\mid \mathbf{E}\right]\right]\\
    &\leq\mathbb{E}\left[\sum_{j\in\mathcal{H}_0}\sum_{k=1}^m\frac{\alpha E_j}{m}\mathbb{P}\left\{|\mathcal{R}_{\alpha}(\mathbf{P}')|=k\big| P_j\leq q_k^{m,\alpha}E_j, \mathbf{E}\right\}\right]\\
    &\leq\frac{\alpha}{m}\sum_{j\in\mathcal{H}_0}\mathbb{E}E_j.
\end{align*}
\end{proof}

\begin{proof}[Proof of Lemma~\ref{lem:cp_weights_control}]

With the definition, we have
\begin{align*}
    &\sum_{j\in\mathcal{H}_0}\mathbb{E}\frac{1\vee R_+(0)}{r+rV_-(0)}\mathbf{1}\{L_j=1\}\\
    =&\sum_{j\in\mathcal{H}_0}\mathbb{E}\frac{\sum_{i\in\mathcal{H}}\mathbf{1}\{L_i=1\}}{r+rV_-(0)}\mathbf{1}\{L_j=1\}\\
    =&\sum_{i\in\mathcal{H}}\mathbb{E}\frac{\sum_{j\in\mathcal{H}_0}\mathbf{1}\{L_j=1\}}{r+rV_-(0)}\mathbf{1}\{L_i=1\}\\
    =&\sum_{i\in\mathcal{H}}\mathbb{E}\frac{V_+(0)}{r+rV_-(0)}\mathbf{1}\{L_i=1\}\\
    \leq&m\mathbb{E}\frac{V_+(0)}{r+rV_-(0)}
\end{align*}
The first equality holds because if $\sum_{i\in\mathcal{H}}\mathbf{1}\{L_i=1\}=0$, then $L_j=0$ for all $j$ and the expectation is zero. Hence we may replace $1\vee R_+(0)$ with $\sum_{i\in\mathcal{H}}\mathbf{1}\{L_i=1\}$. Furthermore,
\[
\mathbb{E}\frac{V_+(0)}{r+rV_-(0)}=\sum_{k=0}^{m_0}\binom{m_0}{k}\frac{k}{r+rm_0-rk}\left(\frac{r}{1+r}\right)^k\left(\frac{1}{1+r}\right)^{m_0-k}<1,
\]
and therefore
\[
\sum_{j\in\mathcal{H}_0}\mathbb{E}\frac{1\vee R_+(0)}{r+rR_-(0)}\mathbf{1}\{L_j=1\}\leq\sum_{j\in\mathcal{H}_0}\mathbb{E}\frac{1\vee R_+(0)}{r+rV_-(0)}\mathbf{1}\{L_j=1\}\leq m.
\]
\end{proof}

\begin{proof}[Proof of Corollary~\ref{coro:fdr_bounded_bh}]

By definition, we have $K=|\mathcal{R}_{\alpha}(\mathbf{P})|$,
\begin{align*}
    &\mathbb{E}\left[\frac{\sum_{j\in\mathcal{H}_0}\mathbf{1}\{P_j\leq q_K^{m,\alpha}\}}{1\vee\sum_{i\in\mathcal{H}}\mathbf{1}\{P_i\leq q_K^{m,\alpha}\}}\right]=\sum_{j\in\mathcal{H}_0}\mathbb{E}\left[\sum_{k=1}^m\frac{\mathbf{1}\{P_j\leq q_k^{m,\alpha}\}}{k}\mathbf{1}\{K=k\}\right]\\
    =&\sum_{j\in\mathcal{H}_0}\sum_{k=1}^m\frac{1}{k}\mathbb{P}\left\{P_j\leq q_k^{m,\alpha},|\mathcal{R}_{\alpha}(\mathbf{P})|=k\right\}\\
    \leq&\sum_{j\in\mathcal{H}_0}\sum_{k=1}^m\frac{1}{k}\mathbb{P}\left\{|\mathcal{R}_{\alpha}(\mathbf{P})|=k, Q_j\leq q_k^{m,\alpha}\right\}
\end{align*}
The inequality in the third line holds because $\mathbb{P}(Q_j\leq P_j)=1$. Unlike the standard FDR control proof for the BH procedure, the condition $Q_j \leq q^{m,\alpha}_k$ for the reference variable $Q_j$ does not immediately yield a non-decreasing set. Hence, we need to take a step back.
\begin{align*}
    &\left\{P_j\leq q_k^{m,\alpha},|\mathcal{R}_{\alpha}(\mathbf{P})|=k\right\}\\
    =&\left\{P^j_{(k-1)}\leq q^{m,\alpha}_k,P^j_{(k)}> q^{m,\alpha}_{k+1},P^j_{(k+1)}> q^{m,\alpha}_{k+2},\cdots,P^j_{(m-1)}> q^{m,\alpha}_k,P_j\leq q^{m,\alpha}_m\right\}
\end{align*}
where $P^j_{(i)}$ denotes the $i$-th order statistic of $\mathbf{P}$ excluding $P_j$. It is clear that $\{\boldsymbol{p}\in\mathbb{R}_*^{m-1}:p_{(k)}>q^{m,\alpha}_{(k+1)},\cdots,p_{(m-1)}>q^{m,\alpha}_{(m)}\}$ is a nondecreasing set. So
\begin{align*}
    &\mathrm{FDR}=\sum_{j\in\mathcal{H}_0}\sum_{k=1}^m\frac{1}{k}\mathbb{P}\left\{|\mathcal{R}_{\alpha}(\mathbf{P})|=k, P_j\leq q_k^{m,\alpha}\right\}\\
    \leq&\sum_{j\in\mathcal{H}_0}\sum_{k=1}^m\frac{1}{k}\mathbb{P}\left\{P^j_{(k-1)}\leq q^{m,\alpha}_k,P^j_{(k)}> q^{m,\alpha}_{k+1},\cdots,P^j_{(m-1)}> q^{m,\alpha}_{m},Q_j\leq q^{m,\alpha}_k\right\}\\
    \leq&\sum_{j\in\mathcal{H}_0}\sum_{k=1}^m\frac{\alpha}{m}\mathbb{P}\left\{P^j_{(k-1)}\leq q^{m,\alpha}_k,P^j_{(k)}> q^{m,\alpha}_{k+1},\cdots,P^j_{(m-1)}> q^{m,\alpha}_{m}\big|Q_j\leq q^{m,\alpha}_k\right\}\\
    =&\sum_{j\in\mathcal{H}_0}\sum_{k=1}^m\frac{\alpha}{m}\left(\mathbb{P}\left\{P^j_{(k)}> q^{m,\alpha}_{k+1},\cdots,P^j_{(m-1)}> q^{m,\alpha}_m\big|Q_j\leq q^{m,\alpha}_k\right\}\right.\\
    &\quad-\left.\mathbb{P}\left\{P^j_{(k-1)}> q^{m,\alpha}_{k},P^j_{(k)}> q^{m,\alpha}_{k+1},\cdots,P^j_{(m-1)}> q^{m,\alpha}_m\big|Q_j\leq q^{m,\alpha}_k\right\}\right)\\
    \leq&\sum_{j\in\mathcal{H}_0}\frac{\alpha}{m}\leq\alpha\frac{m_0}{m}.
\end{align*}
\end{proof}

\begin{proof}[Proof of Theorem~\ref{thm:fdr_ran_problem}]

By definition, we have $K^V=|\mathcal{R}_{\alpha}(\mathbf{P}_{\eta(V)})|$,
\begin{align*}
    &\mathbb{E}\left[\frac{\sum_{j\in\mathcal{H}_0\cap\eta(V)}\mathbf{1}\{P_j\leq q_{K^V}^{|\eta(V)|,\alpha}\}}{1\vee\sum_{i\in\eta(V)}\mathbf{1}\{P_i\leq q_{K^V}^{|\eta(V)|,\alpha}\}}\big| V\right]\\
    =&\sum_{j\in\mathcal{H}_0\cap\eta(V)}\mathbb{E}\left[\sum_{k=1}^{|\eta(V)|}\frac{\mathbf{1}\{P_j\leq q_k^{|\eta(V)|,\alpha}\}}{k}\mathbf{1}\{K^V=k\}\big| V\right]\\
    =&\sum_{j\in\mathcal{H}_0\cap\eta(V)}\sum_{k=1}^{|\eta(V)|}\frac{1}{k}\mathbb{P}\left\{P_j\leq q_k^{|\eta(V)|,\alpha},|\mathcal{R}_{\alpha}(\mathbf{P}_{\eta(V)})|=k\big| V\right\}\\
    \leq&\sum_{j\in\mathcal{H}_0\cap\eta(V)}\sum_{k=1}^{|\eta(V)|}\frac{\alpha}{|\eta(V)|}\mathbb{P}\left\{|\mathcal{R}_{\alpha}(\mathbf{P}_{\eta(V)})|=k\big| P_j\leq q_k^{|\eta(V)|,\alpha},V\right\}.
\end{align*}
Similarly, if $V$ is given as the condition, $|\mathcal{R}_{\alpha}(\mathbf{P}_{\eta(V)})|\leq k$ is a nondecreasing set with respect to $\mathbf{P}_{\eta(V),-j}$ for any $k$ and any $j\in\mathcal{H}_0\cap\eta(V)$. So
\begin{align*}
    \mathrm{FDR}&=\mathbb{E}\left[\mathbb{E}\left[\frac{|\mathcal{H}_0\cap\eta(V)\cap\mathcal{R}_{\alpha}(\mathbf{P}_{\eta(V)})|}{1\vee|\eta(V)\cap\mathcal{R}_{\alpha}(\mathbf{P}_{\eta(V)})|}\big| V\right]\right]\\
    &\leq\mathbb{E}\left[\sum_{j\in\mathcal{H}_0\cap\eta(V)}\sum_{k=1}^{|\eta(V)|}\frac{\alpha}{|\eta(V)|}\mathbb{P}\left\{|\mathcal{R}_{\alpha}(\mathbf{P}_{\eta(V)})|=k\big| P_j\leq q_k^{|\eta(V)|,\alpha},V\right\}\right]\\
    &\leq\alpha\mathbb{E}\frac{|\mathcal{H}_0\cap\eta(V)|}{1\vee|\eta(V)|}\leq\alpha.
\end{align*}
\end{proof}

Theorem~\ref{thm:fdr_cf_rbh} is a corollary of Theorem~\ref{thm:fdr_rbh}, Lemma~\ref{lem:rbh_induce_exch} and Lemma~\ref{lem:embedding}. We first provide the proofs of these three results, and then prove Theorem~\ref{thm:fdr_cf_rbh} as a consequence.

\begin{proof}[Proof of Theorem~\ref{thm:fdr_rbh}]

By definition, we have $K=|\mathcal{R}_{\alpha}(\mathbf{P})|$,
\begin{align*}
    \mathrm{FDR}&=\mathbb{E}\frac{\sum_{j\in\mathcal{H}_0}\mathbf{1}\{P_j\leq q^{m,\alpha}_K\}}{1\vee\sum_{i\in\mathcal{H}}\mathbf{1}\{P_i\leq q^{m,\alpha}_K\}}=\sum_{j\in\mathcal{H}_0}\mathbb{E}\frac{\mathbf{1}\{P_j\leq q^{m,\alpha}_K\}}{1\vee\sum_{i\in\mathcal{H}}\mathbf{1}\{P_i\leq q^{m,\alpha}_K\}}\\
    &=\sum_{j\in\mathcal{H}_0}\mathbb{E}\sum_{k=1}^m\frac{\mathbf{1}\{P_j\leq q^{m,\alpha}_k\}}{k}\mathbf{1}\{K=k\}\\
    &=\sum_{j\in\mathcal{H}_0}\sum_{k=1}^m\frac{1}{k}\mathbb{P}\{P_j\leq q^{m,\alpha}_k,|\mathcal{R}_{\alpha}(\mathbf{P})|=k\}.
\end{align*}
We proceed with a reverse derivation, transforming the standard FDR definition under the BH procedure into its randomized form. Considering that
\begin{align*}
    &\mathbb{P}\left\{P_J\leq q^{m,\alpha}_m,|\mathcal{R}_{\alpha}(\mathbf{P})|=k\right\}\\
    =&\sum_{j\in\mathcal{H}_0}\mathbb{P}\left\{P_J\leq q^{m,\alpha}_m,|\mathcal{R}_{\alpha}(\mathbf{P})|=k,J=j\right\}\\
    =&\sum_{j\in\mathcal{H}_0}\mathbb{P}\left\{P_j\leq q^{m,\alpha}_m,|\mathcal{R}_{\alpha}(\mathbf{P})|=k\big|J=j\right\}\mathbb{P}(J=j)\\
    =&\frac{1}{1\vee|\mathcal{H}_0|}\sum_{j\in\mathcal{H}_0}\mathbb{P}\left\{P_j\leq q^{m,\alpha}_m,|\mathcal{R}_{\alpha}(\mathbf{P})|=k\right\}
\end{align*}
so with the condition of randomized p-variable, we have
\begin{align*}
    \mathrm{FDR}&=\sum_{j\in\mathcal{H}_0}\sum_{k=1}^m\frac{1}{k}\mathbb{P}\{P_j\leq q^{m,\alpha}_k,|\mathcal{R}_{\alpha}(\mathbf{P})|=k\}\\
    &=\sum_{k=1}^m\frac{|\mathcal{H}_0|}{k}\mathbb{P}\{P_J\leq q^{m,\alpha}_k,|\mathcal{R}_{\alpha}(\mathbf{P})|=k\}\\
    &\leq\sum_{k=1}^m\frac{\alpha m_0}{m}\mathbb{P}\{|\mathcal{R}_{\alpha}(\mathbf{P})|=k\big|P_J\leq q^{m,\alpha}_k\}
\end{align*}
Note that due to the randomness of $J$, we must restrict the randomized PRDS condition to order statistics to ensure the formulation is well-defined. As a result, the set $\{\mathbf{P}^J_{(\cdot)}:|\mathcal{R}_{\alpha}(\mathbf{P})|\leq k\}$ is no longer intuitively a non-decreasing set, and further analysis is required. Let
\[
\mathcal{D}_k=\left\{\mathbf{p}\in\mathbb{R}_*^{m-1}:p_{(k-1)}\leq q^{m,\alpha}_k,p_{(k)}> q^{m,\alpha}_{k+1},\cdots,p_{(m-1)}> q^{m,\alpha}_m\right\},
\]
so that $\{\mathbf{P}^J_{(\cdot)}\in\mathcal{D}_k\}=\{|\mathcal{R}_{\alpha}(\mathbf{P})|=k\}$ given $P_J\leq q_k^{m,\alpha}$, and let
\[
\mathcal{C}_k=\left\{\mathbf{p}\in\mathbb{R}_*^{m-1}:p_{(k)}> q^{m,\alpha}_{k+1},\cdots,p_{(m-1)}> q^{m,\alpha}_m\right\},
\]
so that $\mathcal{D}_k=\mathcal{C}_k\setminus\mathcal{C}_{k-1}$, where $\mathcal{C}_0=\emptyset,\mathcal{C}_m=\mathbb{R}_*^{m-1}$. The sets $\mathcal{C}_k$, $k=0,1,\cdots,m$, are all nondecreasing. Hence, with the condition of randomized $\mathrm{PRDS}_{\mathcal{H}_0}$,
\begin{align*}
    \mathrm{FDR}&\leq\sum_{k=1}^m\frac{\alpha m_0}{m}\mathbb{P}\{|\mathcal{R}_{\alpha}(\mathbf{P})|=k\big|P_J\leq q^{m,\alpha}_k\}\\
    &=\sum_{k=1}^m\frac{\alpha m_0}{m}\mathbb{P}\{\mathbf{P}^J_{(\cdot)}\in\mathcal{D}_k\big|P_J\leq q^{m,\alpha}_k\}\\
    &=\sum_{k=1}^m\frac{\alpha m_0}{m}\left(\mathbb{P}\{\mathbf{P}^J_{(\cdot)}\in\mathcal{C}_k\big|P_J\leq q^{m,\alpha}_k\}-\mathbb{P}\{\mathbf{P}^J_{(\cdot)}\in\mathcal{C}_{k-1}\big|P_J\leq q^{m,\alpha}_k\}\right)\\
    &\leq\sum_{k=1}^m\frac{\alpha m_0}{m}\left(\mathbb{P}\{\mathbf{P}^J_{(\cdot)}\in\mathcal{C}_k\big|P_J\leq q^{m,\alpha}_k\}-\mathbb{P}\{\mathbf{P}^J_{(\cdot)}\in\mathcal{C}_{k-1}\big|P_J\leq q^{m,\alpha}_{k-1}\}\right)\\
    &\leq\alpha\frac{m_0}{m}
\end{align*}
\end{proof}

\begin{proof}[Proof of Lemma~\ref{lem:rbh_induce_exch}]
Let $\pi$ be any permutation of $[m]$. Since $(J_1,\dots,J_m)$ is a uniform permutation independent of $\mathbf{X}$, the permuted vector $(J_{\pi(1)},\dots,J_{\pi(m)})$ has the same distribution as the original. Therefore, for any measurable set $A\subseteq\mathbb{R}_*^m$,
\[
\mathbb{P}\{\mathbf{Z}\in A\}=\mathbb{P}\{(X_{J_1},\dots,X_{J_m})\in A\}=\mathbb{P}\{(X_{J_{\pi(1)}},\dots,X_{J_{\pi(m)}})\in A\}=\mathbb{P}\{(Z_{\pi(1)},\dots,Z_{\pi(m)})\in A\},
\]
so $\mathbf{Z}$ is exchangeable.
\end{proof}

\begin{proof}[Proof of Lemma~\ref{lem:embedding}]
Condition on $|\mathcal{H}_0^{\mathrm{test}}|$ and write $m_{0t}=|\mathcal{H}_0^{\mathrm{test}}|$, $m_{0c}=m_0-m_{0t}=|\mathcal{H}^{\mathrm{cal}}|$. The split is uniform:
\[
\mathbb{P}\{\mathcal{H}^{\mathrm{cal}}=A\mid m_{0c}\}=\binom{m_0}{m_{0c}}^{-1},\quad\forall A\subseteq\mathcal{H}_0,\ |A|=m_{0c}.
\]

Fix an arbitrary permutation $\boldsymbol{l}=(l_1,\dots,l_{m_0})$ of $[m_0]$. Independently of $\mathbf{X}$, the event $\{J_1=l_1,\dots,J_{m_0}=l_{m_0}\}$ occurs iff $\{l_1,\dots,l_{m_{0t}}\}$ is chosen as $\mathcal{H}_0^{\mathrm{test}}$ (probability $\binom{m_0}{m_{0t}}^{-1}$) and then ordered as $(l_1,\dots,l_{m_{0t}})$ (probability $1/m_{0t}!$), and $\{l_{m_{0t}+1},\dots,l_{m_0}\}$ is ordered as $(l_{m_{0t}+1},\dots,l_{m_0})$ (probability $1/m_{0c}!$). Hence
\[
\mathbb{P}\{J_1=l_1,\dots,J_{m_0}=l_{m_0}\}=\binom{m_0}{m_{0t}}^{-1}\frac{1}{m_{0t}!}\frac{1}{m_{0c}!}=\frac{1}{m_0!}.
\]
Thus $(J_1,\dots,J_{m_0})$ is a uniform permutation of $[m_0]$, independent of $\mathbf{X}_{\mathcal{H}_1}$. That is, the two-stage construction (random split followed by independent permutations of each part) is equivalent to first applying a global uniform permutation to all null indices and then taking the first $m_{0t}$ elements as the test set. By Lemma~\ref{lem:rbh_induce_exch}, a global uniform permutation induces exchangeability, so for any permutation $\pi$ of $[m_0]$ and any measurable set $A$,
\[
\mathbb{P}\{(Z_{1},\dots,Z_{m_0})\in A\mid\mathbf{Z}_{\mathcal{H}_1}\}=\mathbb{P}\{(Z_{\pi(1)},\dots,Z_{\pi(m_0)})\in A\mid\mathbf{Z}_{\mathcal{H}_1}\}.
\]
Therefore $(Z_1,\dots,Z_{m_0})$ are exchangeable conditional on $(Z_{m_0+1},\dots,Z_m)$.
\end{proof}

\begin{proof}[Proof of Theorem~\ref{thm:fdr_cf_rbh}]
Condition on $|\mathcal{H}_0^{\mathrm{test}}|=m_{0t}$, so $|\mathcal{H}^{\mathrm{cal}}|=m_0-m_{0t}$. Let $J_1,\dots,J_{m_{0t}}$ be a random permutation of $\mathcal{H}^{\mathrm{test}}$ and $J_{m_{0t}+1},\dots,J_{m_0}$ a random permutation of $\mathcal{H}^{\mathrm{cal}}$, independent of $\mathbf{X}$. Set $Z_i=X_i$ for $i=m_0+1,\dots,m$ and $Z_i=X_{J_i}$ for $i=1,\dots,m_0$.

Define conformal p-values $\mathbf{U}\in\mathbb{R}_*^{m-m_0+m_{0t}}$ for the test set $\{1,\dots,m_{0t}\}\cup\{m_0+1,\dots,m\}$ using $\{m_{0t}+1,\dots,m_0\}$ as the calibration set, that is
\[
U_j=\frac{1+\sum_{i=m_{0t}+1}^{m_0}\mathbf{1}\{Z_i\geq Z_j\}}{1+m_0-m_{0t}},\quad j=1,\dots,m_{0t},
\]
\[
U_j=\frac{1+\sum_{i=m_{0t}+1}^{m_0}\mathbf{1}\{Z_i\geq Z_{j+m_0-m_{0t}}\}}{1+m_0-m_{0t}},\quad j=m_{0t}+1,\dots,m_1+m_{0t}.
\]
By Lemma~\ref{lem:embedding}, $(Z_1,\dots,Z_{m_0})$ are exchangeable conditional on $(Z_{m_0+1},\dots,Z_m)$. Hence each $U_j$ is a p-variable and $\mathbf{U}$ satisfies the PRDS condition with respect to the null indices $\{1,\dots,m_{0t}\}$. Moreover, $J_1$ is uniformly distributed over $\mathcal{H}^{\mathrm{test}}_0$ and independent of $\mathbf{X}$. By construction $P_{J_1}=U_1$ and the order statistics satisfy $\mathbf{P}^{J_1}_{(\cdot)}=\mathbf{U}^{1}_{(\cdot)}$, so
\[
\mathbb{P}\{P_{J_1}\leq t\mid |\mathcal{H}_0^{\mathrm{test}}|\}=\mathbb{P}\{U_1\leq t\}\leq t,\quad t\in[0,1],
\]
and for any nondecreasing set $C\subseteq\mathbb{R}_*^{m-m_0+m_{0t}-1}$,
\[
\mathbb{P}\{\mathbf{P}^{J_1}_{(\cdot)}\in C\mid P_{J_1}\leq t,\ |\mathcal{H}_0^{\mathrm{test}}|\}=\mathbb{P}\{\mathbf{U}^{1}_{(\cdot)}\in C\mid U_1\leq t\}
\]
is nondecreasing in $t$. Then let $J$ be $J_1$ with probability $m_{0t}/m_0$ and $J_{m_{0t}+1}$ with probability $(m_{0}-m_{0t})/m_0$, so that $J$ is uniformly distributed over $\mathcal{H}_0$ and independent of $\mathbf{X}$. Define $\mathbf{Q}$ by $Q_j=P_j$ for $j\in\mathcal{H}^{\mathrm{test}}$ and $Q_j=+\infty$ for $j\in\mathcal{H}^{\mathrm{cal}}$. Then
\[
\mathbb{P}\{Q_J\leq t\mid |\mathcal{H}_0^{\mathrm{test}}|\}=\frac{m_{0t}}{m_0}\mathbb{P}\{P_{J_1}\leq t\mid |\mathcal{H}_0^{\mathrm{test}}|\}\leq \frac{m_{0t}}{m_0}t,\quad t\in[0,1],
\]
and for any nondecreasing set $C\subseteq\mathbb{R}_*^{m_1+m_{0t}-1}$, the set $D = \{\boldsymbol{x}\in\mathbb{R}_*^{m-1}: (x_1, \dots, x_{m_1+m_{0t}-1}) \in C\}$ is also nondecreasing and
\[
\mathbb{P}\{\mathbf{Q}^{J}_{(\cdot)}\in D\mid Q_{J}\leq t,\ |\mathcal{H}_0^{\mathrm{test}}|\}=\mathbb{P}\{\mathbf{P}^{J_1}_{(\cdot)}\in C\mid P_{J_1}\leq t,\ |\mathcal{H}_0^{\mathrm{test}}|\}
\]
is nondecreasing in $t$. Therefore $\mathbf{P}$ is randomized BH-valid with weights $m_0/m_{0t}$.
\begin{Lemma}
\label{slem:level_dim}
Let $\mathbf{P}\in\mathbb{R}_*^m$ and $S\subseteq[m]$. If $P_j=+\infty$ for all $j\notin S$, then for any $\alpha\in(0,1)$,
\[
\mathcal{R}_{m\alpha/|S|}(\mathbf{P})=\mathcal{R}_{\alpha}(\mathbf{P}_S),
\]
where $\mathcal{R}_{\alpha}(\mathbf{P}_S)$ denotes the BH procedure applied to the subvector $\mathbf{P}_S$.
\end{Lemma}
Since with Lemma~\ref{slem:level_dim}, $\mathcal{R}_{\alpha}(\mathbf{P})=\mathcal{R}_{m\alpha/(m_1+m_{0t})}(\mathbf{Q})$, then we have
\begin{align*}
    \mathrm{FDR}=&\mathbb{E}\left[\mathbb{E}\left[\frac{|\mathcal{H}_0^{\mathrm{test}}\cap\mathcal{R}_{\alpha}(\mathbf{P})|}{1\vee|\mathcal{R}_{\alpha}(\mathbf{P})|}\Big||\mathcal{H}_0^{\mathrm{test}}|\right]\right]=\mathbb{E}\left[\mathbb{E}\left[\frac{|\mathcal{H}_0\cap\mathcal{R}_{m_0\alpha/m_{0t}}(\mathbf{Q})|}{1\vee|\mathcal{R}_{m_0\alpha/m_{0t}}(\mathbf{Q})|}\Big||\mathcal{H}_0^{\mathrm{test}}|\right]\right]\\
    \leq&\mathbb{E}\left[\mathbb{E}\left[\frac{\sum_{j\in\mathcal{H}_0}\frac{m_{0t}}{m_0}}{m}\cdot\frac{m\alpha}{m_{0t}+m_1}\Big||\mathcal{H}_0^{\mathrm{test}}|\right]\right]=\alpha\mathbb{E}\left[\frac{m_{0t}}{m_{0t}+m_1}\right]\leq\alpha.
\end{align*}
\end{proof}

\section{Embedding Theorems}
\label{app:embedding}

\subsection{Proofs of the three embedding theorems}

\begin{proof}[Proof of Theorem~\ref{thm:id_prds_to_rbhv}]
For any $J$ uniformly distributed over $\mathcal{H}_0$ independent of $\mathbf{P}$ and any nondecreasing set $C\subseteq\mathbb{R}_*^{m-1}$,
\begin{align*}
    \mathbb{P}\{\mathbf{P}^J_{(\cdot)}\in C\mid P_J\leq t\}
    &=\sum_{j\in\mathcal{H}_0}\mathbb{P}\{\mathbf{P}^j_{(\cdot)}\in C\mid P_J\leq t,J=j\}\mathbb{P}\{J=j\mid P_J\leq t\}\\
    &=\sum_{j\in\mathcal{H}_0}\mathbb{P}\{\mathbf{P}^j_{(\cdot)}\in C\mid P_j\leq t\}\frac{\mathbb{P}\{J=j\}\mathbb{P}\{P_j\leq t\}}{\sum_{k\in\mathcal{H}_0}\mathbb{P}\{J=k\}\mathbb{P}\{P_k\leq t\}}.
\end{align*}
Since $P_j$ are identically distributed for $j\in\mathcal{H}_0$, the weight simplifies to $1/|\mathcal{H}_0|$. Hence
\[
\mathbb{P}\{\mathbf{P}^J_{(\cdot)}\in C\mid P_J\leq t\}=\frac{1}{|\mathcal{H}_0|}\sum_{j\in\mathcal{H}_0}\mathbb{P}\{\mathbf{P}^j_{(\cdot)}\in C\mid P_j\leq t\}.
\]
Each term $\mathbb{P}\{\mathbf{P}^j_{(\cdot)}\in C\mid P_j\leq t\}$ is nondecreasing in $t$ by the PRDS condition, so the average is also nondecreasing in $t$. Therefore $\mathbf{P}$ is randomized BH-valid.
\end{proof}

\begin{proof}[Proof of Theorem~\ref{thm:embed_bh}]
For each $j\in\mathcal{H}_0$, let $F_j$ be the cumulative distribution function of $P_j$. Since $P_j$ is a p-variable, $F_j(t)\leq t$ for all $t\in[0,1]$. Let $\mathcal{I}_j\subseteq[0,1]$ denote the set of discontinuity points of $F_j$. Construct $Q_j$ as follows:
\[
Q_j=
\begin{cases}
F_j(P_j), & P_j\in[0,1]\setminus\mathcal{I}_j,\\[4pt]
\mathrm{Unif}\bigl[\lim_{t\to P_j-}F_j(t),\;\lim_{t\to P_j+}F_j(t)\bigr], & P_j\in\mathcal{I}_j,\\[4pt]
\mathrm{Unif}\bigl[F_j(1),\;1\bigr], & P_j\in(1,\infty).
\end{cases}
\]
By construction, $Q_j\leq P_j$ almost surely, so $\mathbb{P}(\mathbf{P}\geq\mathbf{Q})=1$. Moreover, $Q_j$ is uniformly distributed on $[0,1]$, so $\mathbb{P}(Q_j\leq t)=t$ for all $t\in[0,1]$. Furthermore, $Q_j\perp\!\!\!\perp(\mathbf{P}_{-j},\mathbf{Q}_{-j})\mid P_j$, since $Q_j$ is a function of $P_j$ and independent auxiliary randomization. Each $\mathbf{Q}$ uniquely determines $\mathbf{P}\wedge\mathbf{1}$ (componentwise minimum with $1$). Equivalently, $\sigma(\mathbf{P}\wedge\mathbf{1})\subseteq\sigma(\mathbf{Q})$, so the $\sigma$-algebra generated by $\mathbf{P}$ on $[0,1]$ is contained in that generated by $\mathbf{Q}$. In the following discussion, we restrict $t$ to $[0,1]$, since the BH threshold always lies in this interval.

Now let $J$ be uniform over $\mathcal{H}_0$ and independent of $(\mathbf{P},\mathbf{Q})$. For any nondecreasing set $C\subseteq\mathbb{R}_*^{m-1}$,
\begin{align*}
    \mathbb{P}\{\mathbf{P}^J_{(\cdot)}\in C\mid Q_J\leq t\}
    &=\sum_{j\in\mathcal{H}_0}\mathbb{P}\{\mathbf{P}^j_{(\cdot)}\in C\mid Q_J\leq t,J=j\}\mathbb{P}\{J=j\mid Q_J\leq t\}\\
    &=\sum_{j\in\mathcal{H}_0}\mathbb{P}\{\mathbf{P}^j_{(\cdot)}\in C\mid Q_j\leq t\}\frac{\mathbb{P}\{J=j\}\mathbb{P}\{Q_j\leq t\}}{\sum_{k\in\mathcal{H}_0}\mathbb{P}\{J=k\}\mathbb{P}\{Q_k\leq t\}}.
\end{align*}
Since $Q_j$ are identically distributed for $j\in\mathcal{H}_0$, the weight simplifies to $1/|\mathcal{H}_0|$, and
\[
\mathbb{P}\{\mathbf{P}^J_{(\cdot)}\in C\mid Q_J\leq t\}=\frac{1}{|\mathcal{H}_0|}\sum_{j\in\mathcal{H}_0}\mathbb{P}\{\mathbf{P}^j_{(\cdot)}\in C\mid Q_j\leq t\}.
\]
Each $\mathbf{Q}$ uniquely determines $\mathbf{P}\wedge\mathbf{1}$, and the condition $Q_j\leq t$ is equivalent to $F_j(P_j\wedge1)\leq t$ in the sense determined by the piecewise construction of $Q_j$. Since $\mathbf{P}$ is $\mathrm{PRDS}_{\mathcal{H}_0}$, each term $\mathbb{P}\{\mathbf{P}^j_{(\cdot)}\in C\mid Q_j\leq t\}$ is nondecreasing in $t$. Hence the average is also nondecreasing, and $\mathbf{P}$ has controlled randomized $\mathrm{PRDS}_{\mathcal{H}_0}$ by $\mathbf{Q}$.
\end{proof}

\begin{proof}[Proof of Theorem~\ref{thm:embed_cp}]
Let $(\mathbf{W},\mathbf{L})$ be competition statistics with parameter $r$ over $\mathcal{H}_0$. Define the sigma-algebra
\[
\sigma_{\mathcal{H}_1}=\sigma\{V_+(0),V_-(0),\mathbf{W}_{\mathcal{H}_1},\mathbf{W}_{(\cdot:\mathcal{H}_0)},\mathbf{L}_{\mathcal{H}_1}\},
\]
which conditions on the scores and labels of all alternatives, the order statistics of the null scores, and the counts of positive and negative labels among the nulls. Conditional on $\sigma_{\mathcal{H}_1}$, the only remaining randomness is the assignment of labels $1$ and $0$ among the null hypotheses.

We first state a lemma about the conditional distribution of $\mathcal{V}_+(0)$.

\begin{Lemma}
\label{slem:uniform_split}
Conditional on $\sigma_{\mathcal{H}_1}$, the set $\mathcal{V}_+(0)$ is uniformly distributed over all subsets of $\mathcal{H}_0$
\[
\mathbb{P}\{\mathcal{V}_+(0)=A\mid\sigma_{\mathcal{H}_1}\}=\binom{m_0}{|A|}^{-1},\quad\forall A\subseteq\mathcal{H}_0.
\]
\end{Lemma}

Define the transformed statistics as in \eqref{eq:PEq2}. For $j\in\mathcal{R}_+(0)$,
\[
P_j=\frac{1+R_-(W_j)}{1+V_-(0)},\quad
Q_j=\frac{1+V_-(W_j)}{1+V_-(0)},\quad
E_j=\frac{1\vee R_+(0)}{r+rV_-(0)},
\]
and for $j\in\mathcal{R}_-(0)$, set $P_j=Q_j=+\infty$, $E_j=0$. Then conditional on $\sigma_{\mathcal{H}_1}$, the weights $\mathbf{E}$ are constant, $\mathbf{Q}$ are randomized BH-valid, $\mathbf{P}\geq\mathbf{Q}$ almost surely, $\mathbf{P}$ is uniquely determined by $\mathbf{Q}$, and $\mathbf{P}$ has controlled randomized PRDS on $\mathcal{H}_0$ by $\mathbf{Q}$.

Define
\[
K=\sup\left\{k\in[m]:\sum_{j\in\mathcal{H}}\mathbf{1}\{P_j\leq q_k^{R_+(0),\alpha}E_j\}\geq k\right\},
\]
The following lemma establishes the equivalence between the two rejection counts.

\begin{Lemma}
\label{slem:equiv_rejection}
$K$ is the rejection count of the BH procedure at level $\alpha$ applied to the weighted p-values $\mathbf{P}'_{\mathcal{R}_+(0)}=(P_j/E_j)_{j\in\mathcal{R}_+(0)}$, that is
\[
K=|\mathcal{R}_{\alpha}^{\mathrm{BH}}(\mathbf{P}'_{\mathcal{R}_+(0)})|.
\]
\end{Lemma}

Hence the FDR can be expressed as
\begin{align*}
    \mathrm{FDR}=&\mathbb{E}\left[\mathbb{E}\left[\frac{\sum_{j\in\mathcal{H}_0}\mathbf{1}\{P_j\leq q_K^{R_+(0),\alpha}E_j\}}{1\vee K}\;\Big|\;\sigma_{\mathcal{H}_1}\right]\right]\\
    =&\mathbb{E}\left[\sum_{k=1}^m\frac{1}{k}\sum_{j\in\mathcal{H}_0}\mathbb{P}\{P_j\leq q_k^{R_+(0),\alpha}E_j,\;K=k\mid\sigma_{\mathcal{H}_1}\}\right].
\end{align*}

Let $J$ be uniformly distributed over $\mathcal{H}_0$ and independent of $(\mathbf{W},\mathbf{L})$ given $\sigma_{\mathcal{H}_1}$. Using the uniform distribution of $\mathcal{V}_+(0)$,
\begin{align*}
&\mathbb{P}\{K=k,P_J\leq t\mid\sigma_{\mathcal{H}_1}\}
=\sum_{j\in\mathcal{H}_0}\mathbb{P}\{K=k,P_j\leq t,J=j\mid\sigma_{\mathcal{H}_1}\}\\
=&\mathbb{E}_{\mathcal{V}_+(0)}\left[\sum_{j\in\mathcal{V}_+(0)}\mathbb{P}\{K=k,P_j\leq t\mid\mathcal{V}_+(0),\sigma_{\mathcal{H}_1}\}\,\mathbb{P}\{J=j\mid\mathcal{V}_+(0),\sigma_{\mathcal{H}_1}\}\right]\\
=&\frac{1}{|\mathcal{H}_0|}\,\mathbb{E}_{\mathcal{V}_+(0)}\left[\sum_{j\in\mathcal{V}_+(0)}\mathbb{P}\{K=k,P_j\leq t\mid\mathcal{V}_+(0),\sigma_{\mathcal{H}_1}\}\right]\\
=&\frac{1}{|\mathcal{H}_0|}\sum_{j\in\mathcal{H}_0}\mathbb{P}\{K=k,P_j\leq t\mid\sigma_{\mathcal{H}_1}\}.
\end{align*}
Therefore
\[
\mathrm{FDR}=\mathbb{E}\left[\sum_{k=1}^m\frac{|\mathcal{H}_0|}{k}\,\mathbb{P}\{K=k,\;P_J\leq q_k^{R_+(0),\alpha}E_J\mid\sigma_{\mathcal{H}_1}\}\right].
\]

Define the sets
\[
\mathcal{C}_k(\boldsymbol{q})=\{\mathbf{p}\in\mathbb{R}_*^{m-1}:p_{(k-1)}\leq q_k,\;p_{(k)}>q_{k+1},\dots,p_{(m-1)}>q_m\},
\]
\[
\mathcal{D}_k(\boldsymbol{q})=\{\mathbf{p}\in\mathbb{R}_*^{m-1}:p_{(k)}>q_{k+1},\dots,p_{(m-1)}>q_m\},
\]
which satisfy $\mathcal{C}_k=\mathcal{D}_k\setminus\mathcal{D}_{k-1}$ with $\mathcal{D}_0=\mathbb{R}_*^{m-1}$, and each $\mathcal{D}_k$ is nondecreasing. Let 
\[
\boldsymbol{q}'=\left(q_1^{R_+(0),\alpha}\frac{1\vee R_+(0)}{r+rV_-(0)},\dots,q_m^{R_+(0),\alpha}\frac{1\vee R_+(0)}{r+rV_-(0)}\right).
\]
Conditional on $\sigma_{\mathcal{H}_1}$, the vector $\boldsymbol{q}'$ is constant. Then with sub-uniformity and the controlled randomized PRDS,
\begin{align*}
\mathrm{FDR}&=\mathbb{E}\left[\sum_{k=1}^m\frac{|\mathcal{H}_0|}{k}\,\mathbb{P}\{K=k,\;P_J\leq q_k^{R_+(0),\alpha}E_J\mid\sigma_{\mathcal{H}_1}\}\right]\\
&\leq\mathbb{E}\left[\sum_{k=1}^m\frac{|\mathcal{H}_0|}{k}\,\mathbb{P}\{\mathbf{P}^J_{(\cdot)}\in\mathcal{C}_k(\boldsymbol{q}'),\;Q_J\leq q_k^{R_+(0),\alpha}E_J\mid\sigma_{\mathcal{H}_1}\}\right]\\
&\leq\alpha\,\mathbb{E}\left[|\mathcal{H}_0|\cdot q'_1\cdot\frac{V_+(0)}{1\vee|\mathcal{H}_0|}\right]\leq\alpha.
\end{align*}
\end{proof}

\subsection{Embedding of Sub-competition Statistics}

Embedding sub-competition statistics into the randomized BH framework is more challenging than embedding competition statistics. The main reason is that sub-competition statistics lack the label-independent property. For competition statistics, the null labels are independent of both the scores and the other labels. For sub-competition statistics, the null labels may depend on the scores and the other labels. For example,
\[
\mathbf{P}\{L_j=1\mid \mathbf{W},\mathbf{L}_{-j}\} = \frac{1}{2}\frac{r}{1+r}+f(\mathbf{W},\mathbf{L}_{-j})\frac{1}{2}\frac{1}{1+r},\quad j\in\mathcal{H}_0,
\]
where $f(\mathbf{W},\mathbf{L}_{-j})\in[0,1]$ is a function of the scores and the labels of the other hypotheses. In this case, the label $L_j$ is not independent of the other labels $\mathbf{L}_{-j}$, but still satisfies the sub-competition property.

However, we can still embed the sub-competition statistics if they have the label-independent property. We give a heuristic analysis of this embedding.

Suppose $(\mathbf{W},\mathbf{L})$ are sub-competition statistics with parameter $r$ over $\mathcal{H}_0$, and there exists $\boldsymbol{r}$ such that
\[
\mathbb{P}\{L_j=1\mid \mathbf{W},\mathbf{L}_{-j}\}=r_j\mathbb{P}\{L_j=0\mid \mathbf{W},\mathbf{L}_{-j}\},\quad j\in\mathcal{H}_0,
\]
where $r_j\leq r$. Then we construct two sets of random variables,
\[
\mathbb{P}\{Z_j=1\mid \mathbf{W},\mathbf{Z}_{-j}\}=r\mathbb{P}\{Z_j=0\mid \mathbf{W},\mathbf{Z}_{-j}\},\quad j\in\mathcal{H}_0,\quad\mathbf{Z}_{\mathcal{H}_1}\overset{d}{=}\mathbf{L}_{\mathcal{H}_1},
\]
\[
\mathbb{P}\{Z'_j=1\mid \mathbf{Z}'_{-j}\}=1-\frac{r_j}{r}\frac{1+r}{1+r_j},\mathbb{P}\{Z'_j=0\mid \mathbf{Z}'_{-j}\}=\frac{r_j}{r}\frac{1+r}{1+r_j},\quad j\in\mathcal{H}_0,\quad\mathbf{Z}'_{\mathcal{H}_1}=\mathbf{0}.
\]
where $\mathbf{Z}$ and $\mathbf{Z}'$ are independent. Let $\mathbf{Z}^* = \mathbf{Z} - \mathbf{Z}\circ \mathbf{Z}'$, where $\boldsymbol{a}\circ\boldsymbol{b} = (a_1b_1, \dots, a_mb_m)$. Then we have for any $j\in\mathcal{H}_0$,
\begin{align*}
&\mathbb{P}\{Z^*_j=1\mid \mathbf{W},\mathbf{Z}^*_{-j}\}=\mathbb{P}\{Z_j=1,Z'_j=0\mid \mathbf{W},\mathbf{Z}^*_{-j}\}\\
=&\frac{\sum_{\mathbf{Z}_{-j},\mathbf{Z}'_{-j}}\mathbb{P}\{Z_j=1,Z'_j=0,\mathbf{Z}_{-j},\mathbf{Z}'_{-j}\mid \mathbf{W}\}}{\sum_{\mathbf{Z}_{-j},\mathbf{Z}'_{-j}}\mathbb{P}\{\mathbf{Z}_{-j},\mathbf{Z}'_{-j}\mid \mathbf{W}\}}\\
=&\frac{\sum_{\mathbf{Z}_{-j},\mathbf{Z}'_{-j}}\mathbb{P}\{Z_j=1,\mathbf{Z}_{-j}\mid \mathbf{W}\}\mathbb{P}\{Z'_j=0,\mathbf{Z}'_{-j}\}}{\sum_{\mathbf{Z}_{-j},\mathbf{Z}'_{-j}}\mathbb{P}\{\mathbf{Z}_{-j}\mid \mathbf{W}\}\mathbb{P}\{\mathbf{Z}'_{-j}\}}\\
=&\frac{r}{1+r}\cdot\frac{r_j}{r}\frac{1+r}{1+r_j}=\frac{r_j}{1+r_j},
\end{align*}
which implies that $(\mathbf{W},\mathbf{Z}^*)\overset{d}{=}(\mathbf{W},\mathbf{L})$. We establish the following lemma.
\begin{Lemma}
\label{slem:fdr_eq}
If $(\mathbf{W},\mathbf{L})\overset{d}{=}(\mathbf{W}',\mathbf{L}')$, let $\mathcal{R}_{\alpha}$ be competition procedure for $\mathcal{H}_0$, then we have
\[
\mathbb{E}\left[\frac{|\mathcal{H}_0\cap\mathcal{R}_{\alpha}(\mathbf{W},\mathbf{L})|}{1\vee|\mathcal{R}_{\alpha}(\mathbf{W},\mathbf{L})|}\right]=\mathbb{E}\left[\frac{|\mathcal{H}_0\cap\mathcal{R}_{\alpha}(\mathbf{W}',\mathbf{L}')|}{1\vee|\mathcal{R}_{\alpha}(\mathbf{W}',\mathbf{L}')|}\right].
\]
\end{Lemma}
This lemma is straightforward but useful, since it allows us to consider $\mathbf{Z}$ and $\mathbf{Z}'$ instead of $\mathbf{L}$. Similarly, we define $R_+^Z,R_+',R_+^*$ and $V_+^Z,V_+',V_+^*$, and $R_-^Z,R_-',R_-^*$ and $V_-^Z,V_-',V_-^*$. Construct
\[
P_j=\frac{1+R_-^*(W_j)}{1+V_-^Z(0)},\quad Q_j=\frac{1+V_-^Z(W_j)}{1+V_-^Z(0)},\quad E_j=\frac{1\vee R_+^Z(0)}{r+rV_-^Z(0)},\quad j\in\mathcal{R}_+^*(0),
\]
and 
\[
P_j=Q_j=+\infty,\quad E_j=0,\quad j\in\mathcal{R}_-^*(0).
\]
Notice that
\[
r\frac{1+R^*_-(W_j)}{1\vee R^*_+(W_j)}\leq \alpha \quad\text{and}\quad Z^*_j=1\iff\frac{P_j}{E_j}\leq q^{R^Z_+(0),\alpha}_{R^*_+(W_j)}=q^{R^*_+(0),\alpha}_{R^*_+(W_j)}\frac{R^*(0)}{R^Z(0)}.
\]
For any $j\in\mathcal{R}_+^*(0)$,
\[
P_j=\frac{1+R_-^*(W_j)}{1+V_-^Z(0)}\geq\frac{1+R_-^Z(W_j)}{1+V_-^Z(0)}\geq Q_j.
\]
Then $\mathbf{Q}$ is randomized BH-valid, and we can construct a sigma-algebra under which $\mathbf{P}$ is determined by $\mathbf{Q}$. Then with the same analysis as in the proof of Theorem~\ref{thm:embed_cp}, we can show that the FDR of $\mathcal{R}_{\alpha}(\mathbf{W},\mathbf{Z}^*)$ is controlled at level $\alpha$, and by Lemma~\ref{slem:fdr_eq}, the FDR of $\mathcal{R}_{\alpha}(\mathbf{W},\mathbf{L})$ is also controlled at level $\alpha$. However, we do not give a rigorous proof for this claim, and we leave it as a heuristic conjecture.

\section{Analysis of Compound p-Values under the Randomized BH Framework}
\label{app:compound}

\subsection{Violation of PRDS by compound p‑values}

We consider the example of independent compound p-values from Barber et al. Note that their example inherently includes a $\pi_0$ correction, and we retain it as a weight without adjustment. Let $k = \frac{1}{2\alpha}$ which is much lower than $m$, and define the set of nulls as $\mathcal{H}_0 = \{1, \ldots, m - 3k + 2\} \subseteq [m]=\mathcal{H}$. Let $\mathbf{P} = (P_1, \ldots, P_m)$ have the following distribution:

\begin{itemize}
    \item The distribution of the null $P_i$'s is given by
    \[
    P_1 \sim \operatorname{Unif}\left\{\frac{1.5}{m}, 1\right\}, \quad 
    P_2 = \frac{1}{m}, \quad 
    P_3 = \dots = P_{m-3k+2} = 1.
    \]
    \item The non-null $P_i$'s are deterministic, with values
    \[
    P_{m-3k+3} = \dots = P_{m-k+1} = \frac{1}{m}, \quad 
    P_{m-k+2} = \dots = P_m = \frac{1.5}{m}.
    \]
\end{itemize}

Because the $p_i$'s are mutually independent by definition. To see that this construction satisfies the definition of compound p-values, it suffices to observe that
\[
\sum_{i \in \mathcal{H}_0} \mathbb{P}\left\{P_i \leq \frac{1}{m}\right\} = \mathbb{P}\left\{P_2 \leq \frac{1}{m}\right\} = 1,
\]
and
\[
\sum_{i \in \mathcal{H}_0} \mathbb{P}\left\{P_i \leq \frac{1.5}{m}\right\} = \mathbb{P}\left\{P_1 \leq \frac{1.5}{m}\right\} + \mathbb{P}\left\{P_2 \leq \frac{1.5}{m}\right\} = \frac{1}{2} + 1 = 1.5.
\]
In this example, only the p-value $P_1$ is random. Clearly, when $P_1 = 1.5/m$, we have $\mathcal{R}_{\alpha}(\mathbf{P}) = \{1, 2\} \cup \mathcal{H}_1$, and when $P_1 = 1$, we have $\mathcal{R}_{\alpha}(\mathbf{P}) = \{2\} \cup \{m-3k+3, \cdots, m-k+1\}$. Therefore, FDR control is lost and $\mathrm{FDR} \geq 7\alpha/6$. This is because the randomized $\mathrm{PRDS}_{\mathcal{H}_0}$ condition is not satisfied. To see this, consider the nondecreasing set $C=\{\boldsymbol{p}\in\mathbb{R}_*^{m-1}:p_{(3k-1)}\geq 2/m\}$ and two values of $t$. Specifically,
\begin{align*}
    &\mathbb{P}\left\{\mathbf{P}^J_{(\cdot)}\in C\mid P_J\leq\frac{1}{m}\right\}\\
    =&\sum_{j\in\mathcal{H}_0}\mathbb{P}\left\{\mathbf{P}^j_{(\cdot)}\in C,J=j\mid P_J\leq\frac{1}{m}\right\}\\
    =&\sum_{j\in\mathcal{H}_0}\mathbb{P}\left\{\mathbf{P}^j_{(\cdot)}\in C\mid J=j\right\}\mathbb{P}\left\{J=j\mid P_J\leq\frac{1}{m}\right\}\\
    =&\mathbb{P}\left\{P_1\geq \frac{2}{m}\mid J=2\right\}=\frac{1}{2}
\end{align*}
while
\begin{align*}
    &\mathbb{P}\left\{\mathbf{P}^J_{(\cdot)}\in C\mid P_J\leq\frac{1.5}{m}\right\}\\
    =&\sum_{j\in\mathcal{H}_0}\mathbb{P}\left\{\mathbf{P}^j_{(\cdot)}\in C,J=j\mid P_J\leq\frac{1.5}{m}\right\}\\
    =&\sum_{j\in\mathcal{H}_0}\mathbb{P}\left\{\mathbf{P}^j_{(\cdot)}\in C\mid J=j\right\}\mathbb{P}\left\{J=j\mid P_J\leq\frac{1.5}{m}\right\}\\
    =&\frac{1}{3}\mathbb{P}\left\{\mathbf{P}^1_{(\cdot)}\in C\mid J=1\right\}+\frac{2}{3}\mathbb{P}\left\{P_1\geq\frac{2}{m}\mid J=2\right\}\\
    =&\frac{1}{3}\cdot0+\frac{2}{3}\cdot\frac{1}{2}=\frac{1}{3}<\frac{1}{2}.
\end{align*}
This example demonstrates that independence, without the guarantee of balance, does not imply the randomized $\mathrm{PRDS}_{\mathcal{H}_0}$. The key distinction between compound p-values (or randomized p-variables) and ordinary p-values lies precisely in this balance property. More generally, we have the following analysis.

Suppose $\mathbf{P}\in\mathbb{R}_*^m$ are independent randomized p-variables with respect to $\mathcal{H}_0$. Define
\[
\mathcal{C}_k=\left\{\boldsymbol{p}\in\mathbb{R}_*^{m-1}:p_{(k)}>q^{m,\alpha}_k,\cdots,p_{(m-1)}>q^{m,\alpha}_k\right\},
\]
with $p_{(0)}=0$ and $\mathcal{C}_0=\emptyset$, and let $\mathcal{D}_k=\mathcal{C}_k\setminus\mathcal{C}_{k-1}$. Then the BH procedure $\mathcal{R}_{\alpha}(\mathbf{P})$ satisfies
\begin{align*}
    \mathrm{FDR}\leq&\alpha\frac{m_0}{m}\sum_{k=1}^m\mathbb{P}\left\{|\mathcal{R}|=k\mid P_J\leq q^{m,\alpha}_k\right\}=\alpha\frac{m_0}{m}\sum_{k=1}^m\mathbb{P}\left\{\mathbf{P}^J_{(\cdot)}\in\mathcal{D}_k\mid P_J\leq q^{m,\alpha}_k\right\}\\
    =&\alpha\frac{m_0}{m}\sum_{k=1}^m\left(\mathbb{P}\left\{\mathbf{P}^J_{(\cdot)}\in\mathcal{C}_k\mid P_J\leq q^{m,\alpha}_k\right\}-\mathbb{P}\left\{\mathbf{P}^J_{(\cdot)}\in\mathcal{C}_{k-1}\mid P_J\leq q^{m,\alpha}_k\right\}\right)\\
    =&\alpha\frac{m_0}{m}+\alpha\frac{m_0}{m}\sum_{k=1}^m\left(\mathbb{P}\left\{\mathbf{P}^J_{(\cdot)}\in\mathcal{C}_{k-1}\mid P_J\leq q^{m,\alpha}_{k-1}\right\}-\mathbb{P}\left\{\mathbf{P}^J_{(\cdot)}\in\mathcal{C}_{k-1}\mid P_J\leq q^{m,\alpha}_k\right\}\right)
\end{align*}
Because of independence, we have
\begin{align*}
    \mathbb{P}\left\{\mathbf{P}^J_{(\cdot)}\in\mathcal{C}_{k-1}\mid P_J\leq q^{m,\alpha}_{k-1}\right\}=&\sum_{j\in\mathcal{H}_0}\mathbb{P}\left\{\mathbf{P}^J_{(\cdot)}\in\mathcal{C}_{k-1},J=j\mid P_J\leq q^{m,\alpha}_{k-1}\right\}\\
    =&\sum_{j\in\mathcal{H}_0}\mathbb{P}\left\{\mathbf{P}^j_{(\cdot)}\in\mathcal{C}_{k-1}\right\}\mathbb{P}\left\{J=j\mid P_J\leq q^{m,\alpha}_{k-1}\right\}
\end{align*}
and
\begin{align*}
    \mathbb{P}\left\{\mathbf{P}^J_{(\cdot)}\in\mathcal{C}_{k-1}\mid P_J\leq q^{m,\alpha}_{k}\right\}=&\sum_{j\in\mathcal{H}_0}\mathbb{P}\left\{\mathbf{P}^J_{(\cdot)}\in\mathcal{C}_{k-1},J=j\mid P_J\leq q^{m,\alpha}_{k}\right\}\\
    =&\sum_{j\in\mathcal{H}_0}\mathbb{P}\left\{\mathbf{P}^j_{(\cdot)}\in\mathcal{C}_{k-1}\right\}\mathbb{P}\left\{J=j\mid P_J\leq q^{m,\alpha}_{k}\right\}
\end{align*}
Let
\[
A_{j,k}=\mathbb{P}\left\{\mathbf{P}^j_{(\cdot)}\in\mathcal{C}_{k}\right\},\quad B_{j,k}=\mathbb{P}\left\{J=j\mid P_J\leq q^{m,\alpha}_{k}\right\},
\]
then we have
\begin{align*}
    &\sum_{k=1}^m\left(\mathbb{P}\left\{\mathbf{P}^J_{(\cdot)}\in\mathcal{C}_{k-1}\mid P_J\leq q^{m,\alpha}_{k-1}\right\}-\mathbb{P}\left\{\mathbf{P}^J_{(\cdot)}\in\mathcal{C}_{k-1}\mid P_J\leq q^{m,\alpha}_k\right\}\right)\\
    =&\sum_{k=1}^m\sum_{j\in\mathcal{H}_0}\left(A_{j,k-1}B_{j,k-1}-A_{j,k-1}B_{j,k}\right)\\
    =&\sum_{k=1}^m\sum_{j\in\mathcal{H}_0}(A_{j,k}-A_{j,k-1})B_{j,k}-A_{j,m-1}B_{j,m}
\end{align*}
which gives a computable upper bound expressed as the solution to a high-dimensional optimization problem, although the computation may be challenging.

\subsection{Negative dependence and compound p-values}

\begin{proof}[Proof of Theorem~\ref{thm:nd_compound}]

Construct $\mathbf{Q}\in\mathbb{R}_*^m$ with $Q_i=P_i$ for $i\in\mathcal{H}_1=\{m_0+1,\dots,m\}$ and $Q_i=P_{J_i}$ for $i\in\mathcal{H}_0=[m_0]$, where $\mathbf{J}$ is an independent random uniform permutation in $[m_0]$. If $\mathbf{Q}_{\mathcal{H}_0}$ is weakly negatively dependent in the sense that
\[
\mathbb{P}\left(\cap_{k\in A}\{Q_k\leq x\}\right)\leq\prod_{k\in A}\mathbb{P}\{Q_k\leq x\}
\]
for any $A\subseteq\mathcal{H}_0$ and $x\in[0,1]$, then the FDR-Linking theorem gives
\[
\mathrm{FDR}\leq\alpha+\alpha\int_{\alpha}^1\frac{\mathrm{FDR}_0(x)}{x^2}\mathrm{d}x,
\]
where $\mathrm{FDR}_0(x)$ is the FDR of the BH procedure when all hypotheses are null and the target level is $x$, that is
\[
\mathrm{FDR}_0(x)=\mathbb{P}\{S_m(\mathbf{Q})\leq x\}\leq x+\sum_{k=2}^m\binom{m}{k}\left(\frac{xk}{m}\right)^k\leq x+2x^2+\frac{9}{2}x^3+\sum_{k=4}^{\infty}\frac{(\mathrm{e}x)^k}{\sqrt{2\pi k}}
\]
with $S_m(\boldsymbol{q})=\wedge_{k=1}^m mq_{(k)}/k$. Hence we need only verify that $\mathbf{Q}$ has the required weak negative dependence property under the given conditions.

Consider any two disjoint subsets $A,B\subseteq\mathcal{H}_0$ and non-decreasing functions $f,g$. By the law of total covariance,
\begin{align*}
\mathrm{Cov}(f(\mathbf{Q}_A),g(\mathbf{Q}_B))&=\mathbb{E}_{\mathbf{P}}[\mathrm{Cov}(f(\mathbf{Q}_A),g(\mathbf{Q}_B)\mid \mathbf{P})]\\
&\qquad+\mathrm{Cov}\left(\mathbb{E}_{\mathbf{P}}[f(\mathbf{Q}_A)\mid \mathbf{P}],\mathbb{E}_{\mathbf{P}}[g(\mathbf{Q}_B)\mid \mathbf{P}]\right).
\end{align*}
For the first term, the conditional covariance given $\mathbf{P}$ is non-positive because the permutation $\mathbf{J}$ induces negative dependence among the permuted null variables. Hence
\[
\mathbb{E}_{\mathbf{P}}[\mathrm{Cov}(f(\mathbf{Q}_A),g(\mathbf{Q}_B)\mid \mathbf{P})]\leq 0.
\]
For the second term, set $F(\mathbf{P})=\mathbb{E}[f(\mathbf{Q}_A)\mid \mathbf{P}]$ and $G(\mathbf{P})=\mathbb{E}[g(\mathbf{Q}_B)\mid \mathbf{P}]$. Both $F$ and $G$ are coordinatewise non-decreasing functions of $\mathbf{P}$. Under the assumption that the original p-values $\mathbf{P}$ are negatively associated,
\[
\mathrm{Cov}\left(\mathbb{E}_{\mathbf{P}}[f(\mathbf{Q}_A)\mid \mathbf{P}],\mathbb{E}_{\mathbf{P}}[g(\mathbf{Q}_B)\mid \mathbf{P}]\right)=\mathrm{Cov}\left(F(\mathbf{P}),G(\mathbf{P})\right)\leq 0.
\]
Combining the two bounds yields $\mathrm{Cov}(f(\mathbf{Q}_A),g(\mathbf{Q}_B))\leq0$, which establishes that $\mathbf{Q}$ is weakly negatively dependent.
\end{proof}

\section{Analysis of Integrated Tests under the Randomized BH Framework}

\subsection{Proofs for Integrated Tests}

\begin{proof}[Proof of Theorem~\ref{thm:int_rp_rp}]

By definition and Lemma~\ref{slem:equiv_rejection}, we have
\[
K=\sup\left\{k:\sum_{j_1\in\mathcal{H}^1}\mathbf{1}\{P_{j_1} \leq q^{m_1+m_2,\alpha}_k\}+\sum_{j_2\in\mathcal{H}^2}\mathbf{1}\{Q_{j_2} \leq q^{m_1+m_2,\alpha}_k\}\geq k\right\}
\]
and $K=|\mathcal{R}_{\alpha}((\mathbf{P},\mathbf{Q}))|$. Then
\begin{align*}
    \mathrm{FDR}&=\mathbb{E}\left[\frac{\sum_{j_1\in\mathcal{H}^1_0}\mathbf{1}\{P_{j_1} \leq q^{m_1+m_2,\alpha}_K\}+\sum_{j_2\in\mathcal{H}^2_0}\mathbf{1}\{Q_{j_2} \leq q^{m_1+m_2,\alpha}_K\}}{1\vee\left(\sum_{j_1\in\mathcal{H}^1}\mathbf{1}\{P_{j_1} \leq q^{m_1+m_2,\alpha}_K\}+\sum_{j_2\in\mathcal{H}^2}\mathbf{1}\{Q_{j_2} \leq q^{m_1+m_2,\alpha}_K\}\right)}\right]\\
    &=\mathbb{E}\left[\frac{\sum_{j_1\in\mathcal{H}^1_0}\mathbf{1}\{P_{j_1} \leq q^{m_1+m_2,\alpha}_K\}}{1\vee K}+\frac{\sum_{j_2\in\mathcal{H}^2_0}\mathbf{1}\{Q_{j_2} \leq q^{m_1+m_2,\alpha}_K\}}{1\vee K}\right]\\
    &=\sum_{k=1}^{m_1+m_2}\frac{1}{k}\left(\sum_{j_1\in\mathcal{H}_0^1}\mathbb{P}\left\{P_{j_1}\leq q^{m_1+m_2,\alpha}_k,K=k\right\}+\sum_{j_2\in\mathcal{H}_0^2}\mathbb{P}\left\{Q_{j_2}\leq q^{m_1+m_2,\alpha}_k,K=k\right\}\right)
\end{align*}
Let $J_1$ and $J_2$ be uniformly random selections from $\mathcal{H}_0^1$ and $\mathcal{H}_0^2$ respectively. For any set $D\in\mathbb{R}_*^{m_1+m_2-1}$ and $t$,
\begin{align*}
    \mathbb{P}\left\{(\mathbf{P}^{J_1},\mathbf{Q})_{(\cdot)}\in D\mid P_{J_1}\leq t,\mathbf{Q}\right\}&=\frac{1}{1\vee|\mathcal{H}_0^1|}\sum_{j_1\in\mathcal{H}_0^1}\mathbb{P}\left\{(\mathbf{P}^{j_1},\mathbf{Q})_{(\cdot)}\in D\mid P_{j_1}\leq t,\mathbf{Q}\right\},\\
    \mathbb{P}\left\{(\mathbf{P},\mathbf{Q}^{J_2})_{(\cdot)}\in D\mid Q_{J_2}\leq t,\mathbf{P}\right\}&=\frac{1}{1\vee|\mathcal{H}_0^2|}\sum_{j_2\in\mathcal{H}_0^2}\mathbb{P}\left\{(\mathbf{P},\mathbf{Q}^{j_2})_{(\cdot)}\in D\mid Q_{j_2}\leq t,\mathbf{P}\right\},
\end{align*}
where $(\mathbf{P}^{j_1},\mathbf{Q})_{(\cdot)}$ and $(\mathbf{P},\mathbf{Q}^{j_2})_{(\cdot)}$ denote the order statistics of the combined vectors obtained by removing $P_{j_1}$ from $\mathbf{P}$ or $Q_{j_2}$ from $\mathbf{Q}$ respectively. Define
\[
\mathcal{C}_k=\left\{\boldsymbol{u}\in\mathbb{R}_*^{m_1+m_2-1}:u_{(k)}>q^{m_1+m_2,\alpha}_{k+1},\cdots,u_{(m_1+m_2-1)}>q^{m_1+m_2,\alpha}_{m_1+m_2}\right\}
\]
with $u_{(0)}=0$ and $\mathcal{C}_{0}=\emptyset$, $\mathcal{C}_{m_1+m_2}=\mathbb{R}_*^{m_1+m_2-1}$, and let $\mathcal{D}_k=\mathcal{C}_k\setminus\mathcal{C}_{k-1}$. Then by the independence of $\mathbf{P}$ and $\mathbf{Q}$,
\[
\mathbb{P}\left\{P_{j_1}\leq q^{m_1+m_2,\alpha}_k,K=k\right\}=\mathbb{E}_{\mathbf{Q}}\mathbb{P}\left\{P_{j_1}\leq q^{m_1+m_2,\alpha}_k,(\mathbf{P}^{j_1},\mathbf{Q})_{(\cdot)}\in\mathcal{D}_k\mid\mathbf{Q}\right\},
\]
\[
\mathbb{P}\left\{Q_{j_2}\leq q^{m_1+m_2,\alpha}_k,K=k\right\}=\mathbb{E}_{\mathbf{P}}\mathbb{P}\left\{Q_{j_2}\leq q^{m_1+m_2,\alpha}_k,(\mathbf{P},\mathbf{Q}^{j_2})_{(\cdot)}\in\mathcal{D}_k\mid\mathbf{P}\right\}.
\]
Now set
\[
\mathcal{C}^1_k(\boldsymbol{q})=\left\{\boldsymbol{p}\in\mathbb{R}_*^{m_1-1}:(\boldsymbol{p},\boldsymbol{q})\in\mathcal{C}_k\right\},\quad\mathcal{C}^2_k(\boldsymbol{p})=\left\{\boldsymbol{q}\in\mathbb{R}_*^{m_2-1}:(\boldsymbol{p},\boldsymbol{q})\in\mathcal{C}_k\right\},
\]
\[
\mathcal{D}^1_k(\boldsymbol{q})=\left\{\boldsymbol{p}\in\mathbb{R}_*^{m_1-1}:(\boldsymbol{p},\boldsymbol{q})\in\mathcal{D}_k\right\},\quad\mathcal{D}^2_k(\boldsymbol{p})=\left\{\boldsymbol{q}\in\mathbb{R}_*^{m_2-1}:(\boldsymbol{p},\boldsymbol{q})\in\mathcal{D}_k\right\}.
\]
For any given $\boldsymbol{p},\boldsymbol{q}$ and any $k\in[m_1+m_2]$, we have $\mathcal{D}^1_k(\boldsymbol{q})=\mathcal{C}^1_k(\boldsymbol{q})\setminus\mathcal{C}^1_{k-1}(\boldsymbol{q})$ and $\mathcal{D}^2_k(\boldsymbol{p})=\mathcal{C}^2_k(\boldsymbol{p})\setminus\mathcal{C}^2_{k-1}(\boldsymbol{p})$. Moreover $\mathcal{C}^1_k(\boldsymbol{q})$ and $\mathcal{C}^2_{k}(\boldsymbol{p})$ are non-decreasing sets. For brevity, set
\[
a_{n_1,n_2}(\mathbf{Q})=\mathbb{P}\bigl\{P_{J_1}\leq q^{m_1+m_2,\alpha}_{n_1},
    \mathbf{P}^{J_1}_{(\cdot)}\in\mathcal{C}^1_{n_2}(\mathbf{Q})\mid\mathbf{Q}\bigr\},
\]
\[
b_{n_1,n_2}(\mathbf{P})=\mathbb{P}\bigl\{Q_{J_2}\leq q^{m_1+m_2,\alpha}_{n_1},
    \mathbf{Q}^{J_2}_{(\cdot)}\in\mathcal{C}^2_{n_2}(\mathbf{P})\mid\mathbf{P}\bigr\},
\]
with $a_{n,0}(\mathbf{Q})=b_{n,0}(\mathbf{P})=0$. Then
\begin{align*}
    \mathrm{FDR} &= \sum_{k=1}^{m_1+m_2}\frac{1}{k}
        \Bigl(\sum_{j_1\in\mathcal{H}_0^1}
            \mathbb{P}\bigl\{P_{j_1}\leq q^{m_1+m_2,\alpha}_k,\;K=k\bigr\}
        + \sum_{j_2\in\mathcal{H}_0^2}
            \mathbb{P}\bigl\{Q_{j_2}\leq q^{m_1+m_2,\alpha}_k,\;K=k\bigr\}\Bigr) \\[4pt]
    &= \sum_{k=1}^{m_1+m_2}\frac{1}{k}
        \Bigl(|\mathcal{H}_0^1|\,
            \mathbb{E}_{\mathbf{Q}}
            \mathbb{P}\bigl\{P_{J_1}\leq q^{m_1+m_2,\alpha}_k,
                \mathbf{P}^{J_1}_{(\cdot)}\in\mathcal{D}^1_k(\mathbf{Q})\mid\mathbf{Q}\bigr\}\\
        &\qquad + |\mathcal{H}_0^2|\,
            \mathbb{E}_{\mathbf{P}}
            \mathbb{P}\bigl\{Q_{J_2}\leq q^{m_1+m_2,\alpha}_k,
                \mathbf{Q}^{J_2}_{(\cdot)}\in\mathcal{D}^2_k(\mathbf{P})\mid\mathbf{P}\bigr\}\Bigr) \\[4pt]
    &= \mathbb{E}_{\mathbf{Q}}\Bigg[
        \sum_{k=1}^{m_1+m_2}\frac{|\mathcal{H}_0^1|}{k}
        \bigl(a_{k,k}(\mathbf{Q})-a_{k,k-1}(\mathbf{Q})\bigr)
    \Bigg]
    + \mathbb{E}_{\mathbf{P}}\Bigg[
        \sum_{k=1}^{m_1+m_2}\frac{|\mathcal{H}_0^2|}{k}
        \bigl(b_{k,k}(\mathbf{P})-b_{k,k-1}(\mathbf{P})\bigr)
    \Bigg] \\[4pt]
    &\leq \alpha\frac{|\mathcal{H}_0^1|+|\mathcal{H}_0^2|}{m_1+m_2}.
\end{align*}
\end{proof}

We present only the proof of the second part of Theorem~\ref{thm:fdr_int} (Algorithm~\ref{algo:int_p_cp}) since the first part follows similarly by the same approach.

\begin{proof}[Proof of Theorem~\ref{thm:fdr_int}]

Let
\[
Y_j=\frac{1+\sum_{i=1}^{m_2}\mathbf{1}\{W_i\geq W_j,L_i=0\}}{1+\sum_{i\in\mathcal{H}^2_0}\mathbf{1}\{L_i=0\}},\qquad
Z_j=\frac{1+\sum_{i\in\mathcal{H}^2_0}\mathbf{1}\{W_i\geq W_j,L_i=0\}}{1+\sum_{i\in\mathcal{H}^2_0}\mathbf{1}\{L_i=0\}},\\
\]
\[
E_j=\frac{m_2}{r+r\sum_{i\in\mathcal{H}^2_0}\mathbf{1}\{L_i=0\}},\qquad \forall j\in\{j:L_j=1\},
\]
and
\[
Y_j=+\infty,\quad Z_j=+\infty,\quad E_j=0,\qquad \forall j\in\{j:L_j=0\}.
\]
For any $k$, we have the equivalence such that
\[
X_j\leq q_k^{m_1+m_2,\alpha},L_j=1\Leftrightarrow Y_j\leq q_k^{m_1+m_2,\alpha}E_j.
\]
Then
\begin{align*}
    \mathrm{FDR} &= \mathbb{E}\left[\frac{|\mathcal{R}_1\cap\mathcal{H}_0^1|+|\mathcal{R}_2\cap\mathcal{H}_0^2|}{1\vee\left(|\mathcal{R}_1|+|\mathcal{R}_2|\right)}\right] \\
    &= \mathbb{E}\Bigg[\mathbb{E}\left[\frac{\sum_{j\in\mathcal{H}^1_0}\mathbf{1}\{P_j\leq q^{m_1+m_2,\alpha}_K\}}{1\vee K}\mid \mathbf{W},\mathbf{L}\right]+\mathbb{E}\left[\frac{\sum_{j\in\mathcal{H}^2_0}\mathbf{1}\{X_j\leq q^{m_1+m_2,\alpha}_K,L_j=1\}}{1\vee K}\mid\mathbf{P}\right]\Bigg].
\end{align*}

We consider the two conditional expectations separately. Since $\sigma\{\mathbf{X},\mathbf{L}\}\supseteq\sigma\{\mathbf{W},\mathbf{L}\}$, we may treat the p-value $X_j$ for any $j$ with $L_j=0$ as $+\infty$. From the proof of Theorem~\ref{thm:int_rp_rp}, it follows that
\[
\mathbb{E}\left[\frac{\sum_{j\in\mathcal{H}^1_0}\mathbf{1}\{P_j\leq q^{m_1+m_2,\alpha}_K\}}{1\vee K}\mid \mathbf{W},\mathbf{L}\right]\leq\alpha\frac{|\mathcal{H}_0^1|}{m_1+m_2},
\]
where the bound does not depend on $\mathbf{W}$ or $\mathbf{L}$.

For the second conditional expectation, we similarly treat $Y_j$ and $Z_j$ for indices $j$ with $L_j=0$ as infinity. Consider the $\sigma$-algebra $\sigma_{\mathcal{H}_1^2}=\sigma\{V_+(0),V_-(0),\mathbf{W},\mathbf{L}_{\mathcal{H}_1^2}\}$. Since $\mathbf{P}$ and $(\mathbf{W},\mathbf{L})$ are independent, we have conditional controlled randomized $\mathrm{PRDS}_{\mathcal{H}_0^2}$ by $\mathbf{Z}$ that for any nondecreasing set $C\subseteq\mathbb{R}^{m_2-1}$, the conditional probability $\mathbb{P}\{\mathbf{Y}^J_{(\cdot)}\in C\mid Z_J\leq t,\sigma_{\mathcal{H}_1^2},\mathbf{P}\}$ is nondecreasing in $t$. By Theorem~\ref{thm:embed_cp}, we need only verify that, given $Z_J\leq q^{m_1+m_2,\alpha}_k$, $\sigma_{\mathcal{H}_1^2}$, and $\mathbf{P}$, the event $\{K=k\}$ is a nondecreasing set with respect to $\mathbf{Y}^J_{(\cdot)}$. The proof of Theorem~\ref{thm:int_rp_rp} shows that this condition holds as well. Hence
\[
\mathbb{E}\left[\frac{\sum_{j\in\mathcal{H}^2_0}\mathbf{1}\{Y_j\leq q^{m_1+m_2,\alpha}_KE_j\}}{1\vee K}\mid\mathbf{P},\sigma_{\mathcal{H}_1^2}\right]\leq\alpha\frac{m_2}{m_1+m_2}\frac{V_+(0)}{r+rV_-(0)}.
\]
Combining the two bounds gives
\[
\mathrm{FDR}\leq\alpha\,\mathbb{E}\left[\frac{|\mathcal{H}_0^1|}{m_1+m_2}+\frac{m_2}{m_1+m_2}\frac{V_+(0)}{r+rV_-(0)}\right]\leq\alpha.
\]
\end{proof}

\begin{proof}[Proof of Theorem~\ref{thm:cp_cp_any_dep}]

Rewrite the FDR as
\[
\mathrm{FDR} =
\mathbb{E}\left[ \sum_{g=1}^2 \frac{1 + \sum_{j\in\mathcal{R}^g_-(0)} \mathbf{1}\bigl\{ \frac{1+R^g_-(W_j)}{m_g c(r_g)} \leq q^{m_1+m_2}_K \bigr\}}{K}
\cdot \frac{\sum_{j\in\mathcal{H}^g_0} \mathbf{1}\{ X^g_j \leq q^{m_1+m_2}_K \}}{1 + \sum_{j\in\mathcal{R}^g_-(0)} \mathbf{1}\bigl\{ \frac{1+R^g_-(W_j)}{m_g c(r_g)} \leq q^{m_1+m_2}_K \bigr\}} \right].
\]

Define the minimal negative statistic
\[
W^g_{\mathrm{negmin}} = \min\Bigl\{ W^g_j : j\in\mathcal{R}^g_-(0),\; \frac{1+R^g_-(W^g_j)}{m_g c(r_g)} \leq q^{m_1+m_2}_K \Bigr\}.
\]
For any $W^g_j < W^g_{\mathrm{negmin}}$ with $j\in\mathcal{R}^g_-(0)$,
\[
\frac{1+R^g_-(W^g_j)}{m_g c(r_g)} \ge \frac{2+R^g_-(W^g_{\mathrm{negmin}})}{m_g c(r_g)} > q^{m_1+m_2}_K.
\]
Set
\[
W^g_{\mathrm{negmin}+1} = \max\{ W^g_j : j\in\mathcal{R}^g_-(0),\; W^g_j < W^g_{\mathrm{negmin}} \}.
\]
Then
\[
X^g_j \leq q^{m_1+m_2}_K \quad\Longleftrightarrow\quad W^g_j > W^g_{\mathrm{negmin}+1}\ \text{and}\ L^g_j=1,
\]
and consequently
\[
\frac{1 + \sum_{j\in\mathcal{R}^g_-(0)} \mathbf{1}\bigl\{ \frac{1+R^g_-(W_j)}{m_g c(r_g)} \leq q^{m_1+m_2}_K \bigr\}}{K}
= \frac{1+R^g_-(W^g_{\mathrm{negmin}})}{K}
= \frac{m_g c(r_g)}{K} \sup_{j\in\mathcal{H}^g_0} \{ X^g_j : X^g_j \leq q^{m_1+m_2}_K \}.
\]

Therefore,
\begin{align*}
\mathrm{FDR}
&\leq \alpha \sum_{g=1}^2 \frac{m_g c(r_g)}{m_1+m_2}\;
\mathbb{E}\left[ \frac{\sum_{j\in\mathcal{H}^g_0} \mathbf{1}\{ X^g_j \leq q^{m_1+m_2}_K \}}{1 + \sum_{j\in\mathcal{R}^g_-(0)} \mathbf{1}\bigl\{ \frac{1+R^g_-(W_j)}{m_g c(r_g)} \leq q^{m_1+m_2}_K \bigr\}} \right] \\[6pt]
&= \alpha \sum_{g=1}^2 \frac{m_g c(r_g)}{m_1+m_2}\;
\mathbb{E}\left[ \frac{\sum_{j\in\mathcal{H}^g_0} \mathbf{1}\{ W^g_j < W^g_{\mathrm{negmin}+1},\; L^g_j=1 \}}{1 + \sum_{j\in\mathcal{H}^g} \mathbf{1}\{ W^g_j < W^g_{\mathrm{negmin}+1},\; L^g_j=0 \}} \right],
\end{align*}
where $W^g_{\mathrm{negmin}+1}$ depends on $K$, and $K$ depends on both groups, so direct computation is infeasible. By the properties of competition statistics, we may replace $W^g_{\mathrm{negmin}+1}$ with an arbitrary threshold $t$ and take the supremum over $t$ to obtain a bound independent of the inter-group dependence structure. This motivates the definition
\[
c(r_g)\cdot\mathbb{E}\left[ \sup_{t\in\mathbb{R}} \frac{\sum_{j\in\mathcal{H}^g_0} \mathbf{1}\{ W^g_j < t,\; L^g_j=1 \}}{1 + \sum_{j\in\mathcal{H}^g} \mathbf{1}\{ W^g_j < t,\; L^g_j=0 \}} \right]\leq1.
\]
which is independent of the inter-group dependence structure. Finally,
\begin{align*}
&\mathbb{E}\left[ \sup_{t\in\mathbb{R}} \frac{\sum_{j\in\mathcal{H}^g_0} \mathbf{1}\{ W^g_j < t,\; L^g_j=1 \}}{1 + \sum_{j\in\mathcal{H}^g} \mathbf{1}\{ W^g_j < t,\; L^g_j=0 \}} \right]
\leq \mathbb{E}\left[ \sup_{t\in\mathbb{R}} \frac{\sum_{j\in\mathcal{H}^g_0} \mathbf{1}\{ W^g_j < t,\; L^g_j=1 \}}{1 + \sum_{j\in\mathcal{H}^g_0} \mathbf{1}\{ W^g_j < t,\; L^g_j=0 \}} \right] \\[6pt]
&= \mathbb{E}\left[ \sup_{k\in\{0\}\cup[|\mathcal{H}^g_0|]} \frac{S_k}{1+k-S_k} \right]
\leq \mathbb{E}\left[ \sup_{k\in\mathbb{N}} \frac{S_k}{1+k-S_k} \right],
\end{align*}
where $S_k$ follows a binomial distribution with parameters $k$ and $r_g/(1+r_g)$. The bound is independent of the statistics. To maximize the number of rejections, we should choose $c(r_g)$ as large as possible, so we take
\[
c(r) = \left( \mathbb{E}\left[ \sup_{k\in\mathbb{N}} \frac{S_k}{1+k-S_k} \right] \right)^{-1},
\]
where $S_k\sim\mathrm{Binomial}(k, r/(1+r))$. When $r=1$,
\[
\mathbb{E}\left[ \sup_{k\in\mathbb{N}} \frac{S_k}{1+k-S_k} \right] \leq 1.922.
\]
\end{proof}

\subsection{Analysis of Proposition~\ref{pro:loss_control}}

We construct an example. Without loss of generality, consider two groups of competition statistics with parameter $r_i=1$. Both groups involve $11$ hypotheses, of which the first $9$ are alternative and the last $2$ are null. Under the alternative, the label is $1$ and the score is always higher than under the null. For a target FDR level $\alpha=0.1$, the constraint inequality of the filter admits three configurations for the null labels: (a) both null hypotheses take label $1$, (b) only the higher-scoring null hypothesis takes label $1$, and (c) the higher-scoring null hypothesis takes label $0$. Because $r=1$, the corresponding probabilities are $0.25$, $0.25$, and $0.5$, and the numbers of total and false rejections are $(11,2)$, $(10,1)$, and $(0,0)$ respectively. Hence
\begin{align*}
    \mathrm{FDR}&=\mathbb{E}\left[\frac{|(\mathcal{H}_0^1\cap\mathcal{R}_{0.1}(\mathbf{W}^1,\mathbf{L}^1))\cup(\mathcal{H}_0^2\cap\mathcal{R}_{0.1}(\mathbf{W}^2,\mathbf{L}^2))|}{1\vee|\mathcal{R}_{0.1}(\mathbf{W}^1,\mathbf{L}^1)\cup\mathcal{R}_{0.1}(\mathbf{W}^2,\mathbf{L}^2)|}\right]\\
    &=\frac{1}{4}\times\frac{1}{4}\times\frac{4}{22}+\frac{1}{4}\times\frac{1}{4}\times\frac{2}{20}+2\times\frac{1}{4}\times\frac{1}{4}\times\frac{3}{21}\\
    &\qquad+2\times\frac{1}{4}\times\frac{1}{2}\times\frac{2}{11}+2\times\frac{1}{4}\times\frac{1}{2}\times\frac{1}{10}\\
    &=\frac{261}{2464}>0.1=\alpha.
\end{align*}

We now analyze the loss of FDR control in two steps.

First, we directly analyze Proposition~\ref{pro:loss_control}. Without loss of generality, consider competition statistics with parameter $r=1$ and fix $\mathbf{W},\mathbf{L}_{\mathcal{H}_1}$ to determine the ranking of scores. By interleaving null hypotheses with alternative hypotheses whose labels are $0$ and those whose labels are $1$, we can achieve
\[
\frac{1+R_-(T)}{1\vee R_+(T)} = \alpha.
\]
Consider the following example ordered by descending scores. First, there are $10$ alternative hypotheses with label $1$, followed by a loop. In each iteration, we place one alternative hypothesis with label $0$, then one null hypothesis, and finally nine alternative hypotheses with label $1$. Setting $\alpha=0.1$ satisfies the above equation. The sequence of labels is given below, where $x$ denotes a null hypothesis with undetermined label:
\[
1,1,1,1,1,1,1,1,1,1,\underbrace{0,x,1,1,1,1,1,1,1,1,1}_{\text{loop}},\cdots.
\]
If $x=1$, the procedure proceeds to the next iteration. If $x=0$, it rejects the last alternative hypothesis with label $1$ that precedes this null hypothesis, and the equality holds. By the proof of FDR control for the competition procedure, we need only consider
\[
\mathbb{E}\left[\frac{V^1_+(T^1)+V^2_+(T^2)}{1+V^1_-(T^1)+V^2_-(T^2)}\right],
\]
where $T^1,T^2$ are the thresholds from the competition procedure. Applying the flip-one method,
\begin{align*}
    &\mathbb{E}\left[\frac{V^1_+(T^1)+V^2_+(T^2)}{1+V^1_-(T^1)+V^2_-(T^2)}\right]
    =\mathbb{E}\left[\frac{\sum_{g=1}^2\sum_{i\in\mathcal{H}_0^g}\mathbf{1}\{W^g_i\geq T^g,L^g_i=1\}}{1+\sum_{h=1}^2\sum_{j\in\mathcal{H}_0^h}\mathbf{1}\{W^h_j\geq T^h,L^h_j=0\}}\right]\\
    &=\mathbb{E}\left[\sum_{g=1}^2\sum_{i\in\mathcal{H}_0^g}\mathbb{E}\left[\frac{\mathbf{1}\{W^g_i\geq T^g,L^g_i=1\}}{1+\sum_{h=1}^2\sum_{j\in\mathcal{H}_0^h}\mathbf{1}\{W^h_j\geq T^h,L^h_j=0\}}\mid \mathbf{W}^{3-g},\mathbf{L}^{3-g},\mathbf{W}^g,\mathbf{L}^g_{-i}\right]\right]\\
    &=\sum_{g=1}^2\sum_{i\in\mathcal{H}_0^g}\mathbb{E}\Bigg[\mathbb{E}\Bigg[\frac{\mathbf{1}\{W^g_i\geq T^g_i,L^g_i=1\}}{1+\sum_{j\in\mathcal{H}_0^g}\mathbf{1}\{W^g_j\geq T^g_i,L^g_j=0\}+\sum_{j\in\mathcal{H}_0^{3-g}}\mathbf{1}\{W^{3-g}_j\geq T^{3-g},L^{3-g}_j=0\}}\mid \sigma_i^g\Bigg]\Bigg]
\end{align*}
where $\sigma^g_i=\sigma\{\mathbf{W}^{3-g},\mathbf{L}^{3-g},\mathbf{W}^g,\mathbf{L}^g_{-i}\}$ and
\[
T^g_i=\inf\left\{t\in\{W^g_j:L_j=1\}:\frac{\sum_{j\neq i}\mathbf{1}\{W^g_j\geq t,L^g_j=0\}+1}{1\vee\left(\sum_{j\neq i}\mathbf{1}\{W^g_j\geq t,L^g_j=0\}+\mathbf{1}\{W^g_i\geq t\}\right)}\leq\alpha\right\}.
\]
By the definition of competition statistics,
\begin{align*}
    &\mathbb{E}\left[\frac{\mathbf{1}\{W^g_i\geq T^g,L^g_i=1\}}{1+\sum_{j\in\mathcal{H}_0^g}\mathbf{1}\{W^g_j\geq T^g,L^g_j=0\}+\sum_{j\in\mathcal{H}_0^{3-g}}\mathbf{1}\{W^{3-g}_j\geq T^{3-g},L^{3-g}_j=0\}}\right]\\
    &=\mathbb{E}\left[\frac{\mathbf{1}\{W^g_i\geq T^g_i,L^g_i=0\}}{1+\sum_{j\in\mathcal{H}_0^g\setminus\{i\}}\mathbf{1}\{W^g_j\geq T^g_i,L^g_j=0\}+\sum_{j\in\mathcal{H}_0^{3-g}}\mathbf{1}\{W^{3-g}_j\geq T^{3-g},L^{3-g}_j=0\}}\right]
\end{align*}
and by Lemma~\ref{slem:biovervariable},
\begin{align*}
    &\mathbb{E}\left[\frac{V^1_+(T^1)+V^2_+(T^2)}{1+V^1_-(T^1)+V^2_-(T^2)}\right]\\
    &=\sum_{g=1}^2\mathbb{E}\left[\frac{\sum_{j\in\mathcal{H}^g_0}\mathbf{1}\{W^g_j\geq T^g_j,L^g_j=0\}}{1\vee\left(\sum_{j\in\mathcal{H}^g_0}\mathbf{1}\{W^g_j\geq T^g_j,L^g_j=0\}+\sum_{j\in\mathcal{H}^{3-g}_0}\mathbf{1}\{W^{3-g}_j\geq T^{3-g},L^{3-g}_j=0\}\right)}\right].
\end{align*}
In this example, unless the flip involves the last null hypothesis, it always decreases the threshold and increases the number of rejections. Consequently,
\[
\sum_{g=1}^2\frac{\sum_{j\in\mathcal{H}^g_0}\mathbf{1}\{W^g_j\geq T^g_j,L^g_j=0\}}{1\vee\left(\sum_{j\in\mathcal{H}^g_0}\mathbf{1}\{W^g_j\geq T^g_j,L^g_j=0\}+\sum_{j\in\mathcal{H}^{3-g}_0}\mathbf{1}\{W^{3-g}_j\geq T^{3-g},L^{3-g}_j=0\}\right)}>1.
\]
Thus the constructed example can lead to a loss of FDR control.

Second, we use Theorem~\ref{thm:fdr_int} to analyze why Proposition~\ref{pro:loss_control} occurs, that is, why direct integration of multiple testing results fails. Without proof, we state that if the following substitutions are made to Algorithm~\ref{algo:int_p_cp},
\[
X_j\leftarrow\frac{r+r\sum_{i=1}^{m_2}\mathbf{1}\{W_i\geq W_j,L_i=0\}}{m_2}
\quad\Longrightarrow\quad
X_j\leftarrow\frac{r+r\sum_{i=1}^{m_2}\mathbf{1}\{W_i\geq W_j,L_i=0\}}{1\vee\sum_{i=1}^{m_2}\mathbf{1}\{L_i=1\}},
\]
and
\[
q^{m_1+m_2,\alpha}_k \;\Longrightarrow\; q^{m_1+R_+(0),\alpha}_k,
\]
where $R_+(0)=\sum_{i=1}^{m_2}\mathbf{1}\{L_i=1\}$, then
\[
\mathrm{FDR}\leq\alpha\,\mathbb{E}\left[\frac{|\mathcal{H}_0^1|}{m_1+R_+(0)}+\frac{R_+(0)}{m_1+R_+(0)}\frac{V_+(0)}{r+rV_-(0)}\right].
\]
Under a fixed multiple testing problem, $R_+(0)$ and $V_+(0)$ are strongly positively correlated. By the rearrangement inequality,
\[
\mathbb{E}\left[\frac{R_+(0)}{m_1+R_+(0)}\frac{V_+(0)}{r+rV_-(0)}\right]>\mathbb{E}\left[\frac{R_+(0)}{m_1+R_+(0)}\right]\mathbb{E}\left[\frac{V_+(0)}{r+rV_-(0)}\right],
\]
and when $m_2$ is sufficiently large,
\[
\mathbb{E}\left[\frac{V_+(0)}{r+rV_-(0)}\right]\to1.
\]
This analysis suggests that the loss of global FDR control when integrating multiple testing results may be understood through the rearrangement inequality. Results with higher FDP may inherently have larger numbers of rejections, consequently occupying a greater proportion in the global FDR and causing the overall FDR to exceed the target level.

In brief, consistent with both the constructed example and the principle of the rearrangement inequality, if each group of tests tends to reject more hypotheses when its local FDP is large, then the global FDR may exceed the target level.

\subsection{Integrated Test with Different Weights}

We present the following algorithms. They are almost identical to the algorithms given in the main article, except that the value $m$ for the integrated competition testing is replaced by $R_-(0)$. The details are as follows.

\begin{algorithm}[H]
    \caption{Integrated Test of Competition and Competition with $R_-(0)$}
    \SetAlgoLined
    \DontPrintSemicolon
    \SetAlgoNoEnd
    \LinesNotNumbered
    \SetKwProg{Fn}{Function}{}{}

    \textbf{Input}: $(\mathbf{W}^1, \mathbf{L}^1) \in \mathbb{R}_*^{m_1} \times \{0,1\}^{m_1}$, $(\mathbf{W}^2, \mathbf{L}^2) \in \mathbb{R}_*^{m_2} \times \{0,1\}^{m_2}$, $\alpha \in (0,1)$, $r_1,r_2 > 0$ \\
    \textbf{Output}: $\mathcal{R}_1$, $\mathcal{R}_2$

    \For{$g=1$ \KwTo $2$}{
        \For{$j=1$ \KwTo $m_g$}{
          $X^g_j \leftarrow \frac{r_g+r_g\sum_{i=1}^{m_g}\mathbf{1}\{W^g_i\geq W^g_j,L^g_i=0\}}{1\vee\sum_{i=1}^{m_g}\mathbf{1}\{L_i^g=0\}}$
        }
    }
    $K \leftarrow 0$, $R^g_-(0) \leftarrow \sum_{i=1}^{m_g}\mathbf{1}\{L_i^g=0\}$
    \For{$k=R^1_-(0)+R^2_-(0)$ \KwTo $1$}{
      \If{$\sum_{g=1}^{2}\sum_{j=1}^{m_g} \mathbf{1}\{X^g_j \leq q^{R^1_-(0)+R^2_-(0),\alpha}_k,L^g_j=1\} \geq k$}{
        $K \leftarrow k$; \textbf{break}
      }
    }
    $\mathcal{R}_g \leftarrow \{j \in [m_g] : X^g_j \leq q^{R^1_-(0)+R^2_-(0),\alpha}_K,L^g_j=1\}$, $g=1,2$ \\
    \Return $(\mathcal{R}_1, \mathcal{R}_2)$
    \label{salgo:int_cp_cp}
\end{algorithm}

\begin{algorithm}[H]
    \caption{Integrated Test of P-value and Competition with $R_-(0)$}
    \SetAlgoLined
    \DontPrintSemicolon
    \SetAlgoNoEnd
    \LinesNotNumbered
    \SetKwProg{Fn}{Function}{}{}

    \textbf{Input}: $\mathbf{P} \in \mathbb{R}_*^{m_1}$, $(\mathbf{W}, \mathbf{L}) \in \mathbb{R}_*^{m_2} \times \{0,1\}^{m_2}$, $\alpha \in (0,1)$, $r > 0$ \\
    \textbf{Output}: $\mathcal{R}_1$, $\mathcal{R}_2$

    \For{$j=1$ \KwTo $m_2$}{
          $X_j \leftarrow \frac{r+r\sum_{i=1}^{m_2}\mathbf{1}\{W_i\geq W_j,L_i=0\}}{1\vee\sum_{i=1}^{m_2}\mathbf{1}\{L_i=0\}}$
        }
    $K \leftarrow 0$, $R_-(0)\leftarrow\sum_{i=1}^{m_2}\mathbf{1}\{L_i=0\}$
    \For{$k=m_1+m_2$ \KwTo $1$}{
      \If{$\sum_{j=1}^{m_1} \mathbf{1}\{P_j \leq q^{m_1+R_-(0),\alpha}_k\} + \sum_{j=1}^{m_2} \mathbf{1}\{X_j \leq q^{m_1+R_-(0),\alpha}_k,L_j=1\} \geq k$}{
        $K \leftarrow k$; \textbf{break}
      }
    }
    $\mathcal{R}_1 \leftarrow \{j \in [m_1] : P_j \leq q^{m_1+R_-(0),\alpha}_K\}$,
    $\mathcal{R}_2 \leftarrow \{j \in [m_2] : X_j \leq q^{m_1+R_-(0),\alpha}_K,L_j=1\}$ \\
    \Return $(\mathcal{R}_1, \mathcal{R}_2)$
    \label{salgo:int_p_cp}
\end{algorithm}

Similarly, we have the following theorem to show they can control the FDR at the target level.
\begin{Thm}[FDR Control for Integrated Tests]
\label{sthm:fdr_int}
    Let Algorithm~\ref{salgo:int_cp_cp} and Algorithm~\ref{salgo:int_p_cp} be defined as above.
    \begin{enumerate}
        \item In Algorithm~\ref{salgo:int_cp_cp}, if $(\mathbf{W}^1,\mathbf{L}^1)$ are competition statistics with respect to $\mathcal{H}^1_0 \subseteq \mathcal{H}^1$ and parameter $r_1$, $(\mathbf{W}^2,\mathbf{L}^2)$ are competition statistics with respect to $\mathcal{H}^2_0 \subseteq \mathcal{H}^2$ and parameter $r_2$, and they are mutually independent,
        \item In Algorithm~\ref{salgo:int_p_cp}, if $\mathbf{P}$ is randomized BH-valid with respect to $\mathcal{H}^1_0 \subseteq \mathcal{H}^1$, $(\mathbf{W},\mathbf{L})$ are competition statistics with respect to $\mathcal{H}^2_0 \subseteq \mathcal{H}^2$ and parameter $r$, and they are mutually independent,
    \end{enumerate}
    then the FDR satisfies
    \[
    \mathrm{FDR} = \mathbb{E}\left[\frac{|\mathcal{R}_1 \cap \mathcal{H}^1_0| + |\mathcal{R}_2 \cap \mathcal{H}^2_0|}{1 \vee (|\mathcal{R}_1| + |\mathcal{R}_2|)}\right] \leq \alpha.
    \]
\end{Thm}
We present the proof directly. As before, we focus only on Algorithm~\ref{salgo:int_p_cp}. From the proof of Theorem~\ref{thm:fdr_int}, it follows directly that
\[
\mathbb{E}\left[\frac{\sum_{j\in\mathcal{H}_0^1}\mathbf{1}\{P_j\leq q_K^{m_1+R_-(0),\alpha}\}}{1\vee K}\;\Bigg|\;\mathbf{W},\mathbf{L}\right]\leq\alpha\frac{|\mathcal{H}_0^1|}{m_1+R_-(0)}
\]
and
\[
\mathbb{E}\left[\frac{\sum_{j\in\mathcal{H}_0^2}\mathbf{1}\{Y_j\leq q_K^{m_1+R_-(0),\alpha}E_j,L_j=1\}}{1\vee K}\;\Bigg|\;\mathbf{P},\sigma_1\right]\leq\alpha\frac{R_-(0)}{m_1+R_-(0)}\frac{V_+(0)}{r+rV_-(0)}.
\]
By the rearrangement inequality,
\[
\mathbb{E}\left[\frac{R_-(0)}{m_1+R_-(0)}\frac{V_+(0)}{r+rV_-(0)}\;\Bigg|\;\mathbf{L}_{\mathcal{H}^2_1}\right]\leq\mathbb{E}\left[\frac{R_-(0)}{m_1+R_-(0)}\;\Bigg|\;\mathbf{L}_{\mathcal{H}^2_1}\right]\mathbb{E}\left[\frac{V_+(0)}{r+rV_-(0)}\right]
\]
and therefore
\begin{align*}
    \mathrm{FDR} &\leq \mathbb{E}\left[\alpha\frac{|\mathcal{H}_0^1|}{m_1+R_-(0)}+\alpha\frac{R_-(0)}{m_1+R_-(0)}\frac{V_+(0)}{r+rV_-(0)}\right] \\
    &= \mathbb{E}\left[\mathbb{E}\left[\alpha\frac{|\mathcal{H}_0^1|}{m_1+R_-(0)}+\alpha\frac{R_-(0)}{m_1+R_-(0)}\frac{V_+(0)}{r+rV_-(0)}\;\Bigg|\;\mathbf{L}_{\mathcal{H}^2_1}\right]\right] \\
    &\leq \mathbb{E}\left[\mathbb{E}\left[\alpha\frac{|\mathcal{H}_0^1|}{m_1+R_-(0)}+\alpha\frac{R_-(0)}{m_1+R_-(0)}\;\Bigg|\;\mathbf{L}_{\mathcal{H}^2_1}\right]\right]\leq\alpha.
\end{align*}

These two algorithms serve as examples illustrating that weighted operations can be introduced even with dependent random weights. The same analysis of Theorem~\ref{thm:fdr_int} is valid.

\subsection{More Analysis for Theorem~\ref{thm:cp_cp_any_dep}}

First, consider why a correction factor $c(r)$ is needed for inter-group dependence. For competition statistics $(\mathbf{W}^1,\mathbf{L}^1)$ and $(\mathbf{W}^2,\mathbf{L}^2)$, Algorithm~\ref{algo:int_cp_cp} yields $\mathbf{X}^1$, $\mathbf{X}^2$, and the threshold $K$. The false discovery rate is given by
\begin{align*}
    \mathrm{FDR} = \mathbb{E}\left[ \frac{1}{K} \sum_{g=1}^2 \sum_{j\in\mathcal{H}^g_0} \mathbf{1}\bigl\{ X^g_j \leq q^{m_1+m_2}_K \bigr\} \right].
\end{align*}

Under inter-group independence, the integration test remains valid because the conditional probability
\[
\mathbb{P}\bigl\{K\leq k \mid X^g_j\leq t,\; \mathbf{X}^{3-g},\; \mathbf{L}^1,\; \mathbf{L}^2\bigr\}
\]
is non-increasing in $t$ for any $j\in\mathcal{H}^g_0$, coinciding with the marginal probability
\[
\mathbb{P}\bigl\{K\leq k \mid X^g_j\leq t,\; \mathbf{L}^g\bigr\}.
\]
Inter-group dependence, however, breaks this monotonicity and invalidates the integration test. To overcome this, we must apply the correction factor.

Second, does the correction factor $c(r)$ restore the conditional PRDS property? It does not. The correction factor $c(r)$ is designed to adapt to the special dependence structure of competition statistics, which is not PRDS. If this correction factor is applied to the pBH part of the integrated test, the FDR remains uncontrolled. Hence $c(r)$ addresses the dependence structure specific to competition statistics without restoring conditional PRDS.

Third, what property of the randomized p-variable generated by competition statistics allows FDR control under arbitrary dependence with the correction factor $c(r)$? From the proof of Theorem~\ref{thm:cp_cp_any_dep}, if $\mathbf{P}$ are continuous p-values (generated p-values such as conformal p-values can be made continuous by adding independent uniform noise), we construct a series of random variables $U_k\in[0,1]$ satisfying
\[
\sum_{j\in\mathcal{H}_0}\mathbf{1}\{P_j\leq U_k\} + \lfloor mU_k \rfloor = k.
\]
In other words, $U_k$ solves the equation
\[
\sum_{j\in\mathcal{H}_0}\mathbf{1}\{P_j\leq t\} + \lfloor mt \rfloor = k.
\]
The solution is unique in terms of $\lfloor mt \rfloor$ and always exists when $k\leq m$, because the left-hand side is a step function that jumps by one as $t$ increases from $0$ to $1$. A sufficient condition for FDR control with the correction factor $c(r)$ is that $k-\lfloor mU_k \rfloor$ is stochastically dominated by a binomial distribution with parameters $k$ and $r/(1+r)$.

\section{Proofs for Lemmas in the Supplementary Material}
\label{app:lemmas}

\begin{proof}[Proof of Lemma~\ref{slem:overvariable}]

First, for a fixed threshold $t$,
\begin{align*}
    &\mathbb{P}\left(\delta(t)=k_3,V_+(t)=k_1,V_-(t)=k_2\right)\\
    &= \sum_{l\in \Omega(k_1,k_2,k_3)}\sum_{j_1,j_2,\cdots,j_{k_1+k_2}\in\mathcal{H}_0}
       \mathbb{P}\left(W_{j_1}>W_{j_2}>\cdots>W_{j_{k_1+k_2}}>t>W_{\max}(j_1,j_2,\cdots,j_{k_1+k_2})\right)\\
    &\qquad \times \mathbb{P}\left(L_{j_s}=l_s;s=1,2,\cdots,k_1+k_2\right)
\end{align*}
by the independence of $\mathbf{W}$ and $\mathbf{L}_{\mathcal{H}_0}$, where
\[
W_{\max}(j_1,j_2,\cdots,j_{k_1+k_2})=\max\left\{W_{j}:h_{j}=0,j\notin \{j_s:s=1,2,\cdots,k_1+k_2\}\right\}
\]
and
\[
\Omega(k_1,k_2,k_3)=\left\{l\in\{0,1\}^{k_1+k_2}:\sum_{s=1}^{k_1+k_2}l_s=k_1,\sum_{s=1}^{k_3}l_s=k_3,l_{k_3+1}=0\right\}.
\]
Similarly,
\begin{align*}
    &\mathbb{P}\left(V_+(t)=k_1,V_-(t)=k_2\right)\\
    &= \sum_{l\in \Omega(k_1,k_2)}\sum_{j_1,j_2,\cdots,j_{k_1+k_2}\in\mathcal{H}_0}
       \mathbb{P}\left(W_{j_1}>W_{j_2}>\cdots>W_{j_{k_1+k_2}}>t>W_{\max}(j_1,j_2,\cdots,j_{k_1+k_2})\right)\\
    &\qquad \times \mathbb{P}\left(L_{j_s}=l_s;s=1,2,\cdots,k_1+k_2\right)
\end{align*}
where
\[
\Omega(k_1,k_2)=\left\{l\in\{0,1\}^{k_1+k_2}:\sum_{s=1}^{k_1+k_2}l_s=k_1\right\}=\bigcup_{k_3=0}^{k_1}\Omega(k_1,k_2,k_3).
\]

By the definition of competition statistics, for any $l\in\Omega(k_1,k_2,k_3)$ and $j_1,j_2,\cdots,j_{k_1+k_2}\in\mathcal{H}_0$,
\[
\mathbb{P}\left(L_{j_s}=l_s;s=1,2,\cdots,k_1+k_2\right)=\left(\frac{r}{r+1}\right)^{k_1}\left(\frac{1}{r+1}\right)^{k_2}.
\]
Therefore,
\begin{align*}
    &\mathbb{P}\left(\delta(t)=k_3\,\middle|\,V_+(t)=k_1,V_-(t)=k_2\right)
      = \frac{\mathbb{P}\left(\delta(t)=k_3,V_+(t)=k_1,V_-(t)=k_2\right)}
             {\mathbb{P}\left(V_+(t)=k_1,V_-(t)=k_2\right)}\\[4pt]
    &= \frac{\displaystyle\sum_{l\in \Omega(k_1,k_2,k_3)}
                     \sum_{j_1,j_2,\cdots,j_{k_1+k_2}\in\mathcal{H}_0}
                     \mathbb{P}\left(W_{j_1}>\cdots>W_{j_{k_1+k_2}}>t>W_{\max}(j_1,j_2,\cdots,j_{k_1+k_2})\right)}
            {\displaystyle\sum_{l\in \Omega(k_1,k_2)}
                     \sum_{j_1,j_2,\cdots,j_{k_1+k_2}\in\mathcal{H}_0}
                     \mathbb{P}\left(W_{j_1}>\cdots>W_{j_{k_1+k_2}}>t>W_{\max}(j_1,j_2,\cdots,j_{k_1+k_2})\right)}\\[4pt]
    &= \frac{|\Omega(k_1,k_2,k_3)|}{|\Omega(k_1,k_2)|}
       = \frac{\binom{k_1}{k_3}\cdot k_3!\cdot k_2\cdot (k_1-k_3+k_2-1)!}{(k_1+k_2)!}
       = \binom{k_1-k_3+k_2-1}{k_2-1}\Bigg/\binom{k_1+k_2}{k_2}\\[4pt]
    &= f(k_3;k_1,k_2),
\end{align*}
which is independent of $t$.

Next we show that the same result holds for the data-driven threshold $T$.
\begin{align*}
    &\mathbb{P}\left(\delta(T)=k_3,V_+(T)=k_1,V_-(T)=k_2\right)\\
    &= \sum_{t}\mathbb{P}\left(\delta(t)=k_3,V_+(t)=k_1,V_-(t)=k_2,T=t\right)\\
    &= \sum_{t}\mathbb{P}\left(T=t\;\middle|\;\delta(t)=k_3,V_+(t)=k_1,V_-(t)=k_2\right)
       \mathbb{P}\left(\delta(t)=k_3,V_+(t)=k_1,V_-(t)=k_2\right)\\
    &= \sum_{t}\mathbb{P}\left(T=t\;\middle|\;V_+(t)=k_1,V_-(t)=k_2\right)
       \mathbb{P}\left(\delta(t)=k_3,V_+(t)=k_1,V_-(t)=k_2\right)\\
    &= f(k_3;k_1,k_2)\,\mathbb{P}\left(V_+(T)=k_1,V_-(T)=k_2\right).
\end{align*}
Hence,
\[
\mathbb{P}\left(\delta(T)=k\big|V_+(T),V_-(T)\right)=f\left(k;V_+(T),V_-(T)\right).
\]

With the exact conditional distribution known, we can compute the conditional expectation by a combinatorial argument. Treat $\{j\in\mathcal{H}_0:W_j\geq T,\,L_j=0\}$ as $V_-(T)$ separating points that partition $\{j\in\mathcal{H}_0:W_j\geq T,\,L_j=1\}$ into $V_-(T)+1$ bins. The variable $\delta(T)$ counts the number of labeled null variables in the first bin. Because the permutation of null variables is uniformly random, the expected count in each bin is the same. Since the $V_-(T)+1$ bins partition $V_+(T)$ total labeled null variables,
\[
\mathbb{E}\left[\delta(T)\big|V_+(T),V_-(T)\right]=\frac{V_+(T)}{1+V_-(T)}.
\]
\end{proof}

\begin{proof}[Proof of Lemma~\ref{slem:biovervariable}]

The first fact is obvious.

If $\mathbf{1}\{W_i\geq T,L_i=0\}\mathbf{1}\{W_k\geq T_i,L_k=0\}=1$, for any $t\leq T_i$,
\begin{align*}
    \sum_{j\in\mathcal{H}\backslash\{i\}}\mathbf{1}\{W_j\geq t,L_j=1\}&=\sum_{j\in\mathcal{H}}\mathbf{1}\{W_j\geq t,L_j=1\}=\sum_{j\in\mathcal{H}\backslash\{k\}}\mathbf{1}\{W_j\geq t,L_j=1\},\\
    \sum_{j\in\mathcal{H}\backslash\{i\}}\mathbf{1}\{W_j\geq t,L_j=0\}&=\sum_{j\in\mathcal{H}}\mathbf{1}\{W_j\geq t,L_j=0\}-1=\sum_{j\in\mathcal{H}\backslash\{k\}}\mathbf{1}\{W_j\geq t,L_j=0\},
\end{align*}
which implies $T_k\leq T_i$ and $T_k\geq T_i$, so $T_k=T_i$.

If $\mathbf{1}\{W_k\geq T_i,L_k=0\}=0$, for any $t$,
\begin{align*}
    \sum_{j\in\mathcal{H}\backslash\{k\}}\mathbf{1}\{W_j\geq t,L_j=1\}+1&\geq\sum_{j\in\mathcal{H}}\mathbf{1}\{W_j\geq t,L_j=1\}\geq\sum_{j\in\mathcal{H}\backslash\{k\}}\mathbf{1}\{W_j\geq t,L_j=1\},\\
    \sum_{j\in\mathcal{H}}\mathbf{1}\{W_j\geq t,L_j=0\}-1&\leq\sum_{j\in\mathcal{H}\backslash\{k\}}\mathbf{1}\{W_j\geq t,L_j=0\}\leq\sum_{j\in\mathcal{H}}\mathbf{1}\{W_j\geq t,L_j=0\},
\end{align*}
and the right part of the second inequality is equal when $t\geq T_i$, so $T_k\geq T$ and $T_k\leq T$ naturally, hence $T=T_k$.
\end{proof}

\begin{proof}[Proof of Lemma~\ref{slem:level_dim}]

The BH threshold for $\mathbf{P}$ at level $m\alpha/|S|$ is $q_k^{m,m\alpha/|S|}=k(m\alpha/|S|)/m=k\alpha/|S|$. Since $P_j=+\infty$ for all $j\notin S$, the order statistics satisfy $P_{(k)}=P_{S,(k)}$ for $k\leq|S|$ and $P_{(k)}=+\infty$ for $k>|S|$. Hence the BH rejection count for $\mathbf{P}$ is
\[
K=\max\left\{k: P_{(k)}\leq\frac{k\alpha}{|S|}\right\}
  =\max\left\{k\leq|S|: P_{S,(k)}\leq\frac{k\alpha}{|S|}\right\},
\]
which coincides with the rejection count for $\mathbf{P}_S$ at level $\alpha$. Therefore
\[
\mathcal{R}_{m\alpha/|S|}(\mathbf{P})=\left\{j:P_j\leq\frac{K\alpha}{|S|}\right\}
=\left\{j\in S:P_{j}\leq\frac{K\alpha}{|S|}\right\}
=\mathcal{R}_{\alpha}(\mathbf{P}_S).
\]
\end{proof}

\begin{proof}[Proof of Lemma~\ref{slem:uniform_split}]

For any $\boldsymbol{l}\in\{0,1\}^{m_0}$,
\[
\mathbb{P}\left\{\mathbf{L}_{\mathcal{H}_0}=\boldsymbol{l}\mid\mathbf{W},\mathbf{L}_{\mathcal{H}_1}\right\}=\left(\frac{r}{1+r}\right)^{\sum_{i=1}^{m_0}l_i}\left(\frac{1}{1+r}\right)^{\sum_{i=1}^{m_0}(1-l_i)}.
\]
Let $\mathcal{L}_{k}=\{\boldsymbol{l}\in\{0,1\}^{m_0}:\sum_{i=1}^{m_0}l_i=k\}$. Then $\{V_+(0)=k,V_-(0)=m_0-k\}=\{\mathbf{L}_{\mathcal{H}_0}\in\mathcal{L}_k\}$ and
\[
\mathbb{P}\left\{V_+(0)=k,V_-(0)=m_0-k\mid\mathbf{W},\mathbf{L}_{\mathcal{H}_1}\right\}
=\sum_{\boldsymbol{l}\in\mathcal{L}_k}\mathbb{P}\left\{\mathbf{L}_{\mathcal{H}_0}=\boldsymbol{l}\mid\mathbf{W},\mathbf{L}_{\mathcal{H}_1}\right\}
=|\mathcal{L}_k|\left(\frac{r}{1+r}\right)^{k}\left(\frac{1}{1+r}\right)^{m_0-k}.
\]
Hence, conditional on $\sigma_{\mathcal{H}_1}$,
\[
\mathbb{P}\left\{\mathbf{L}_{\mathcal{H}_0}=\boldsymbol{l}\mid\sigma_{\mathcal{H}_1}\right\}=
\begin{cases}
\dfrac{1}{|\mathcal{L}_{V_+(0)}|}, & \boldsymbol{l}\in\mathcal{L}_{V_+(0)},\\[6pt]
0, & \boldsymbol{l}\in\{0,1\}^{m_0}\setminus\mathcal{L}_{V_+(0)}.
\end{cases}
\]
In other words, $V_+(0)=\{i\in\mathcal{H}_0:L_i=1\}$ is uniformly distributed over all subsets of $\mathcal{H}_0$ of size $V_+(0)$.
\end{proof}

\begin{proof}[Proof of Lemma~\ref{slem:equiv_rejection}]

By the definition of $K$, we have
\[
K \leq \sum_{j \in \mathcal{H}_1} \mathbf{1}\{P_j \leq q^{R_+(0),\alpha}_K E_j\} + \sum_{j \in \mathcal{H}_0} \mathbf{1}\{P_j \leq q^{R_+(0),\alpha}_K E_j\} = \sum_{j=1}^m \mathbf{1}\{P_j \leq q^{R_+(0),\alpha}_K E_j\}.
\]
We show that the strict inequality cannot hold. Suppose for contradiction that
\[
K < \sum_{j=1}^m \mathbf{1}\{P_j \leq q^{R_+(0),\alpha}_K E_j\}.
\]
Then
\begin{align*}
    K + 1 &\leq \sum_{j=1}^m \mathbf{1}\{P_j \leq q^{R_+(0),\alpha}_K E_j\} \\
           &\leq \sum_{j=1}^m \mathbf{1}\{P_j \leq q^{R_+(0),\alpha}_{K+1} E_j\},
\end{align*}
where the second inequality follows from $q^{R_+(0),\alpha}_K \leq q^{R_+(0),\alpha}_{K+1}$ by the monotonicity of the critical values. This contradicts the maximality of $K$. Therefore,
\[
K = \sum_{j=1}^m \mathbf{1}\{P_j \leq q^{R_+(0),\alpha}_K E_j\}.
\]

Now let $\mathbf{P}'_{\mathcal{R}_+(0)} = (P_j/E_j)_{j\in\mathcal{R}_+(0)}$ be the weighted p-values. The equality above implies $P'_{(K)} \leq q_K^{R_+(0),\alpha}$, so $K \leq |\mathcal{R}_{\alpha}(\mathbf{P}'_{\mathcal{R}_+(0)})|$. For any $k > K$, the definition of $K$ gives
\[
k > \sum_{j=1}^m \mathbf{1}\{P_j \leq q_k^{R_+(0),\alpha} E_j\},
\]
which means $P'_{(k)} > q_k^{R_+(0),\alpha}$. Hence $k > |\mathcal{R}^{\mathrm{BH}}_{\alpha}(\mathbf{P}'_{\mathcal{R}_+(0)})|$ for all $k > K$, and consequently $K \geq |\mathcal{R}^{\mathrm{BH}}_{\alpha}(\mathbf{P}'_{\mathcal{R}_+(0)})|$. Combining the two inequalities yields
\[
K = |\mathcal{R}^{\mathrm{BH}}_{\alpha}(\mathbf{P}'_{\mathcal{R}_+(0)})|.
\]
\end{proof}

\begin{proof}[Proof of Lemma~\ref{slem:fdr_eq}]
The expression inside each expectation is a measurable function of $(\mathbf{W},\mathbf{L})$ and $(\mathbf{W}',\mathbf{L}')$, respectively. Since $(\mathbf{W},\mathbf{L})$ and $(\mathbf{W}',\mathbf{L}')$ are identically distributed, the two expectations are equal.
\end{proof}

\section{More Numerical Results}
\label{app:morefig}

\subsection{More Analysis of the Prescreen Test}

First, we show more results of Figure~\ref{fig:prescreen_cal_box3}.
\begin{figure}[H]
    \centering
    \includegraphics[width=0.9\linewidth]{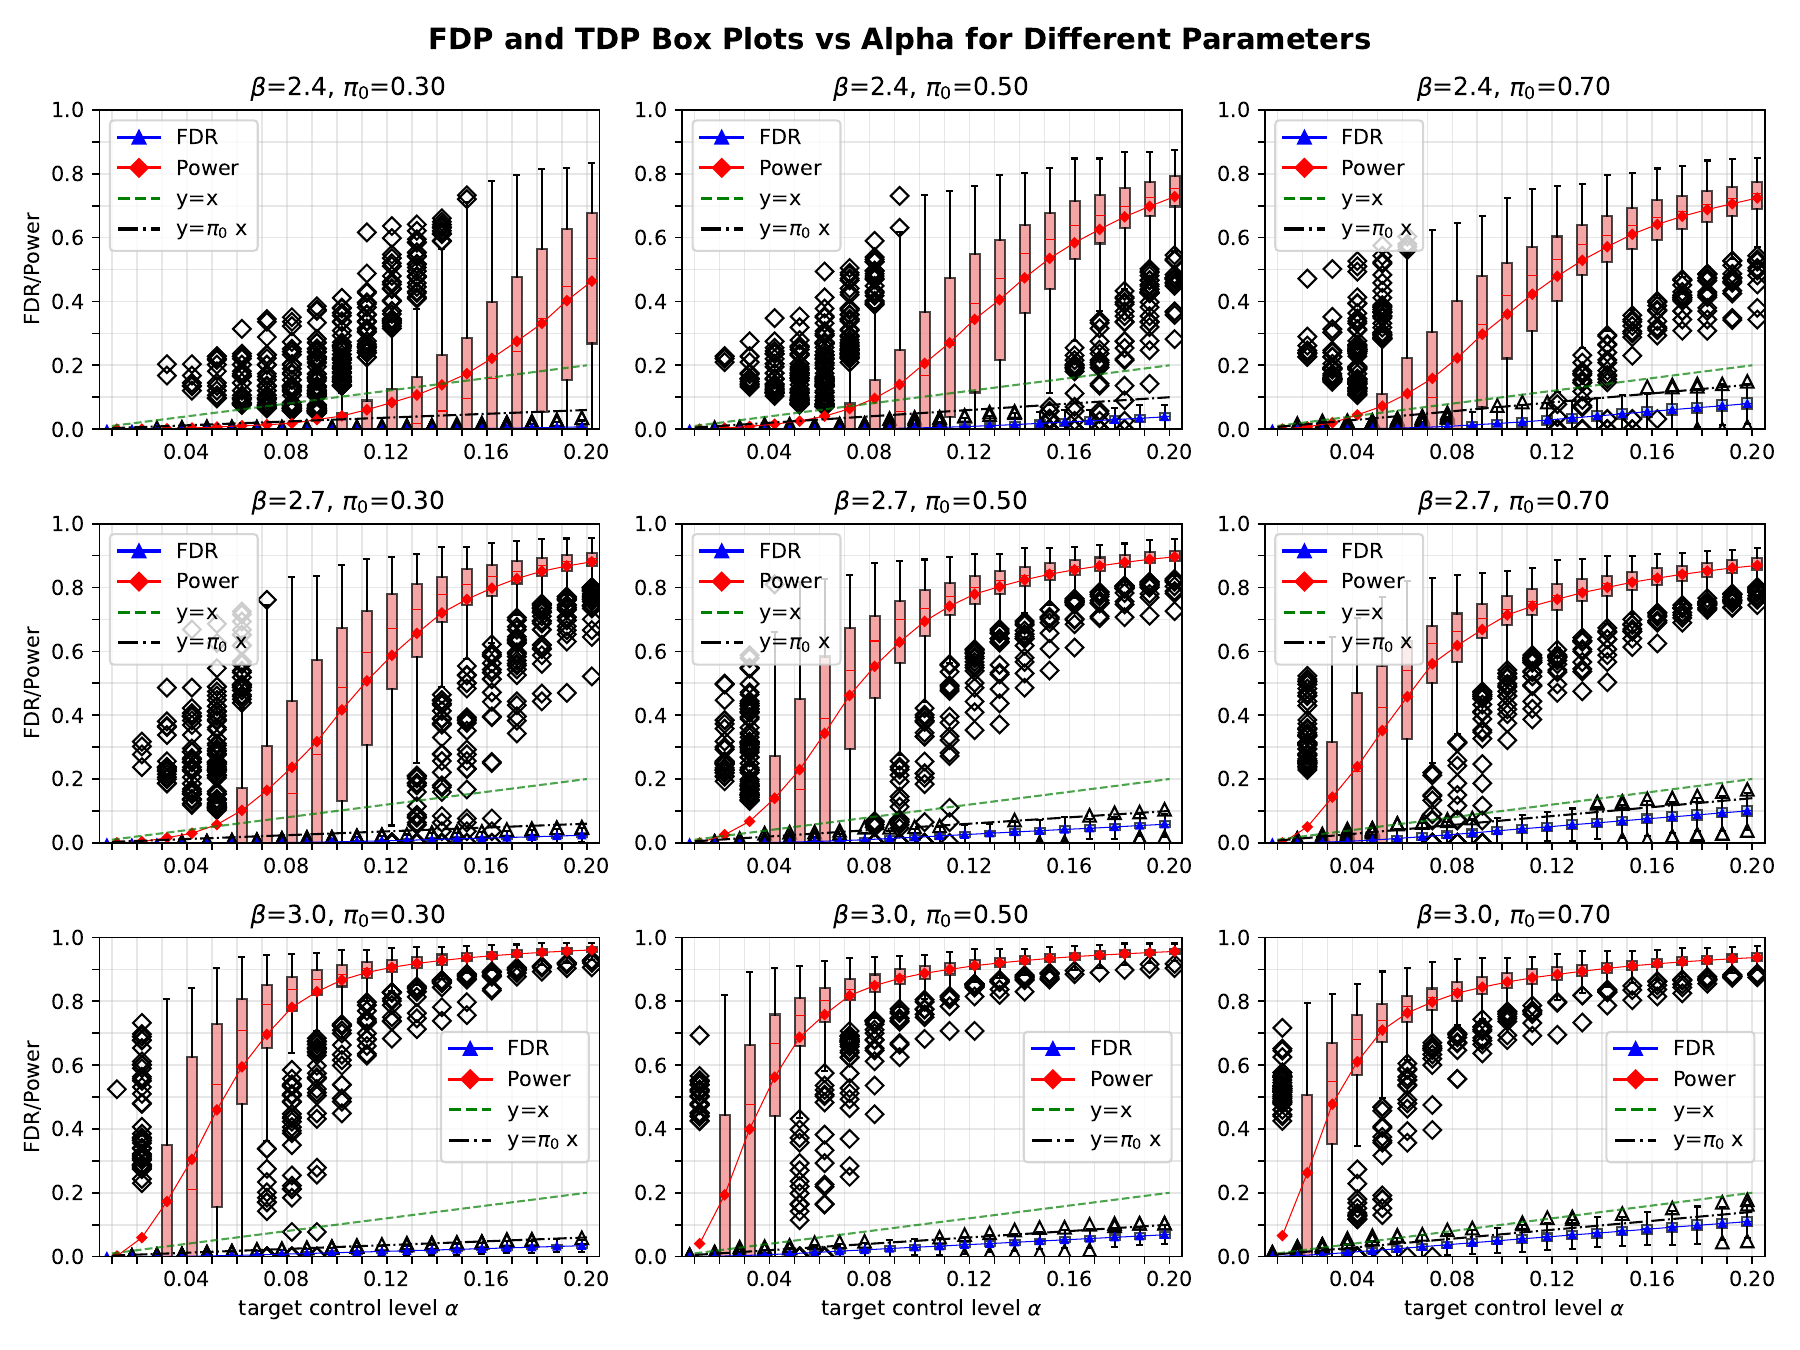}
    \caption{The box plots of FDR under different signal strength $\beta$ and parameter $\pi_0$, target levels settings $\alpha$.}
    \label{fig:prescreen_cal_box}
\end{figure}

We emphasize that when performing the test via the conformal BH procedure with a calibration set constructed through prescreening, an important issue is that the prescreening step is not guaranteed to be perfectly accurate. Specifically, the constructed calibration set $\mathcal{D}^{cal} = \mathcal{D}^{cal}_0 + \mathcal{D}^{cal}_1$ is only partially exchangeable. While exchangeability holds within $\mathcal{D}^{cal}_0$ and null hypotheses, it does not hold for $\mathcal{D}^{cal}_1$, which should be incorporated as weights in the procedure. For instance, in our simulation experiments, if we specifically examine the behavior of FDR under the same experimental setting, we obtain the following results.
\begin{figure}[H]
    \centering
    \includegraphics[width=0.9\linewidth]{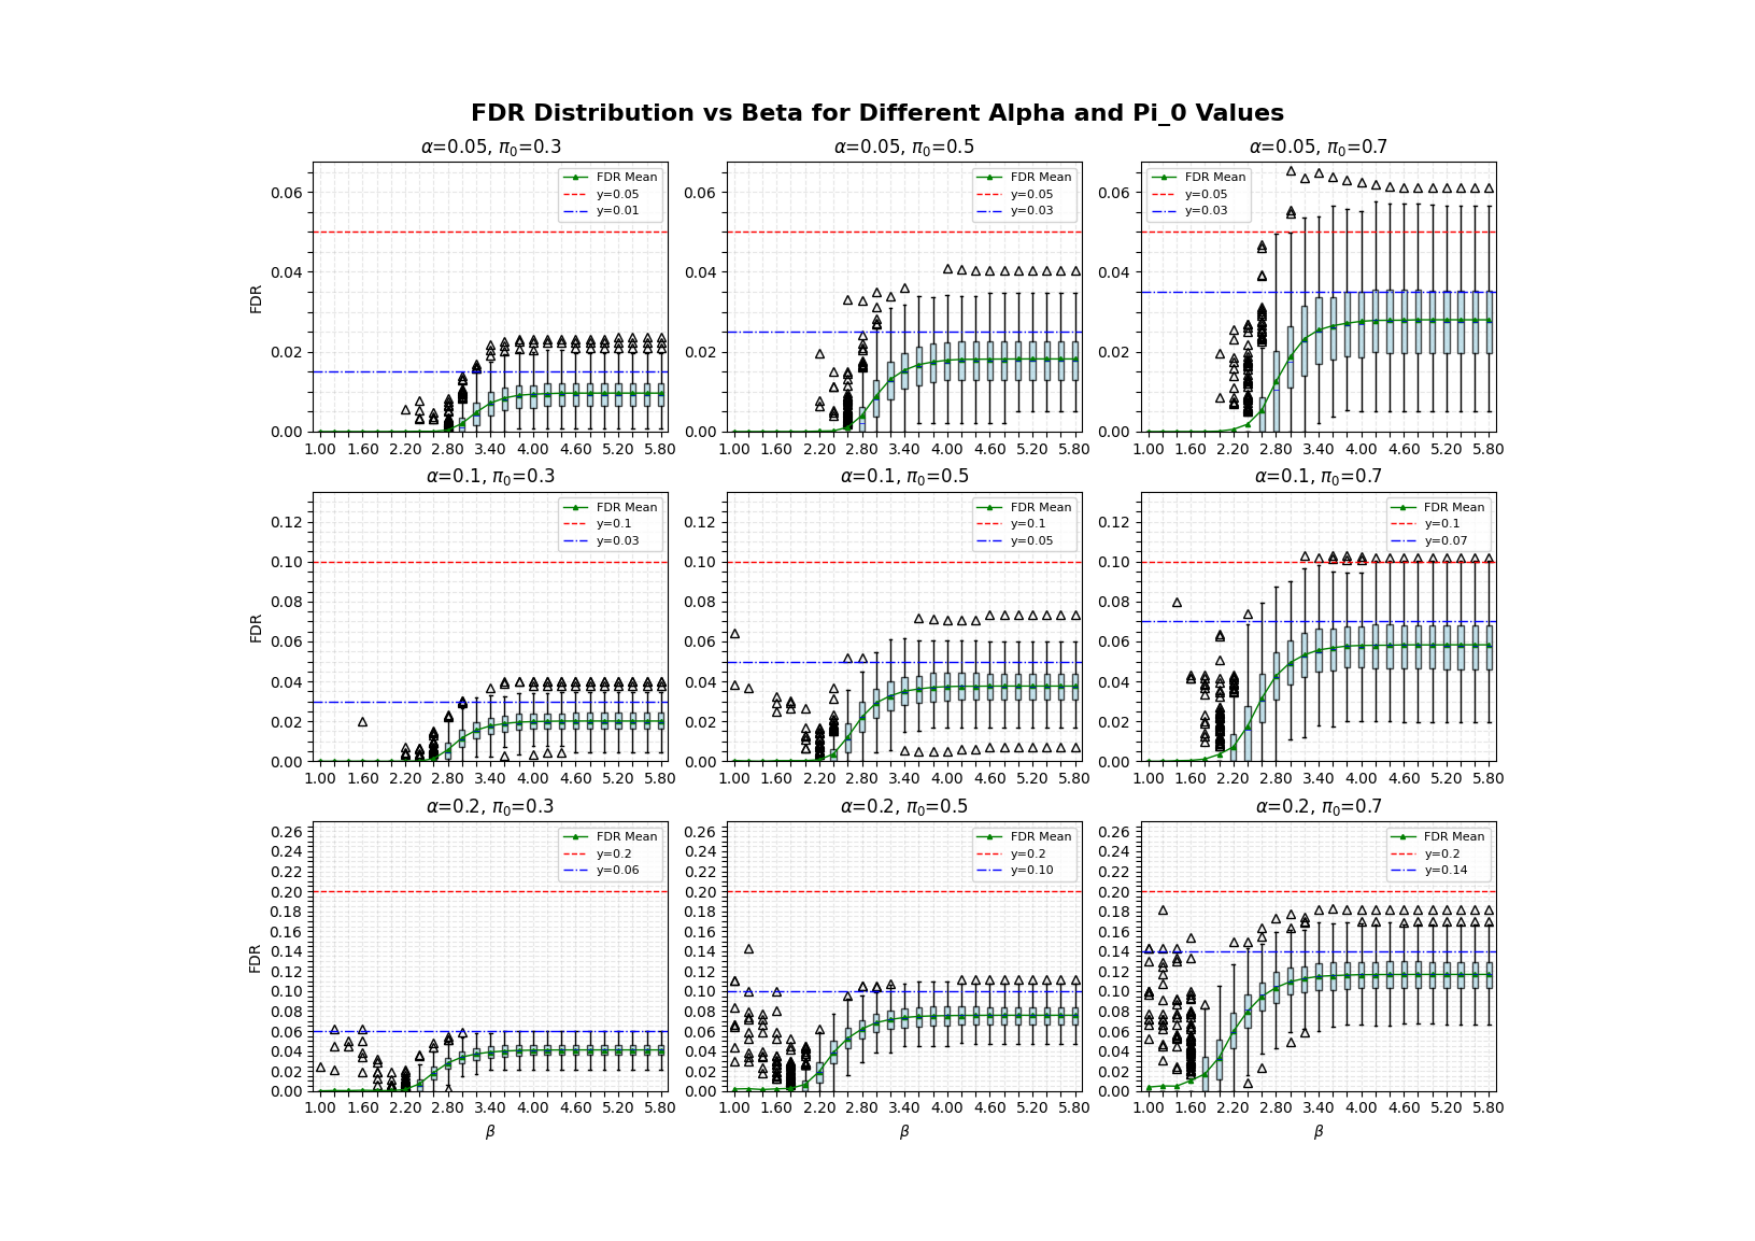}
    \caption{The box plots of FDR under different signal strength $\beta$ and parameter $\pi_0$, target levels settings $\alpha$.}
    \label{fig:prescreen_cal_focus_fdr}
\end{figure}
Theoretically, according to Theorem~\ref{thm:fdr_ran_problem} and Theorem~\ref{thm:fdr_wbh}, we obtain
\[
\mathrm{FDR}=\mathbb{E}\left[\mathbb{E}\left[\frac{|\mathcal{R}_{\alpha}(\mathbf{P}(\mathbf{X}_{\mathcal{D}^{test}},\mathbf{X}_{\mathcal{D}^{cal}}))\cap\mathcal{D}^{test}\cap\mathcal{H}_0|}{1\vee|\mathcal{R}_{\alpha}(\mathbf{P}(\mathbf{X}_{\mathcal{D}^{test}},\mathbf{X}_{\mathcal{D}^{cal}}))|}\mid\mathbf{X}^{pre}\right]\right]\leq\alpha\mathbb{E}_{\mathbf{X}^{pre}}\left[\frac{|\mathcal{D}^{test}\cap\mathcal{H}_0|}{1\vee|\mathcal{D}^{test}|}\cdot\frac{1+|\mathcal{D}^{cal}|}{1+|\mathcal{D}^{cal}_0|}\right].
\]
Notice that
\[
\frac{|\mathcal{D}^{test}\cap\mathcal{H}_0|}{1\vee|\mathcal{D}^{test}|}\cdot\frac{1+|\mathcal{D}^{cal}|}{1+|\mathcal{D}^{cal}_0|}=\frac{|\mathcal{H}_0|-|\mathcal{D}_0^{cal}|}{1\vee(|\mathcal{H}|-|\mathcal{D}^{cal}|)}\cdot\frac{1+|\mathcal{D}^{cal}|}{1+|\mathcal{D}^{cal}_0|}.
\]
Without loss of generality, we assume that the pre-screening process ensures that $\mathcal{H} \setminus \mathcal{D}^{cal}$ is always nonempty (for example, by guaranteeing that the most significant hypothesis is never screened out). Then, let $|\mathcal{H}|=h, |\mathcal{D}^{cal}|=c, |\mathcal{D}_0^{cal}|=c_0$, we have for any $\varepsilon\geq 0$, if $c_0\geq (1+\varepsilon)\pi_0c$
\[
\frac{|\mathcal{H}_0|-|\mathcal{D}_0^{cal}|}{1\vee(|\mathcal{H}|-|\mathcal{D}^{cal}|)}\cdot\frac{1+|\mathcal{D}^{cal}|}{1+|\mathcal{D}^{cal}_0|}=\frac{\pi_0h-c_0}{h-c}\cdot\frac{1+c}{1+c_0}\leq\pi_0\cdot\frac{1}{(1+\varepsilon)\pi_0}=\frac{1}{1+\varepsilon},
\]
hence
\[
\mathrm{FDR}\leq\inf_{\varepsilon\geq0}\frac{\alpha}{1+\varepsilon}\mathbb{P}_{\mathbf{X}^{pre}}\{|\mathcal{D}_0^{cal}|\geq(1+\varepsilon)\pi_0|\mathcal{D}^{cal}|\}+\mathbb{P}_{\mathbf{X}^{pre}}\{|\mathcal{D}_0^{cal}|<(1+\varepsilon)\pi_0|\mathcal{D}^{cal}|\}.
\]

This inequality follows from the data splitting method, which ensures that the samples used for testing and those used for pre-screening are independent. The second term can be made sufficiently small by choosing an appropriate screening procedure. To visually demonstrate the influence of the pre-screening threshold on FDR, we fix the signal strengths at $\beta = 2, 3, 4$, set the target significance level to $\alpha = 0.2$ and null proportion $\pi_0=0.7$, and define the calibration set constructed with pre-screening as $\mathcal{D}^{cal} = \{ i : |X^{pre}_i| < \tau \}$. The results are as follows.
\begin{figure}[H]
    \centering
    \includegraphics[width=0.9\linewidth]{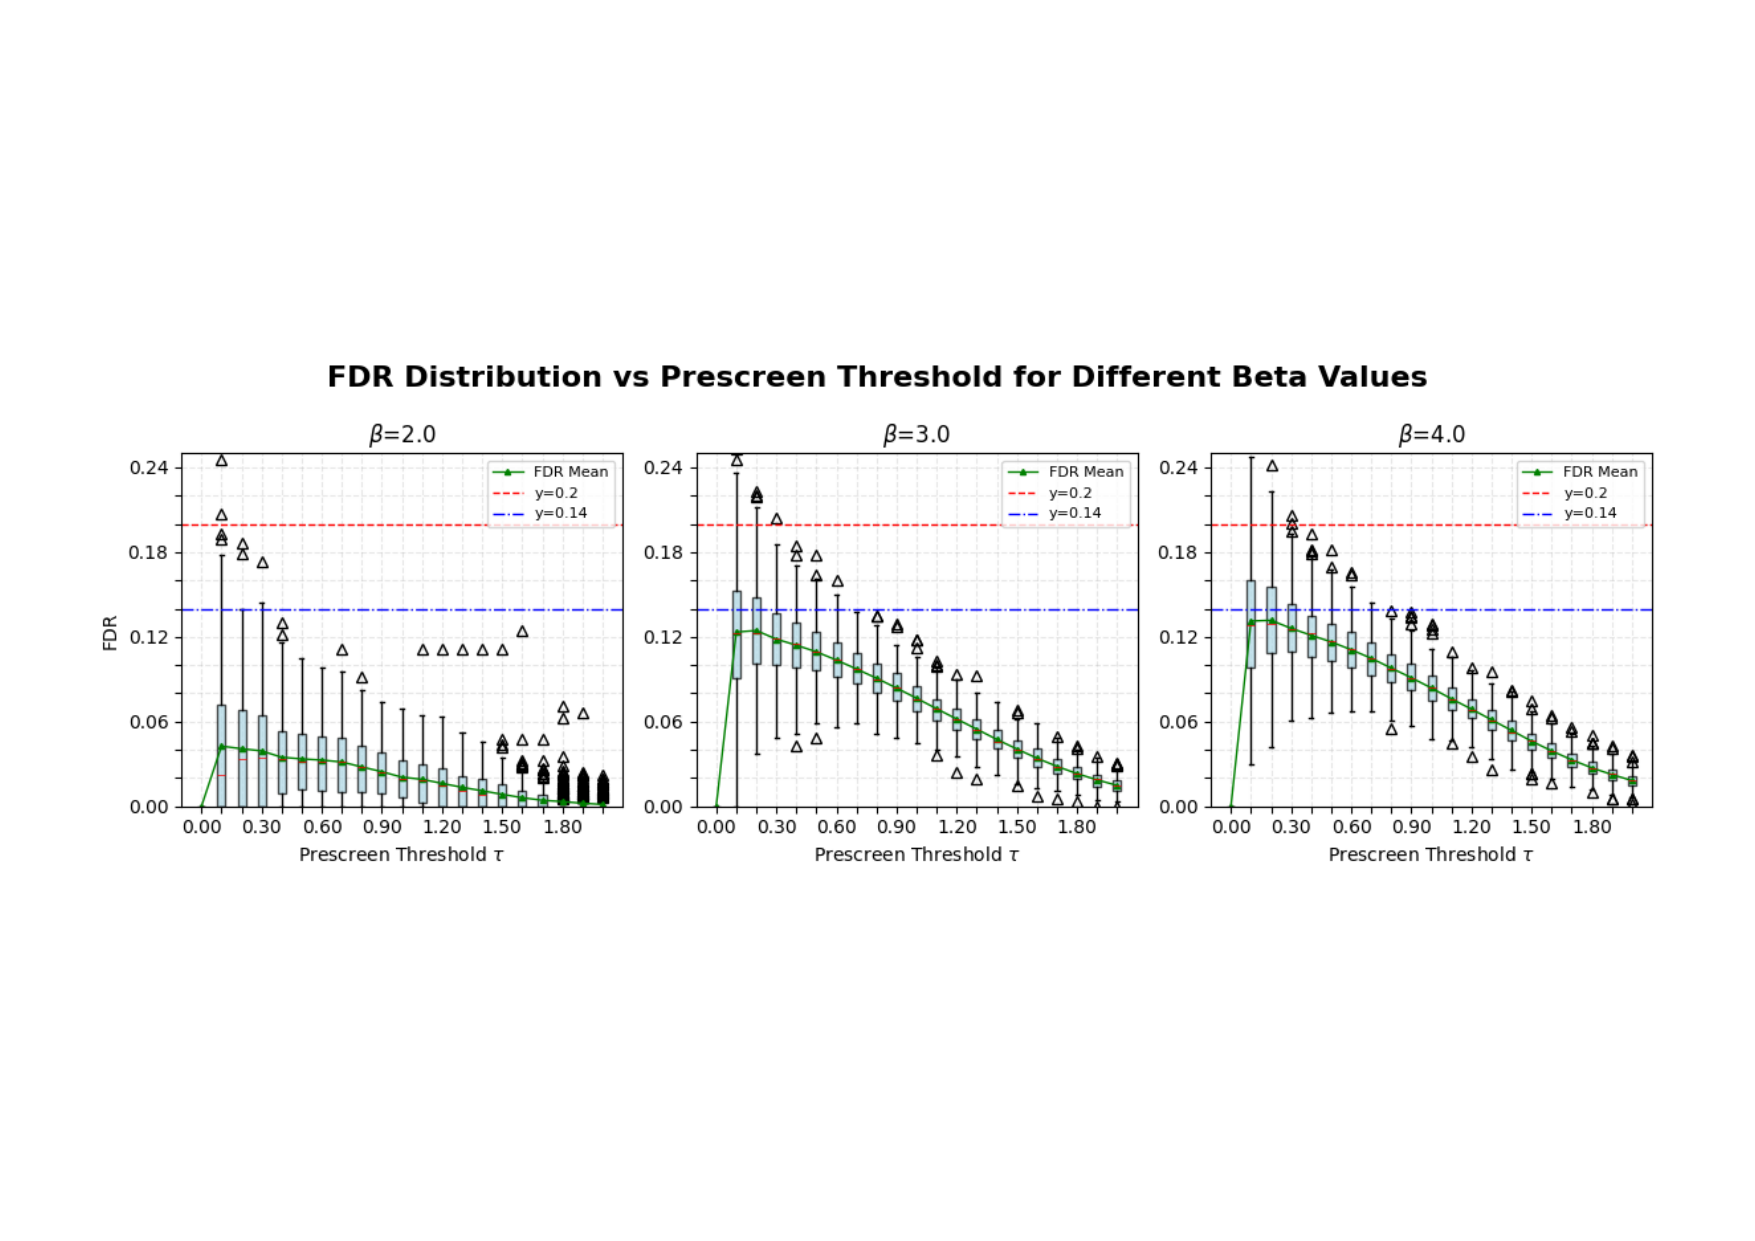}
    \caption{The box plots of FDR under different pre-screening threshold and signal strength setting $\beta$.}
    \label{fig:prescreen_cal_focus_threshold}
\end{figure}
In practice, whether pre-screening compromises FDR control should be examined case by case. However, the results above suggest that in most routine cases this concern can be disregarded. A reasonable pre-screening procedure tends to first screen out null hypotheses, then nonnull hypotheses, so that the proportion of the two remains below the null proportion $\pi_0$. When this proportion approaches $\pi_0$, most of the nulls have been screened out, which makes the first fractional term extremely small and renders the test results actually more conservative.

\subsection{FDR and Power Comparison between Conformal and Competition Methods}

According to the analysis presented in our work, the conformal test and the competition test reside within a unified framework, in other words, the conformal test can be regarded as a special case of the competition test. This naturally raises a further question: if the sample conditions simultaneously satisfy the requirements for both the conformal test and the competition test, how will the test results differ between the two?

We design the following experiment: generate random variables $X_i \sim N(\mu_i, 1)$, $i = 1, 2, \dots, m$, corresponding to the tests, where the testing set and the null set are $\mathcal{H} = [m]$, $\mathcal{H}_0 = [m_0]$, respectively. If $i \in \mathcal{H}_0$, set $\mu_i = 0$. If $i \in \mathcal{H}_1$, set $\mu_i = \beta$, where $\beta$ is the signal strength. Simultaneously, generate reference random variables $X^{ref}_i \sim N(0, 1)$, $i = 1, 2, \dots, m$. Consider three different tests:
\begin{enumerate}
    \item \textbf{Competition test:} construct competition statistics $W_i = \max\{|X_i|, |X^{ref}_i|\}$, $L_i = \mathbf{1}\{|X_i| \geq |X^{ref}_i|\}$, with test result $\mathcal{R}_{\alpha,1}(\mathbf{W}, \mathbf{L})$.
    \item \textbf{Conformal test:} construct conformal p-values $\mathbf{P}(\mathbf{X}, \mathbf{X}^{ref})$, with test result $\mathcal{R}_{\alpha}(\mathbf{P})$.
    \item \textbf{Oracle conformal test:} also use conformal p-values, but with test result $\mathcal{R}_{\alpha \pi_0^{-1}}(\mathbf{P})$, where $\pi_0 = m^{-1} m_0$.
\end{enumerate}
Take $m = 1000$ and perform $300$ repeated experiments. The experimental results are as follows.
\begin{figure}[H]
    \centering
    \includegraphics[width=0.9\linewidth]{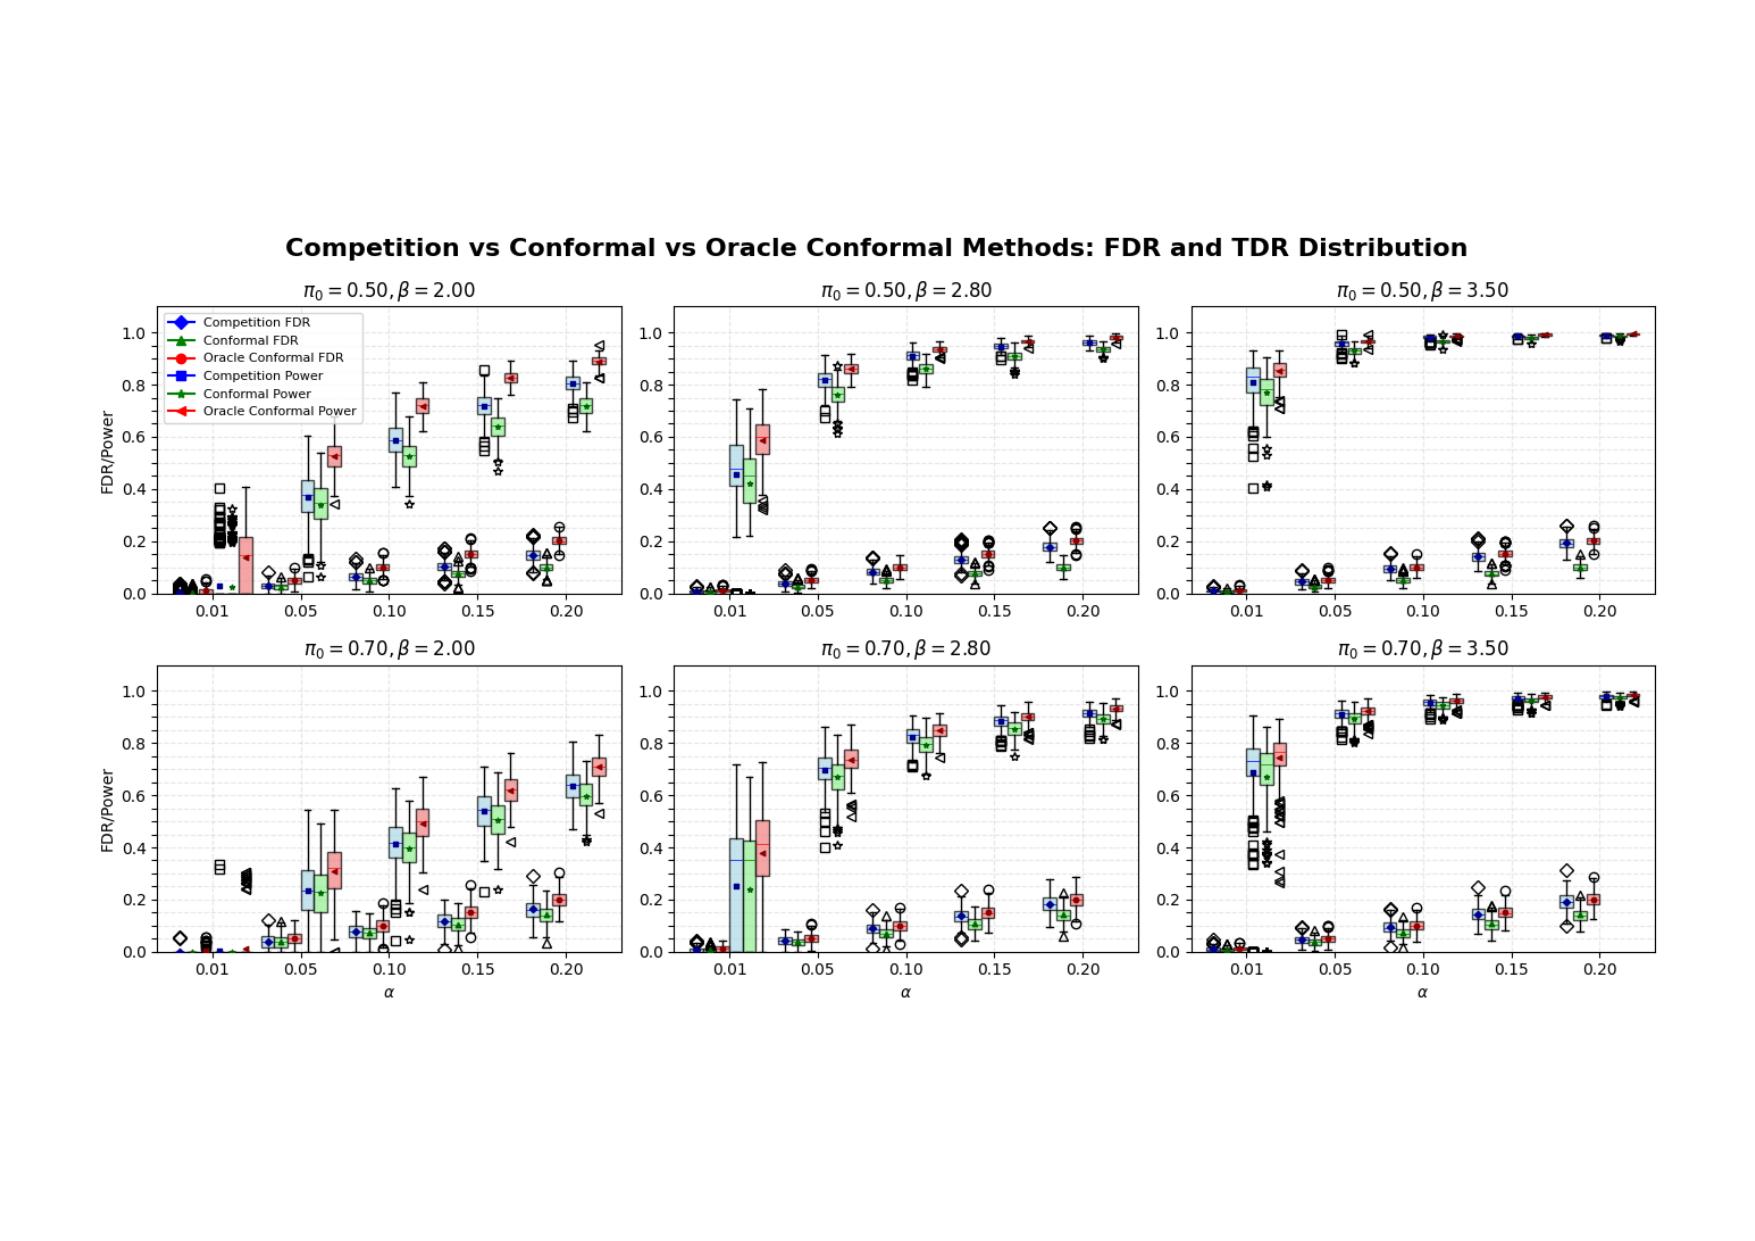}
    \caption{The box plots of FDR and Power under different target control levels $\alpha$ and parameter setting $\beta,\pi_0$}
    \label{fig:cp_vs_cf_vs_ocf_box}
\end{figure}
Furthermore, we can employ a larger reference set. Consider constructing a set of reference random variables $\mathbf{X}^{ref,j}$, $j=1,2,\dots,d$, and denote $\mathbf{X}^{ref}=(\mathbf{X}^{ref,1},\mathbf{X}^{ref,2},\dots,\mathbf{X}^{ref,d})$. We consider the three tests mentioned above, where the conformal test and the oracle conformal test remain unchanged, while the competition test requires the asymmetry coefficient to be set as $r=d^{-1}$, with the test result $\mathcal{R}_{\alpha,d^{-1}}(\mathbf{W},\mathbf{L})$, where
\[
W_i = \max\bigl\{|X_i|, |X^{ref,j}_i| : j=1,2,\dots,d\bigr\}, \qquad L_i = \prod_{j=1}^{d} \mathbf{1}\{|X_i| \geq |X^{ref,j}_i|\}.
\]
Let $d=20$, the experimental results are as follows.
\begin{figure}[H]
    \centering
    \includegraphics[width=0.9\linewidth]{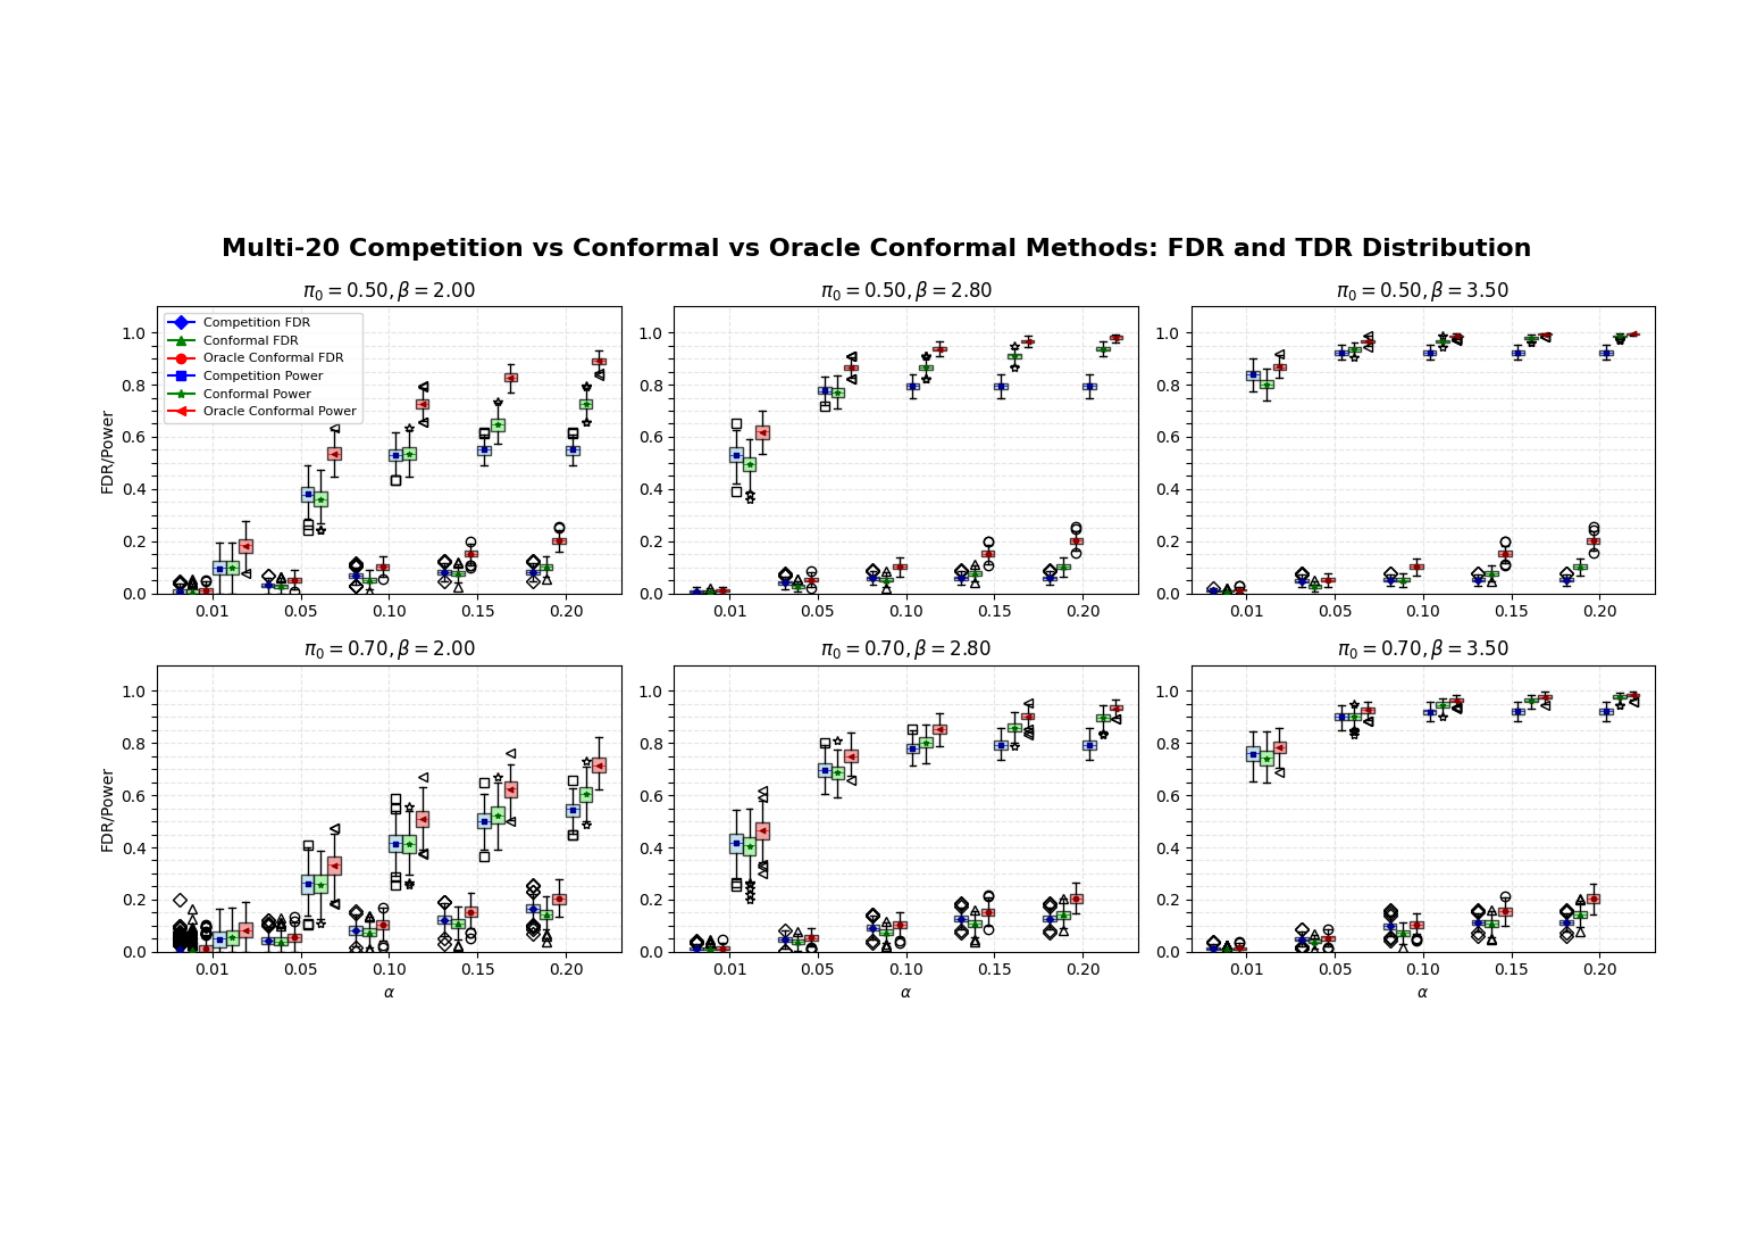}
    \caption{The box plots of FDR and Power under different target control levels $\alpha$ and parameter setting $\beta,\pi_0$}
    \label{fig:multi_cp_vs_cf_vs_ocf_box}
\end{figure}
Note that when a larger reference set is used, the test outcomes exhibit certain differences. Notably, the stability of the tests is greatly improved, both for the conformal test and the competition test. To examine the influence of the size of reference set on the two types of tests, we take the competition test as the baseline and compute the differences between the competition test and the conformal test, as well as between the competition test and the oracle conformal test. With target control level $\alpha=0.1$, the experimental results are as follows.
\begin{figure}[H]
    \centering
    \includegraphics[width=0.9\linewidth]{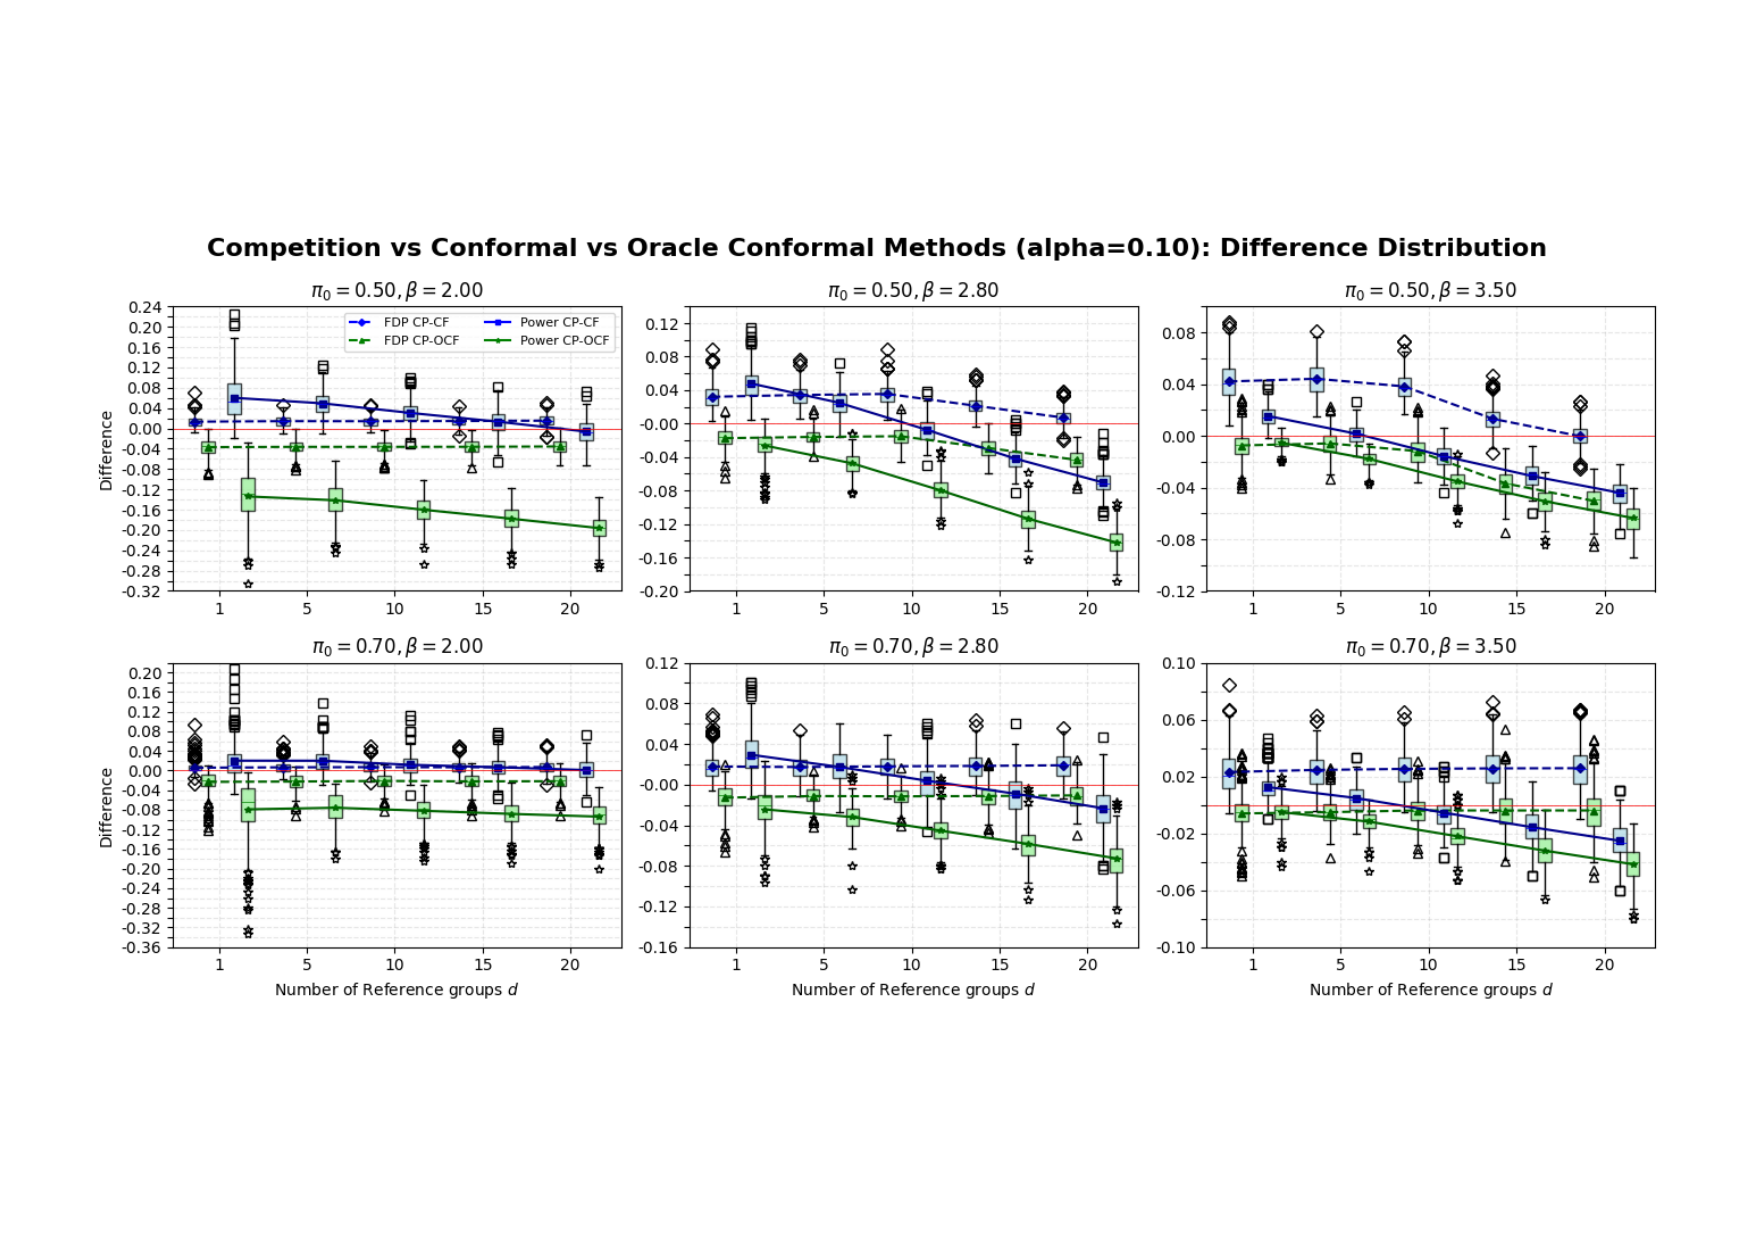}
    \caption{The box plots of the difference of FDR and Power under different reference set size $d$ and parameter setting $\beta,\pi_0$}
    \label{fig:multi_cp_cf_ocf_gap_box}
\end{figure}
It can be observed that as the reference set size increases, the power of the conformal test and that of the oracle conformal test increase relative to the power of the competition test, but the corresponding FDR also becomes larger, although the change in FDR is not so obvious and the FDR itself is always controlled.

\subsection{Integrating More Groups of Hypotheses}

The algorithms and proofs presented in our work can be directly generalized from the integration of two groups to the integration of multiple groups. Here we only provide an example of the integration algorithm for multiple groups of randomized p-values.

\begin{algorithm}[H]
    \caption{Integrated Test of Groups of Randomized p-values}
    \SetAlgoLined
    \DontPrintSemicolon
    \SetAlgoNoEnd
    \LinesNotNumbered
    \SetKwProg{Fn}{Function}{}{}

    \textbf{Input}: $\mathbf{P}^g \in \mathbb{R}_*^{m_g}$, $g=1,2,\cdots,d$, $\alpha \in (0,1)$\\
    \textbf{Output}: $\mathcal{R}_g$, $g=1,2,\cdots,d$

    $K \leftarrow 0,m=\sum_{g=1}^dm_g$ 
    \For{$k=m$ \KwTo $1$}{
      \If{$\sum_{g=1}^{d}\sum_{j=1}^{m_g} \mathbf{1}\{P^g_j \leq q^{m,\alpha}_k\} \geq k$}{
        $K \leftarrow k$; \textbf{break} 
      }
    }
    $\mathcal{R}_g \leftarrow \{j \in [m_g] : P^g_j \leq q^{m,\alpha}_K\}$,$g=1,2,\cdots,d$ \\
    \Return $\mathcal{R}_g$, $g=1,2,\cdots,d$
    \label{salgo:multi_int_cp_cp}
\end{algorithm}
We state without proof that if $\mathbf{P}^g$, $g=1,2,\cdots,d$, are mutually independent randomized p-variables and each satisfies $\mathrm{PRDS}_{\mathcal{H}^g}$, then the FDR is controlled with this algorithm. Replacing $m$ in the algorithm by $m_0 = \sum_{g=1}^d m_0^g$ gives the corresponding oracle algorithm.

We conduct a simulation study to illustrate the performance of our algorithm when integrating multiple groups of hypotheses. For group $g$, we generate random parameters: $m^g \sim \mathrm{Unif}(2000,6000)$, $\pi_0^g \sim \mathrm{Unif}(0.7,0.99)$, $m^g_{cal} = 1000$, $\boldsymbol{w}^g \sim \mathrm{Unif}(0.5,1.5,b)$ with $b=3$, and $\beta^g \sim \mathrm{Unif}(2,3)$. These are used to produce $d$ groups of independent random p-variables, where $m^g$ denotes the size of the testing set, $m^g_{cal}$ denotes the size of the calibration set, $\pi_0^g$ the proportion of true null hypotheses in the testing set, $\boldsymbol{w}^g \in \mathbb{R}_*^b$ the weight vector, and $\beta^g$ the signal strength. At the target FDR level $\alpha = 0.2$, we perform $300$ repeated experiments and compute the average of the FDP and TDP in the experimental results as estimates
of the FDR and Power, respectively, for different numbers of groups $d$.
\begin{figure}[H]
    \centering
    \includegraphics[width=0.9\linewidth]{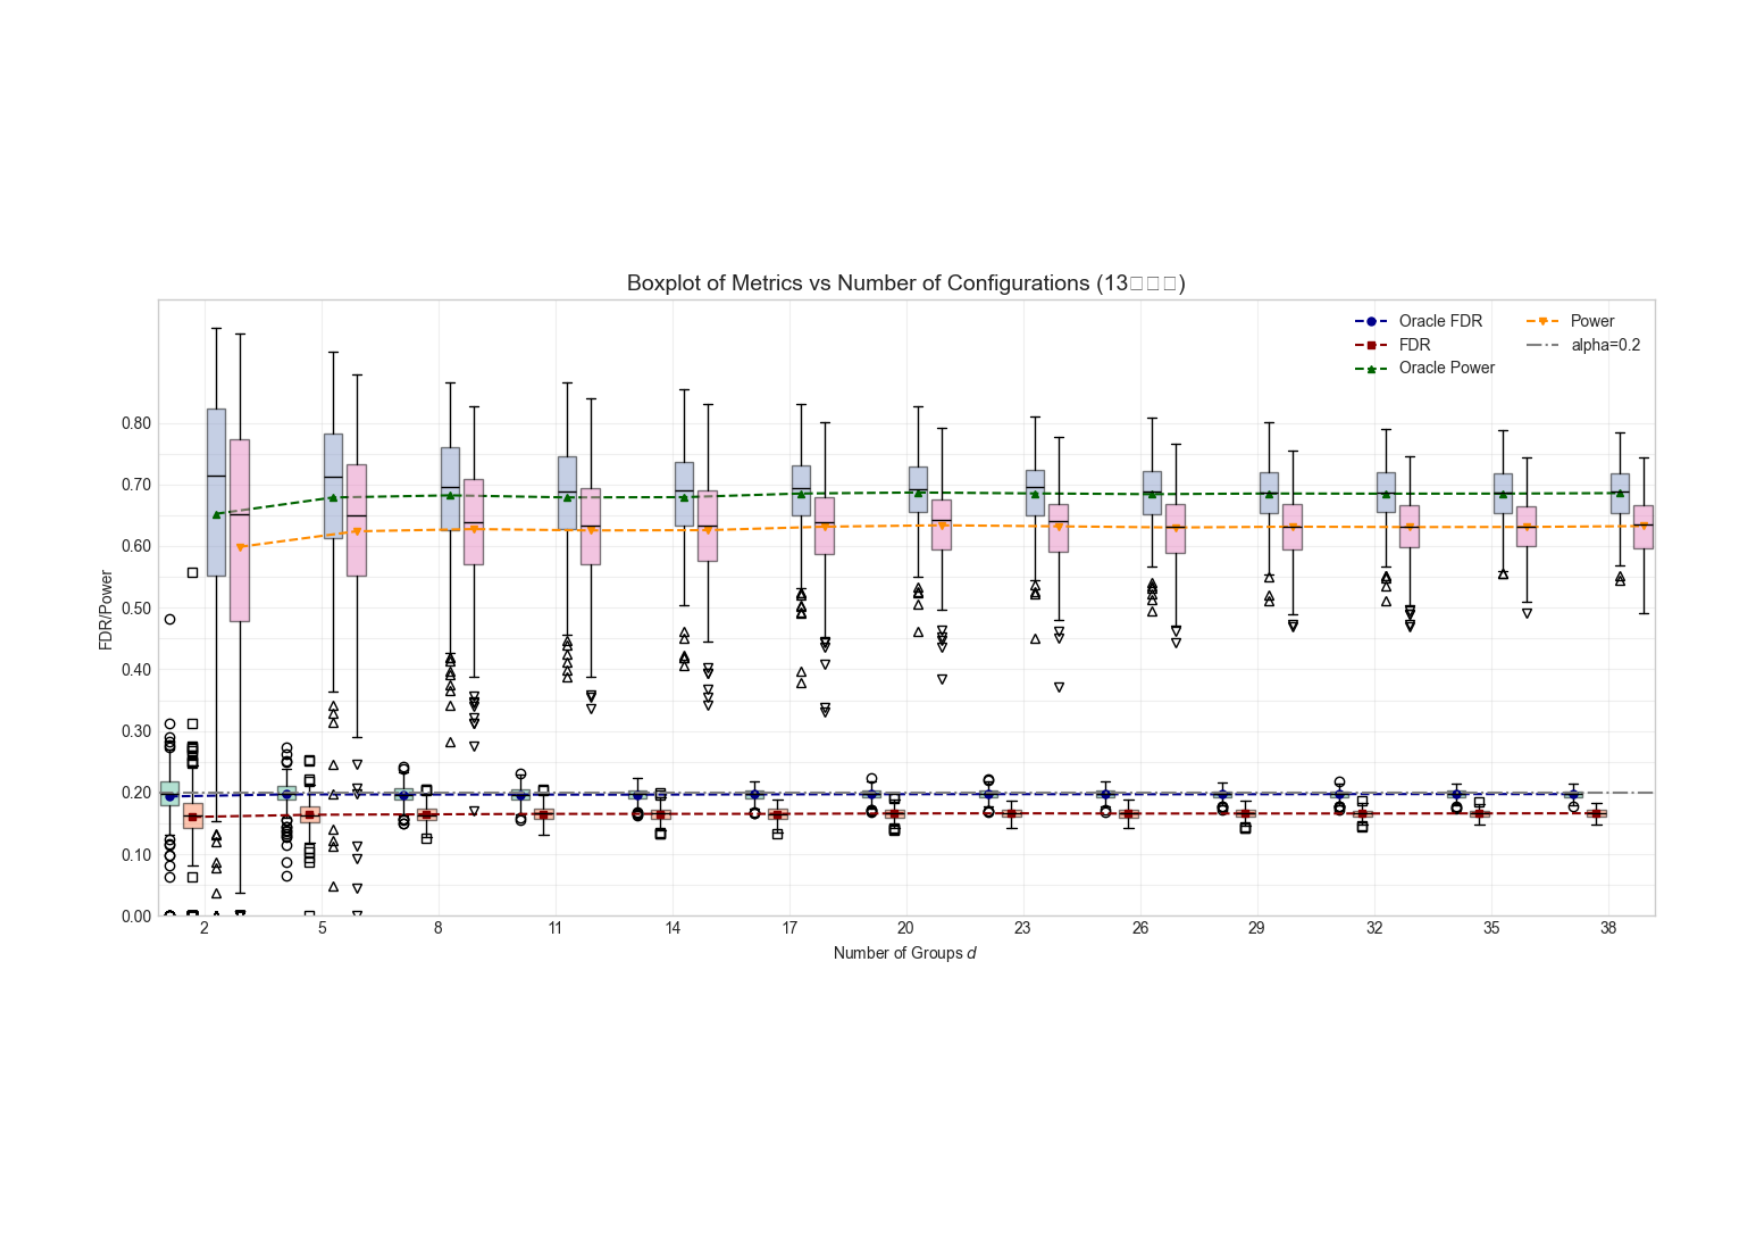}
    \caption{The box plots of FDR and Power under different numbers of groups $d$}
    \label{fig:multi_integration_weights_focus_multi}
\end{figure}
From the simulation results, we observe that our integration algorithm not only preserves FDR control and power, but also improves the stability of the tests to a certain degree.

\subsection{The Influence of Weights in Integration}

When introducing the integration algorithm, we also mentioned that different weights can be assigned to different groups in order to specifically reject more hypotheses from a particular group. Similarly, we only provide an example of the integration algorithm for randomized p-variables.

\begin{algorithm}[H]
    \caption{Weighted Integrated Test of Randomized p-values}
    \SetAlgoLined
    \DontPrintSemicolon
    \SetAlgoNoEnd
    \LinesNotNumbered
    \SetKwProg{Fn}{Function}{}{}

    \textbf{Input}: $\mathbf{P}^1\in \mathbb{R}_*^{m_1}, \mathbf{P}^2\in \mathbb{R}_*^{m_2}$, $\alpha \in (0,1),\rho\in\mathbb{R}_+$\\
    \textbf{Output}: $\mathcal{R}_1,\mathcal{R}_2$

    $K \leftarrow 0$ 
    \For{$k=m_1+m_2$ \KwTo $1$}{
      \If{$\sum_{j=1}^{m_1} \mathbf{1}\{P^1_j \leq q^{m_1+\rho m_2,\alpha}_k\}+\sum_{j=1}^{m_2} \mathbf{1}\{P^2_j/\rho \leq q^{m_1+\rho m_2,\alpha}_k\} \geq k$}{
        $K \leftarrow k$; \textbf{break} 
      }
    }
    $\mathcal{R}_1 \leftarrow \{j \in [m_1] : P^1_j \leq q^{m_1+\rho m_2,\alpha}_K\}$,
    $\mathcal{R}_2 \leftarrow \{j \in [m_2] : P^2_j/\rho \leq q^{m_1+\rho m_2,\alpha}_K\}$ \\
    \Return $\mathcal{R}_1,\mathcal{R}_2$
    \label{salgo:weight_int_cp_cp}
\end{algorithm}
We also construct two independent sets of p-variables. Setting the weight vector $\boldsymbol{w}=1$ is degenerate, meaning that we generate standard p-variables rather than randomized p-variables. We provide the following parameter configurations.
\begin{table}[ht]
    \centering
    \label{tab:data_config}
    \begin{tabular}{ccccc}
    \toprule
    &$m^g$ & $\pi^g_{0}$ & $m^g_{cal}$ & $\beta$ \\
    \midrule
    g=1 & 2000 & 1/2 & 1000 & 2.2 \\
    g=2 & 9000 & 29/30 & 1000 & 2.2 \\
    \bottomrule
    \end{tabular}
    \caption{The parameter setting of weighted integration}
\end{table}
Under the above parameter settings, at the target FDR level $\alpha = 0.2$, we perform $300$ repeated experiments and compute the average of the FDP and TDP in the experimental results as estimates of the FDR and Power, respectively, for different weights $\rho$.
\begin{figure}[H]
    \centering
    \includegraphics[width=0.9\linewidth]{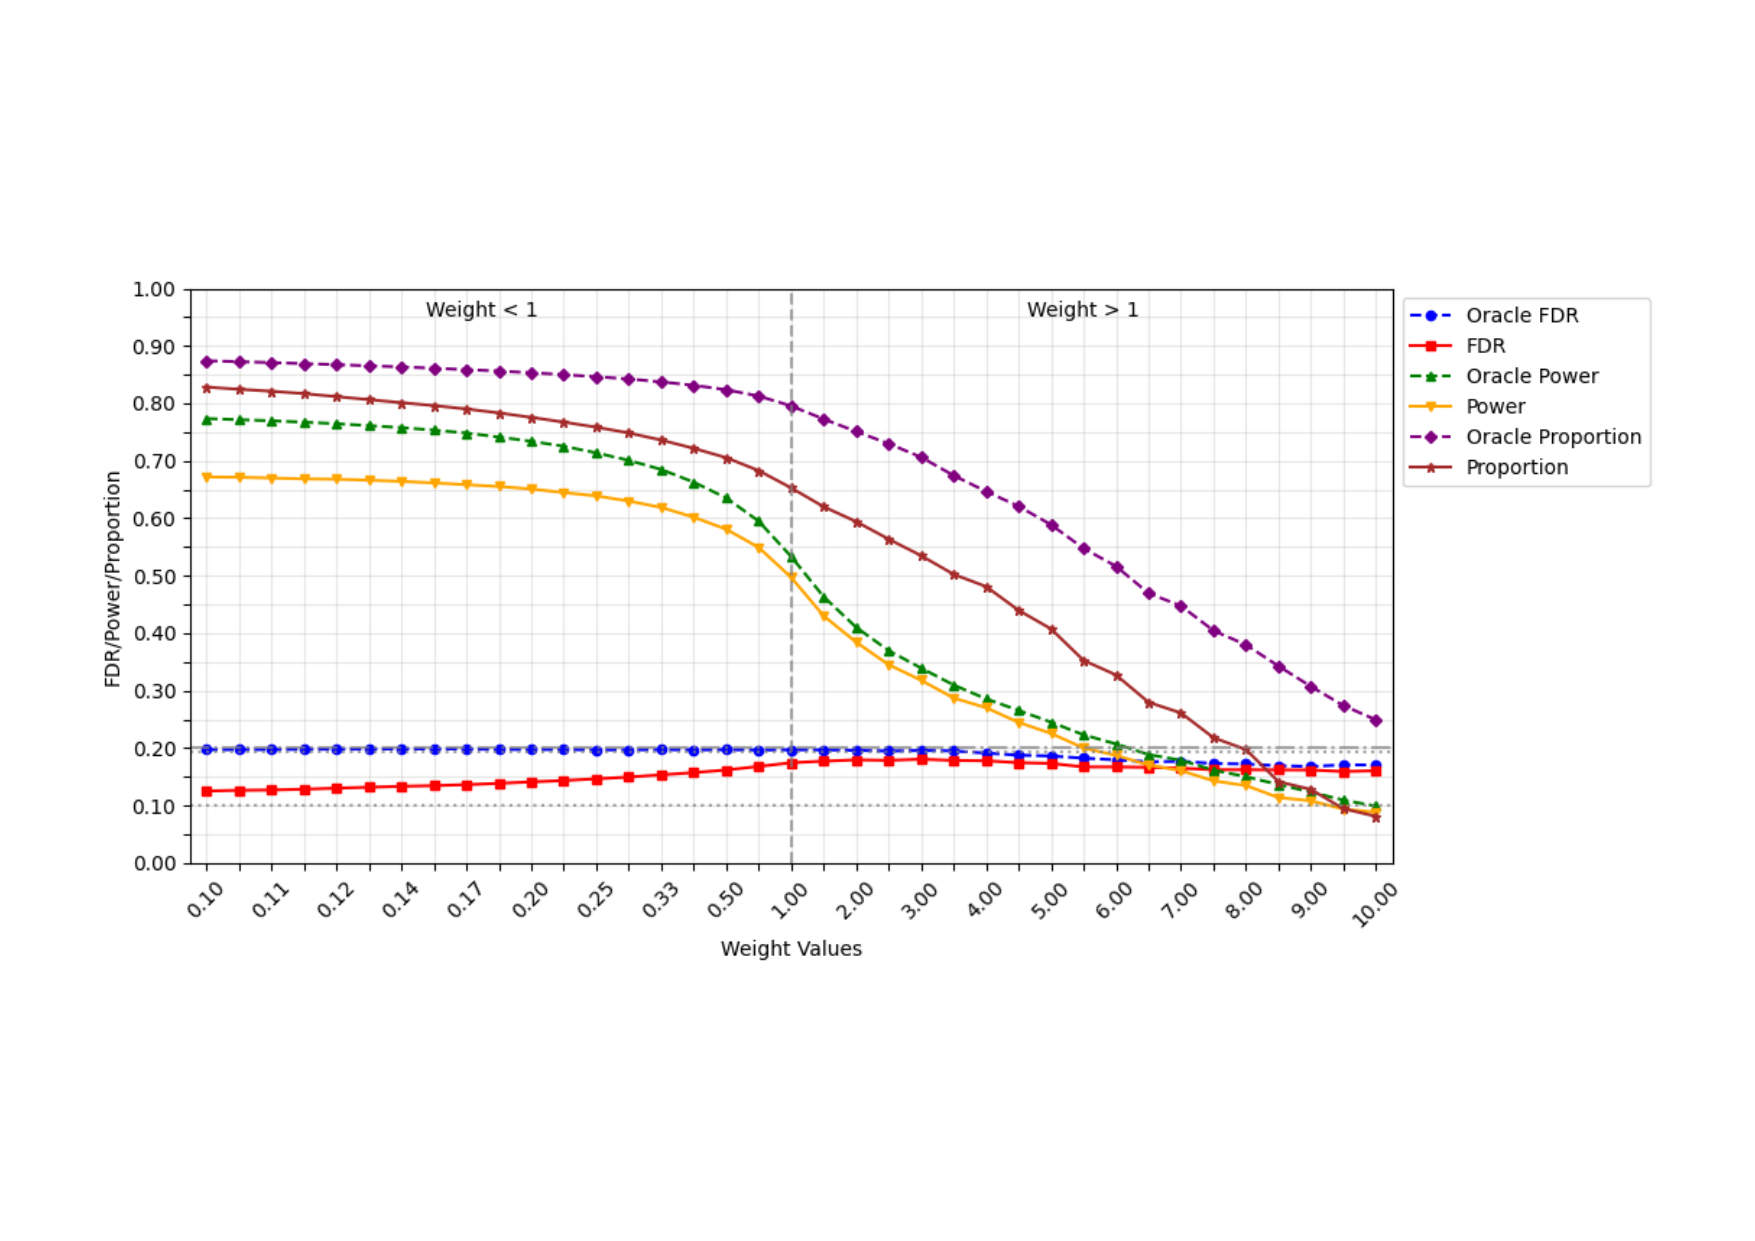}
    \caption{The plots of FDR and Power under different weights $\rho$}
    \label{fig:rp_rp_integration_weights_exps}
\end{figure}

% \bibliography{references}

\end{document}
